# Supplementary material for: Stealing Hyperparameters in Machine Learning
Source: arXiv:1802.05351 source file (2019-09-07)
Supplement: Supplementary file 1 [file appendix-alan.tex]

%\newpage
\appendix

\section{Related Definitions}
\label{app:def}

%\subsection{Definition}
We list definitions that are related to our problems. %as follows. 

%\begin{definition}[Convex Set, Convex Function, and Global Optimality~\cite{boyd2004convex}]
\begin{definition}[Convex Set and Convex Function~\cite{boyd2004convex}]
\label{app:cvx_prop}
A set $\mathbb{C}$ is \emph{\textbf{convex}} if the line segment between any two points in $\mathbb{C}$ lies in $\mathbb{C}$, i.e., $\forall p_1, p_2 \in \mathbb{C}$ and $\forall \theta$ with $0 \leq \theta \leq 1$,
\begin{small}
\begin{align*}
\theta p_1 + (1-\theta) p_2 \in \mathbb{C}.
\end{align*}
\end{small}
\noindent A function $f: \mathbb{R} \rightarrow \mathbb{R}$ is \emph{\textbf{convex}} if the domain of $f$, \textbf{dom} f, is a \emph{convex set}and for all $p, q \in \textbf{dom} f$, and $\forall \theta$ with $0 \leq \theta \leq 1$, %we have
\begin{small} 
\begin{align*}
f(\theta p + (1-\theta) q) \leq \theta f(p) + (1-\theta) f(q).
\end{align*}
\end{small}
%A point $p$ is said to be a global optimum of $f$ if $f(p) \leq f(q)$ for any $q$, and $p$ is local optimum if the inequality holds for any $q$ in some neighborhood of $p$. Obviously, global optimality implies local optimality, while the converse is not true in general. However, for convex functions, global optimality is guaranteed by local optimality.
\end{definition}
\vspace{-5mm}
%\begin{definition}[Smooth Function]
%\end{definition}

\begin{definition}[Subgradient, Subdifferential, and Optimality~\cite{boyd2004convex}]
\label{app:sub_grad}
The \emph{\textbf{subgradient}} of a convex function $f: \mathbb{I} \rightarrow \mathbb{R}$ at a point $p_0$ in the open interval $\mathbb{I}$ is a real number $g$ such that the
\begin{small}
\begin{align*}
f(p)-f(p_0) \geq g (p-p_0), \, \forall p \in \mathbb{I}.
%$f(\mathbf{\theta}-f(\mathbf{\theta}_0) \geq \mathbf{\theta-\theta_0}^C \mathbf{g}$.
\end{align*}
\end{small}
The set of subgradients are defined as the interval $[a, b]$, where $a$ and $b$ are the one-sided limits
\begin{small}
\begin{align*}
a = \lim_{p \to p_0^-} \frac{f(p)-f(p_0)}{p-p_0}, \, 
b = \lim_{p \to p_0^+} \frac{f(p)-f(p_0)}{p-p_0}. 
\end{align*} 
\end{small}
The set $[a, b]$ of all subgradients is called the \emph{\textbf{subdifferential}} of the function $f$ at $p_0$ and is denoted as $\partial f(p)|_{p_0}$. 

For any convex function $f$, a point $p$ is a \textbf{global minimum} of $f$ if and only if the condition $0 \in \partial f(p)$ holds. If $f$ is \textbf{differentiable} at $p$, the set $\partial f(p)$ reduces to the singleton \textbf{gradient} $\{\Delta f(p)\}$, and the condition $0 \in \partial f(p)$ reduces to the gradient-based optimality condition $\Delta f(p) = 0$. 
\end{definition}

%\vspace{-5mm}

\begin{definition}[Kernel Function and Mercer Kernel~\cite{murphy2012machine}] 
\label{app:kernel}
A \textbf{kernel function} $\kappa$ is a real-valued function of two parameters $\mathbf{x}, \mathbf{x}^{\prime} \in \Delta$, where $\Delta$ is some abstract, even infinite dimensional, space, such that $\kappa(\mathbf{x}, \mathbf{x}^{\prime})$ is nonnegative, i.e., $\kappa(\mathbf{x}, \mathbf{x}^{\prime}) \geq 0$, and symmetric, i.e., $\kappa(\mathbf{x}, \mathbf{x}^{\prime}) = \kappa(\mathbf{x}^{\prime}, \mathbf{x})$. Therefore, it can be treated as a measure of similarity. 

\textbf{Mercer kernel (or positive definite kernel)} is the kernel which requires the \textbf{Gram matrix}
\begin{small}
\begin{equation}
\mathbf{K} = 
\begin{bmatrix}
& \kappa(\mathbf{x}_1, \mathbf{x}_1) & \cdots & \kappa(\mathbf{x}_1, \mathbf{x}_n) \\
&  & \vdots & \\
& \kappa(\mathbf{x}_n, \mathbf{x}_1) & \cdots & \kappa(\mathbf{x}_n, \mathbf{x}_n) \\
\end{bmatrix}
\end{equation}
\end{small}
be positive definite for any set of inputs $\{ \mathbf{x}_i \}_{i=1}^n$. In general, if the kernel is Mercer kernel, then there exists a function $\phi$ mapping $\mathbf{x} \in \Delta$ to $\phi(\mathbf{x}) \in \mathbb{R}^M $ such that the kernel function
\begin{small}
\begin{align}
\kappa(\mathbf{x}, \mathbf{x}^\prime) = \langle \phi(\mathbf{x}), \phi(\mathbf{x}^\prime) \rangle,
\end{align}
\end{small}
is represented as an \textbf{inner product} of mapped feature vectors in an implicit feature space defined by $\phi$, which depends on the eigenfunction of $\kappa$. Here, $M$ can be potentially infinite dimension.     
\end{definition}

\vspace{-5mm}
%\section{Details of Convex-induced Regression Models}
\section{Details of Other Regression Algorithms}
\label{app:cvx_reg}

\subsection{LASSO}
\label{app:lasso}

The objective function of LASSO is 
\begin{small}
\begin{align}
\label{lasso}
\mathcal{L}(\mathbf{w}) = \| \mathbf{y}-\mathbf{X}^T \mathbf{w} \|_2^2 + \lambda \| \mathbf{w} \|_1,
\end{align}
\end{small}
where it uses least square loss function and $L_1$ regularization. Note that using $L_1$ regularization can lead to sparse $\mathbf{w}$, that is, many elements of $\mathbf{w}$ would have value 0. 
Generally, $\mathbf{w}$ is efficiently and approximately solved via coordinate descent. 

%Notice that $\| \mathbf{w} \|_1$ is \emph{not differentiable} when $w_i=0$. To handle such a nonsmooth function, we need to extend the notion of gradient to \emph{subgradient}, as defined. 
Notice that $\| \mathbf{w} \|_1$ is \emph{non-differentiable} when $w_i=0$.  To handle such a case, we need to use \emph{subderivative},  defined in Definition~\ref{app:sub_grad}. 
Specifically, its subderivative is 
\begin{small}
\begin{align*}
\partial \| \mathbf{w} \|_1 |_{w_i} = 
\begin{cases}
-1 & \text{if } w_i < 0 \\
[-1, 1] & \text{if } w_i = 0 \\
1  & \text{if } w_i > 0.
\end{cases}
\end{align*}
\end{small}
Then, the subderivative of $\mathcal{L}(\mathbf{w})$ with respect to $w_i$ is
\begin{small}
\begin{align*}
%\label{lasso_grad}
\frac{\partial \mathcal{L}(\mathbf{w})}{\partial w_i} & = 2 (\mathbf{X} \mathbf{X}^T \mathbf{w} - \mathbf{X y})_i+ \lambda \partial \|\mathbf{w}\|_1 |_{w_i} \\
& =  
\begin{cases}
2 (\mathbf{X} \mathbf{X}^T \mathbf{w} - \mathbf{X y})_i - \lambda & \text{if } w_i < 0 \\
\left[ - 2 (\mathbf{X} \mathbf{y})_i - \lambda, - 2 (\mathbf{X} \mathbf{y})_i + \lambda \right] & \text{if } \, w_i = 0 \\
2 (\mathbf{X} \mathbf{X}^T \mathbf{w} - \mathbf{X y})_i + \lambda & \text{if } w_i > 0
\end{cases}
%\frac{\partial \mathcal{L}(\mathbf{w})}{\partial w_i} = 2 \langle \mathbf{x}_i, \mathbf{x}_i \rangle w_i - 2 \left\langle \mathbf{x}_i, \mathbf{r}_i \right\rangle + \lambda \partial \|\mathbf{w}\|_1 |_{w_i},
\end{align*}
\end{small}
% where 
% \begin{align*}
% \partial \| \mathbf{w} \|_1 |_{w_i} = 
% \begin{cases}
% -1 & \text{if } w_i < 0 \\
% [-1, 1] & \text{if } w_i = 0 \\
% 1  & \text{if } w_i > 0.
% \end{cases}
% \end{align*}
%Then, we have the following subgradient 
%\begin{small}
%\begin{align*}
%%\label{lasso_subgrad}
%\frac{\partial \mathcal{L}_{LASSO}}{\partial w_i} =  
%\begin{cases}
%2 \langle \mathbf{x}_i, \mathbf{x}_i \rangle w_i - 2 \left\langle \mathbf{x}_i, \mathbf{r}_i \right\rangle - \lambda & \text{if } w_i < 0 \\
%\left[ - 2 \left\langle \mathbf{x}_i, \mathbf{r}_i \right \rangle - \lambda, - 2 \left\langle \mathbf{x}_i, \mathbf{r}_i \right\rangle + \lambda \right] & \text{if } \, w_i = 0 \\
%2 \langle \mathbf{x}_i, \mathbf{x}_i \rangle w_i - 2 \left\langle \mathbf{x}_i, \mathbf{r}_i \right\rangle + \lambda & \text{if } w_i > 0
%\end{cases}
%\end{align*}
%\end{small}
%By setting it to 0, we can estimate $\lambda$ for each $w_i$ as in Eqn~\ref{lasso_soln}.
We remove $w_i$ with 0 value and the corresponding indexes in $\mathbf{X y}$ and $ \mathbf{X} \mathbf{X}^T \mathbf{y} $ (For simplicity, we still use the same notation).  
Then, by setting the subderivative to be 0, we have $\mathbf{a} = \text{sign}(\mathbf{w})$ and $\mathbf{b} =  2 (\mathbf{X} \mathbf{X}^T \mathbf{w}  - \mathbf{X y}) $.

%By setting it to 0, we can estimate $\lambda$ for each $w_i$ as
%\begin{small}
%\begin{align}
%\label{lasso_soln}
%\hat{\lambda}^{(i)}_{LASSO} =  
%\begin{cases}
%2 \langle \mathbf{x}_i, \mathbf{x}_i \rangle w_i - 2 \left\langle \mathbf{x}_i, \mathbf{r}_i \right\rangle & \text{if }  w_i < 0 \\
%-2 \langle \mathbf{x}_i, \mathbf{x}_i \rangle w_j + 2 \left\langle \mathbf{x}_i, \mathbf{r}_i \right\rangle & \text{if } w_j > 0 
%\end{cases}
%\end{align}
%\end{small}
%Note that if $\lambda \geq \lambda_{\max} = \| \mathbf{X}^\lambda \mathbf{y} \|_{\infty} = \max_i |\langle \mathbf{y}, \mathbf{x}_i \rangle|$, then $\mathbf{w} = \mathbf{0}$. It is because $\mathbf{0}$ is optimal if $(\mathbf{X}^\lambda \mathbf{y})_j \in [-\lambda, \lambda]$, for any $j$. Therefore, $\hat{\lambda}^{(i)}_{LASSO} < \max_i |\langle \mathbf{y}, \mathbf{x}_i \rangle|$.

Note that if $\lambda \geq \lambda_{\max} = \| \mathbf{X} \mathbf{y} \|_{\infty} = \max_j | \mathbf{x}^j \mathbf{y} |$, then $\mathbf{w} = \mathbf{0}$. It is because $\mathbf{0}$ is optimal if $(\mathbf{X} \mathbf{y})_j \in [-\lambda, \lambda]$, for any $j$. Therefore, $\hat{\lambda} < \max_j | \mathbf{x}^j \mathbf{y}|$.

\subsection{Elastic Net (ENet)}
\label{app:enet}

%\myparatight{Elastic Net (ENet)} 
The objective function of ENet is 
\begin{small}
\begin{align}
\label{enet}
\mathcal{L}(\mathbf{w}) = \| \mathbf{y}-\mathbf{X}^T \mathbf{w} \|_2^2 + \lambda_1 \| \mathbf{w} \|_1 + \lambda_2 \| \mathbf{w} \|_2^2.
\end{align}
\end{small}
Here, loss function is least square and regularization term is the $L_2 + L_1$. 
%combination of $L_2$ and $L_1$. 
Similarly with LASSO, $\mathbf{w}$ is efficiently and approximately solved via coordinate descent.  

%Note that $\| \mathbf{w} \|_1$ is \emph{not differentiable} when $w_j=0$. To handle such a case, we need to use \emph{subgradient},  defined in Definition~\ref{app:sub_grad} in Appendix. Then, 
Taking the subderivative of $\mathcal{L}(\mathbf{w})$ with respect to $\mathbf{w}$, we have 
\begin{small}
\begin{align*}
\frac{\partial \mathcal{L}(\mathbf{w})}{\partial \mathbf{w}}  = -2 \mathbf{Xy} + 2 \mathbf{X} \mathbf{X}^T \mathbf{w} + \lambda_1 \partial \|\mathbf{w}\|_1 + 2 \lambda_2 \mathbf{w}. 
\end{align*}
\end{small}

Setting it to be $\mathbf{0}$, we have a system of $m$ equations and 2 unknown variables $\mathbf{\lambda} = \left[ \lambda_1; \lambda_2 \right]$. Such a system is overdetermined and we adopt least square regression to approximate the solution.  
% Taking the subderivative of $\mathcal{L}(\mathbf{w})$ with respect to $w_j$, we have 
% \begin{small}
% \begin{align*}
% \frac{\partial \mathcal{L}(\mathbf{w})}{\partial w_j} = 2 \langle \mathbf{x}_i, \mathbf{x}_i \rangle w_j - 2 \left\langle \mathbf{x}_i, \mathbf{r}_i \right\rangle + \lambda_1 \partial \| \mathbf{w} \|_1 |_{w_j} + \lambda_2 \partial_{w_j} \mathbf{w}^\lambda \mathbf{w},
% \end{align*}
% \end{small}
% where $\mathbf{r}_i = \mathbf{y}-\mathbf{X}_{:,-i} \mathbf{w}_{-i}$ is the residual that all features are used except the $i$-th feature to approximate $\mathbf{y}$. 
% Incorporating into the subdifferential $\partial \| \mathbf{w} \|_1 |_{w_j}$ yields
% \begin{align*}
% \small
% %\label{enet_subgrad}
% \frac{\partial \mathcal{L}_{ENet}}{\partial w_j} =  
% \begin{cases}
% 2 \langle \mathbf{x}_i, \mathbf{x}_i \rangle w_j - 2 \left\langle \mathbf{x}_i, \mathbf{r}_i \right\rangle + 2 \lambda_2 w_j - \lambda_1 & \text{if } w_j < 0 \\
% \left[ - 2 \left\langle \mathbf{x}_i, \mathbf{r}_i \right \rangle + 2 \lambda_2 w_j - \lambda_1, - 2 \left\langle \mathbf{x}_i, \mathbf{r}_i \right\rangle + 2 \lambda_2 w_j + \lambda_1 \right] & \text{if }  w_j = 0 \\
% 2 \langle \mathbf{x}_i, \mathbf{x}_i \rangle w_j - 2 \left\langle \mathbf{x}_i, \mathbf{r}_i \right\rangle + 2 \lambda_2 w_j + \lambda_1 & \text{if } w_j > 0
% \end{cases}
% \end{align*} 
Specifically, 
%we denote $\mathbf{w}^+$ and $\mathbf{w}^-$ as the positive and negative entries of $\mathbf{w}$, and denote $l$-th entry of $\mathbf{w}^+$ and $\mathbf{w}^-$ as $w_l^+$ and $w_l^-$. We arrange $\mathbf{w}$ such that positive values are 
%Furthermore, 
we construct the matrices 
\begin{small} 
\begin{align*}
\mathbf{A} = \left[
\begin{array}{cc}
\text{sign}(w_1) & 2 w_1  \\
\text{sign}(w_2) & 2 w_2  \\
\vdots & \vdots \\
\text{sign}(w_m) & 2 w_m  \\
%\vdots & \vdots \\
\end{array}
\right], \, %\quad
% \bm{\lambda} = \left[ 
% \begin{array}{c}
% \lambda_2 \\
% \lambda_1 \\
% \end{array} 
% \right],
%\quad
\mathbf{c} = \left[ 
\begin{array}{c}
2 \mathbf{x}^1 (\mathbf{y} - \mathbf{X}^T \mathbf{w}) \\
2 \mathbf{x}^2 (\mathbf{y} - \mathbf{X}^T \mathbf{w}) \\
\vdots \\
%-2 \mathbf{x}_1^- (\mathbf{y} - \mathbf{X}^T w_1^-) \\
2 \mathbf{x}^m (\mathbf{y} - \mathbf{X}^T \mathbf{w}) \\
%\vdots
\end{array}
\right]. 
\end{align*}
\end{small}

With above notation, we have the following \emph{normal equation}~\cite{montgomery2015introduction}:
%the system of equations in Eqn~\ref{enet_eqn_1} can be rewritten into the \emph{normal equation}~\cite{montgomery2015introduction}:
\begin{small}
\begin{align}
\label{enet_soln_2}
\mathbf{A}^T \mathbf{A} \bm{\lambda} = \mathbf{A}^T \mathbf{c}.
\end{align}
\end{small}
Hence, $\mathbf{a} = \mathbf{A}$ is a matrix and $\mathbf{b} = \mathbf{c}$.

\section{Details of Other Classification Algorithms}
\label{app:cvx_clf}

% \subsection{$L_2$-regularized LR}
% \label{app:l2blr}

% The gradient of $\mathcal{L}_{L_2-LR}$ with respect to $\mathbf{w}$ is given by
% \begin{align*}
% \small
% %\label{l2lr_grad}
% \begin{split}
% & \frac{\partial \mathcal{L}_{L_2-LR}}{\partial \mathbf{w}} = - \sum_{i=1}^n \left[ y_j \frac{1}{h_\mathbf{w}(\mathbf{x}_j)} \frac{\partial h_\mathbf{w}(\mathbf{x}_j)}{\partial \mathbf{w}} + (1-y_j) \frac{-1}{1-h_\mathbf{w}(\mathbf{x}_j)} \frac{\partial h_\mathbf{w}(\mathbf{x}_j)}{\partial \mathbf{w}}\right] + 2 \lambda \mathbf{w} \\
% & \quad = - \sum_{i=1}^n \left[ y_j \frac{1}{h_\mathbf{w}(\mathbf{x}_j)} h_\mathbf{w}(\mathbf{x}_j) (1-h_\mathbf{w}(\mathbf{x}_j)) + (1-y_j) \frac{1}{1-h_\mathbf{w}(\mathbf{x}_j)} h_\mathbf{w}(\mathbf{x}_j) (1-h_\mathbf{w}(\mathbf{x}_j)) \right] \frac{\partial \mathbf{w}^\lambda \mathbf{x}^j}{\partial \mathbf{w}} + 2 \lambda \mathbf{w} \\
% & \quad = - \sum_{i=1}^n \left(y_j (1-h_\mathbf{w}(\mathbf{x}_j)) - (1-y_j) h_\mathbf{w}(\mathbf{x}_j) \right) \mathbf{x}^j + 2 \lambda \mathbf{w} \\ 
% & \quad = \sum_{i=1}^n (h_\mathbf{w}(\mathbf{x}_j) - y_j) \mathbf{x}^j + 2 \lambda \mathbf{w} \\ 
% & \quad = \mathbf{X}^\lambda (h_\mathbf{w}(\mathbf{X}) - \mathbf{y}) + 2 \lambda \mathbf{w}.
% \end{split}
% \end{align*}

% Setting the derivative to be \textbf{0}, we can then estimate each $w_i$ as in Eqn~\ref{l2lr_soln}.

\subsection{$L_1$-regularized LR (L1-LR)}
\label{app:l1blr}

The objective function of L1-LR is 
\begin{small}
\begin{align}
\label{l1lr}
\mathcal{L}(\mathbf{w}) = \sum_{i=1}^n \text{NLL}(\mathbf{w};\mathbf{x}_i,y_i) + \lambda \| \mathbf{w} \|_1,
%\mathcal{L}_{L1-LR}(\lambda, \mathbf{w}) = - \sum_{i=1}^n \left[ y_j \log h_\mathbf{w}(\mathbf{x}_j) + (1-y_j) \log(1-h_\mathbf{w}(\mathbf{x}_j)) \right] + \lambda \| \mathbf{w} \|_1.
\end{align}
\end{small}
where it uses cross entropy loss function and $L_1$ regularization. Generally, the optimal $\mathbf{w}$ can be approximately solved via LBFGS~\cite{liu1989limited}. 
The subderivative of $\mathcal{L}(\mathbf{w})$ with respect to $\mathbf{w}$ is 
\begin{small}
\begin{align*}
%\label{l1lr_grad}
\frac{\partial \mathcal{L}_{L1-LR}}{\partial \mathbf{w}} = \mathbf{X} (h_\mathbf{w}(\mathbf{X}) - \mathbf{y}) + \lambda \partial_\mathbf{w} \| \mathbf{w} \|_1. 
\end{align*}
\end{small}
Setting it to be \textbf{0} and removing zero $w_i$, we have
$\mathbf{a} = \text{sign}(\mathbf{w}) $ and $\mathbf{b} = \mathbf{X} (h_\mathbf{w}(\mathbf{X}) - \mathbf{y}) $.
\subsection{Support Vector Machine (SVM)}

The objective function of SVM is
\begin{small}
\begin{align}
\label{hl_bsvc}
\mathcal{L}(\mathbf{w}) = \lambda \sum_{j=1}^n L_{HL}(y_j, \langle \mathbf{w}, \mathbf{x}_j \rangle) + \frac{1}{2} \| \mathbf{w} \|_2^2, 
\end{align}
\end{small}
where $L_{HL}(y_j, \langle \mathbf{w}, \mathbf{x}_j \rangle)$ is \textbf{hinge loss} for predicting $\mathbf{x}_j$. 

There are two common hinge loss functions, i.e., regular hinge loss (RHL) and squared hinge loss (SHL). In correspondence, we denote SVM as SVM-RHL and SVM-SHL, respectively. Generally, they are approximately solved via sequential minimal optimization (SMO)~\cite{platt1998sequential} and stochastic gradient descent (SGD)~\cite{bottou2010large} algorithm in their dual form.

%\vspace{-5mm}
\myparatight{RHL} $L_{RHL}(y_j, \langle \mathbf{w}, \mathbf{x}_j \rangle) = \max(0, 1 - y_j \langle \mathbf{w}, \mathbf{x}_j \rangle)$. %Figure~\ref{XX} shows its function as well as squared hinge loss. 
Note that RHL is convex, but non-differential when $y_j \langle \mathbf{w}, \mathbf{x}_j \rangle = 1$. Its subgradient with respect to $\mathbf{w}$ is 
% Once again, it is non-differential because of the \textbf{max} term. However, by introducing slack parameters $\xi_i$, one can show that it is equivalent to solving
% \begin{align}
% \begin{split}
% & \mathcal{L}_{HL-SVM}(\lambda, \mathbf{w}, \bm{\xi}) = \lambda \sum_{i=1}^n \xi_j + \frac{1}{2} \| \mathbf{w} \|^2 \\
% & \text{s.t. } y_j \langle \mathbf{w}, \mathbf{x}_j \rangle \geq 1 - \xi_i, \xi_i \geq 0, \forall i. 
% \end{split}
% \end{align}
%because of the ``max term". Its subgradient with respect to $\mathbf{w}$ is 
\begin{small}
\begin{align*}
%\label{RHL_subg}
\frac{\partial L_{RHL}}{\partial \mathbf{w}} = 
\begin{cases}
-y_j \mathbf{x}_j & \text{if } y_j \langle \mathbf{w}, \mathbf{x}_j \rangle < 1 \\
[-y_j \mathbf{x}_j, \mathbf{0}] & \text{if } y_j \langle \mathbf{w}, \mathbf{x}_j \rangle = 1 \\
\mathbf{0} & \text{if } y_j \langle \mathbf{w}, \mathbf{x}_j \rangle > 1
\end{cases}
\end{align*}
\end{small}
For non-differential point, its subgradient is set to be 0. Therefore, we can estimate $\lambda$ of SVM-RHL using only samples $\mathbf{x}_j$ that satisfy $y_j \langle \mathbf{w}, \mathbf{x}_j \rangle < 1$. 
Then we have $\mathbf{a} = \mathbf{w}$ and $\mathbf{b} = \sum_{j=1}^n -y_j \mathbf{x}_j \mathbf{1}_{y_j \langle \mathbf{w}, \mathbf{x}_j \rangle < 1}$, where $\mathbf{1}_{y_j \langle \mathbf{w}, \mathbf{x}_j \rangle < 1}$ is an indicator function with value 1 if $ y_j \langle \mathbf{w}, \mathbf{x}_j \rangle < 1 $ and 0 otherwise. 

%Setting the derivative of $\mathcal{L}_{SVM}$ with respect to $w_i$ to zero yields
%\begin{small}
%\begin{align}
%\hat{\lambda}^{(i)}_{SVM-RHL} = \frac{w_i}{\sum\limits_{j,y_j \langle \mathbf{w}, \mathbf{x}_j \rangle < 1} y_j {x}_{j,i}}. 
%%\lambda \sum_{j,y_j \langle \mathbf{w}, \mathbf{x}_j \rangle < 1} -y_j \mathbf{x}^j + \mathbf{w} = 0, \quad \text{if } y_j \langle \mathbf{w}, \mathbf{x}_j \rangle < 1.
%%\lambda \sum_{i=1}^n -y_j \mathbf{x}^j + \mathbf{w} = 0, \quad \text{if } y_j \langle \mathbf{w}, \mathbf{x}_j \rangle < 1.
%\end{align} 
%\end{small}

%\vspace{-5mm}
\myparatight{SHL} $L_{SHL}(y_j, \langle \mathbf{w}, \mathbf{x}_j \rangle) = \max(0, 1 - y_j \langle \mathbf{w}, \mathbf{x}_j \rangle)^2$. SHL is convex, smooth, and differential. Its subgradient with respect to $\mathbf{w}$ is given by
\begin{small}
\begin{align*}  
%\label{SHL_subg}
\frac{\partial L_{SHL}}{\partial \mathbf{w}} =
\begin{cases}
-2 y_j \mathbf{x}_j (1 - y_j \langle \mathbf{w}, \mathbf{x}_j \rangle) & \text{if } y_j \langle \mathbf{w}, \mathbf{x}_j \rangle <= 1 \\
\mathbf{0}  & \text{if } y_j \langle \mathbf{w}, \mathbf{x}_j \rangle > 1
\end{cases}
\end{align*}
\end{small}
Therefore, for SVM-SHL, we have $\mathbf{a} = \mathbf{w}$ and $\mathbf{b} = \sum_{j=1}^n -2 y_j \mathbf{x}_j (1 - y_j \langle \mathbf{w}, \mathbf{x}_j \rangle) \mathbf{1}_{y_j \langle \mathbf{w}, \mathbf{x}_j \rangle \leq 1}$.
 
%Therefore, taking the derivative of $\mathcal{L}(\mathbf{w})$ with respect to $w_i$ to zero yields
%\begin{small}
%\begin{align}
%\hat{\lambda}^{(i)}_{SVM-SHL} = \frac{w_i}{\sum\limits_{j,y_j \langle \mathbf{w}, \mathbf{x}_j \rangle \leq 1} 2y_j {x}_{j,i} (1 - y_j \langle \mathbf{w}, \mathbf{x}_j \rangle) }. 
%\end{align}
%\end{small}
For multi-class SVM, it can be derivated from binary SVM in a one-vs-one (or one-vs-rest) fashion~\cite{chang2011libsvm}. In this setting, we can run binary classification Eqn~\ref{hl_bsvc} $K \times (K-1)/2 $ (or $K$) times to estimate the hyperparater.

% \subsection{$L_2$-regularized KLR}
% \label{app:l2bklr}

% Similarly with L2-LR, the derivative of $\mathcal{L}_{L_2-KLR}$ with respect to $\bm{\alpha}$ is given by
% \begin{align}
% \label{l2klr_soln_1}
% \begin{split}
% \frac{\partial \mathcal{L}_{L_2-KLR}}{\partial \bm{\alpha}}
% & = \sum_{i=1}^n (h_{\bm{\alpha}}(\mathbf{k}_j) - y_j) \mathbf{k}_j + 2 \lambda \mathbf{K} \bm{\alpha} \\
% %& = \mathbf{K} (h_{\bm{\alpha}}(\mathbf{K}) - \mathbf{y}) + 2 \lambda \mathbf{K} \bm{\alpha} \\
% & = \mathbf{K} (h_{\bm{\alpha}}(\mathbf{K}) - \mathbf{y} + 2 \lambda \bm{\alpha}),
% \end{split}
% \end{align}
% where we use $\mathbf{K}^\lambda = \mathbf{K}$ and $h_{\bm{\alpha}}(\mathbf{K}) = \left[ h_{\bm{\alpha}}(\mathbf{k}_1), \cdots, h_{\bm{\alpha}}(\mathbf{k}_n) \right]^\lambda $.

% Given $\bm{\alpha}$, we set $\partial_{\bm{\alpha}} \mathcal{L}_{L_2-KLR} = \mathbf{0}$ and consider that $\mathbf{K}$ is full rank, we thus have $h_{\bm{\alpha}}(\mathbf{K}) - \mathbf{y} + 2 \lambda \bm{\alpha} = \mathbf{0}$. Then, for each $\alpha_i$, we then estimate $\lambda$ as in Eqn~\ref{l2klr_soln}.
\subsection{$L_1$-regularized KLR (L1-KLR)}
\label{app:l1bklr}
%The objective function of L1-KLR with primal parameters is 
%\begin{small}
%\begin{align*}
%%\label{l1klr_primal}
%\mathcal{L}_{L1-KLR}(\lambda, \mathbf{w}^\prime) = \sum_{i=1}^n \text{NLL}_{KLR}(\mathbf{w^\prime};\phi(\mathbf{x}_j),y_j) + \lambda \| \mathbf{w}^\prime \|_1.
%%\mathcal{L}_{L2-LR}(\lambda, \mathbf{w}) = - \sum_{i=1}^n \left[ y_j \log h_\mathbf{w}(\mathbf{x}_j) + (1-y_j) \log(1-h_\mathbf{w}(\mathbf{x}_j)) \right] + \lambda \| \mathbf{w} \|_2^2,
%\end{align*}
%\end{small}
%Using $\mathbf{w}^\prime = \Phi(\mathbf{X})^\lambda \bm{\alpha}$, we have its dual form

The objective function of L1-KLR is 
\begin{small}
\begin{align}
\begin{split}
\label{l1klr_dual}
\mathcal{L}(\bm{\alpha}) & = - \sum_{i=1}^n \big( y_j \, \log h_{\bm{\alpha}}(\mathbf{k}_j) + (1 - y_j) \log (1- h_{\bm{\alpha}}(\mathbf{k}_j)) \big) \\
	& + \lambda \| \mathbf{K} \bm{\alpha} \|_1,
\end{split}
\end{align} 
\end{small}
where $\bm{\alpha}$ is approximately solved via LBFGS. 

The subgradient of the second term in Eqn~\ref{l1klr_dual} for $\bm{\alpha}$ is
\begin{small}
\begin{align*}
\begin{split}
\frac{\partial \| \mathbf{K} \bm{\alpha} \|_1 }{\partial \bm{\alpha}} & = \frac{\partial \| \mathbf{K} \bm{\alpha} \|_1 }{\partial \mathbf{K} \bm{\alpha}} \frac{\partial \mathbf{K} \bm{\alpha}}{\partial \bm{\alpha}} = \frac{\bm{\alpha}^T \mathbf{K}^T }{\bm{\alpha}} \textbf{sign}(\mathbf{K} \bm{\alpha}) \\ 
& =  \mathbf{K}^T \textbf{sign}(\mathbf{K} \bm{\alpha}) = \mathbf{K} \textbf{sign}(\mathbf{K} \bm{\alpha}),
\end{split}
\end{align*}
\end{small} 
where $\text{sign}(\mathbf{K} \bm{\alpha}) = \left[ \text{sign}(\mathbf{k}^1\bm{\alpha}); \cdots; \text{sign}(\mathbf{k}^n\bm{\alpha}) \right]$. % is the sign vector of $\mathbf{K} \bm{\alpha}$. 

As $\mathbf{K}$ is invertible, we thus have $\mathbf{a} = \text{sign}(\mathbf{K} \bm{\alpha})$ and $\mathbf{b} = h_{\bm{\alpha}}(\mathbf{K}) - \mathbf{y} $.

\subsection{Kernel SVM (KSVM)}

The objective function of KSVM  is 
%\begin{small}
%\begin{align*}
%%\label{kernel_bsvc_prime}
%\mathcal{L}_{KSVM}(\lambda, \mathbf{w^\prime})  = \lambda \sum_{i=1}^n L_{HL}(y_j, \langle \mathbf{w^\prime}, \phi(\mathbf{x}_j) \rangle) + \frac{1}{2} \| \mathbf{w^\prime} \|_2^2. 
%\end{align*}
%\end{small}
%Using $\mathbf{w}^\prime = \Phi(\mathbf{X})^\lambda \bm{\alpha}$, we have its dual form
\begin{small}
\begin{align}
\label{kernel_bsvc_dual}
\begin{split}
\mathcal{L}(\bm{\alpha}) = \lambda \sum_{i=1}^n L_{HL}(y_j, \langle \bm{\alpha}, \mathbf{k}_j \rangle) + \frac{1}{2} \bm{\alpha}^T \mathbf{K} \bm{\alpha}.
\end{split}
\end{align}
\end{small}
% where $L_{HL}(y_j, \langle \bm{\alpha}, \mathbf{k}_j \rangle) = \max(0, y_j - \langle \bm{\alpha}, \mathbf{k}_j \rangle )$.
Using RHL and SHL, we respectively denote the KSVM as KSVM-RHL and KSVM-SHL. They are approximately solved via SMO and SGD in the dual form.

%vspace{-5mm}
\myparatight{RHL} $L_{RHL}(y_j, \langle \bm{\alpha}, \mathbf{k}_j \rangle) = \max(0, 1 - y_j \langle \bm{\alpha}, \mathbf{k}_j \rangle )$.

Similarly with SVM-RHL, by setting the subderivative of $\mathcal{L}(\bm{\alpha})$ for $\bm{\alpha}$ to be $\mathbf{0}$, 
we have $\mathbf{a} = \mathbf{K} \bm{\alpha}$ and $\mathbf{b} = \sum_{j=1}^n -y_j \mathbf{k}_j \mathbf{1}_{y_j \langle \bm{\alpha}, \mathbf{k}_j \rangle < 1}$. 

%we estimate $\lambda$ for each $\alpha_i$ as 
%\begin{footnotesize}
%\begin{align}
%\label{kernel_bsvc_rhl_soln}
%\hat{\lambda}^{(i)}_{KSVM-RHL} = \frac{\mathbf{k}^i \bm{\alpha}}{\sum\limits_{j, y_j \langle \bm{\alpha}, \mathbf{k}_j \rangle <1} y_j k_{j,i}}.
%\end{align} 
%\end{footnotesize}
%%\vspace{-5mm}
\myparatight{SHL} $L_{SHL}(y_j, \langle \bm{\alpha}, \mathbf{k}_j \rangle) = \max(0, 1 - y_j \langle \bm{\alpha}, \mathbf{k}_j \rangle )^2$. We take the derivative of $\mathcal{L}(\bm{\alpha})$ for $\bm{\alpha}$ and set it to be $\mathbf{0}$. Then, for KSVM-SHL, we have
$\mathbf{a} =\mathbf{K} \bm{\alpha}$ and $\mathbf{b} = \sum_{j=1}^n -2 y_j \mathbf{k}_j (1 - y_j \langle \bm{\alpha}, \mathbf{k}_j \rangle) \mathbf{1}_{y_j \langle \bm{\alpha}, \mathbf{k}_j \rangle \leq 1}$.
 
%\begin{footnotesize} 
%\begin{align}
%\label{kernel_bsvc_shl_soln}
%\hat{\lambda}^{(i)}_{KSVM-SHL} = \frac{\mathbf{k}^i \bm{\alpha}}{\sum\limits_{j,y_j \langle \bm{\alpha}, \mathbf{k}_j \rangle \leq 1} 2y_j {k}_{j,i} (1 - y_j \langle \bm{\alpha}, \mathbf{k}_j \rangle)}. 
%\end{align}
%\end{footnotesize}
For multi-class KSVM, we leverage one-vs-one (or one-vs-rest) fashion of KSVM~\cite{chang2011libsvm}, similar as what SVM does for multi-class SVM. 

%\vspace{-5mm}
\section{**** Theoretical  Analysis***}

We unformally define the sensitive of $\hat{\lambda}$ with respect to $\mathbf{w}$
as $ \frac{\Delta \hat{\lambda}}{\Delta \mathbf{w}}$.  

For RR,
\begin{small}
\begin{align*}
\hat{\lambda}_{RR} = \frac{\mathbf{w}^T (\mathbf{Xy} - \mathbf{X}\mathbf{X}^T \mathbf{w})}{\mathbf{w}^T \mathbf{w}}. 
\end{align*}
\end{small}

The variant of $\hat{\lambda}_{RR}$ with respect to the variant of $\mathbf{w}$ is 
\begin{small}
\begin{align*}
& \Big| \Delta \hat{\lambda}_{RR} \Big| = \Big| \hat{\lambda}_{RR}(\mathbf{w} + \Delta \mathbf{w}) - \hat{\lambda}_{RR}(\mathbf{w}) \Big| \\
& = \Big| \frac{{(\mathbf{w} + \Delta \mathbf{w})}^T (\mathbf{Xy} - \mathbf{X}\mathbf{X}^T (\mathbf{w}+\Delta \mathbf{w}))}{{(\mathbf{w}+\Delta \mathbf{w})}^T (\mathbf{w}+\Delta \mathbf{w})} - \frac{\mathbf{w}^T (\mathbf{Xy} - \mathbf{X}\mathbf{X}^T \mathbf{w})}{\mathbf{w}^T \mathbf{w}} \Big| \\
& = \Big| \frac{\Delta \mathbf{w}^T (\mathbf{Xy} - 2 \mathbf{X} \mathbf{X}^T \mathbf{w}) - \Delta \mathbf{w}^T \mathbf{X} \mathbf{X}^T \Delta \mathbf{w}}{\mathbf{w}^T \mathbf{w}} \Big| \\
& \approx \Big| \frac{\Delta \mathbf{w}^T}{\|\mathbf{w}\|_2^2} \mathbf{X} (\mathbf{y}- 2 \mathbf{X}^T \mathbf{w}) \Big|,
\end{align*}
\end{small}
where in the second and third equations, we use $\mathbf{w} + \Delta \mathbf{w} = \mathbf{w}$ , and $\Delta \mathbf{w}^T \mathbf{X} \mathbf{X}^T \Delta \mathbf{w} = 0$ for sufficient small $\Delta \mathbf{w}$.
Therefore $ \frac{\Delta \hat{\lambda}_{RR}}{\Delta \mathbf{w}} = O(\frac{1}{\|\mathbf{w}\|_2^2})$.

For LASSO,
\begin{small}
\begin{align*}
\hat{\lambda}_{LASSO} = \frac{2 \text{sign}(\mathbf{w})^T (\mathbf{Xy} - \mathbf{X} \mathbf{X}^T \mathbf{w})}{\text{sign}(\mathbf{w})^T \text{sign}(\mathbf{w})}.
\end{align*}
\end{small} 

The variant of $\hat{\lambda}_{LASSO}$ with respect to the variant of $\mathbf{w}$ is 
\begin{small}
\begin{align*}
& \Big| \Delta \hat{\lambda}_{LASSO} \Big| = \Big| \hat{\lambda}_{LASSO}(\mathbf{w} + \Delta \mathbf{w}) - \hat{\lambda}_{LASSO}(\mathbf{w}) \Big| \\
& = \Big| \frac{2 \text{sign}(\mathbf{w} + \Delta \mathbf{w})^T (\mathbf{Xy} - \mathbf{X} \mathbf{X}^T (\mathbf{w} + \Delta \mathbf{w}))}{\text{sign}(\mathbf{w} + \Delta \mathbf{w})^T \text{sign}(\mathbf{w} + \Delta \mathbf{w})} - \frac{2 \text{sign}(\mathbf{w})^T (\mathbf{Xy} - \mathbf{X} \mathbf{X}^T \mathbf{w})}{\text{sign}(\mathbf{w})^T \text{sign}(\mathbf{w})} \Big| \\
& = \Big| \frac{\text{sign}(\mathbf{w})^T \mathbf{X} \mathbf{X}^T \Delta \mathbf{w}}{\|\text{sign}(\mathbf{w})\|_2^2} \Big| \\
& = \Big| \frac{\Delta \mathbf{w}^T}{\|\text{sign}(\mathbf{w})\|_2^2} \mathbf{X} \mathbf{X}^T \text{sign}(\mathbf{w}) \Big|,
\end{align*}
\end{small}
where in the third equation, we use $\text{sign}(\mathbf{w} + \Delta \mathbf{w}) = \text{sign}(\mathbf{w})$.
Therefore $ \frac{\Delta \hat{\lambda}_{LASSO}}{\Delta \mathbf{w}} = O(\frac{1}{\|\text{sign}(\mathbf{w})\|_2^2})$.

For L2-LR,
\begin{small}
\begin{align*}
\hat{\lambda}_{L2-LR} = \frac{\mathbf{w}^T \mathbf{X} (\mathbf{y} - \mathbf{h}_{\mathbf{w}}(\mathbf{X}))}{\mathbf{w}^T \mathbf{w}}. 
\end{align*}
\end{small}

The variant of $\hat{\lambda}_{L2-LR}$ with respect to the variant of $\mathbf{w}$ is 
\begin{small}
\begin{align*}
& \Big| \Delta \hat{\lambda}_{L2-LR} \Big|  = \Big| \hat{\lambda}_{L2-LR}(\mathbf{w} + \Delta \mathbf{w}) - \hat{\lambda}_{L2-LR}(\mathbf{w}) \Big| \\ 
& = \Big| \frac{(\mathbf{w}+ \Delta \mathbf{w})^T (\mathbf{y} - \mathbf{h}_{\mathbf{w}+\Delta \mathbf{w}}(\mathbf{X}))}{(\mathbf{w} + \Delta \mathbf{w})^T (\mathbf{w} + \Delta \mathbf{w})} -  \frac{\mathbf{w}^T \mathbf{X} (\mathbf{y} - \mathbf{h}_{\mathbf{w}}(\mathbf{X}))}{\mathbf{w}^T \mathbf{w}} \Big| \\
& = \Big| \frac{\Delta \mathbf{w}^T \mathbf{X}(\mathbf{y} - \mathbf{h}_{\mathbf{w} + \Delta \mathbf{w}}(\mathbf{X})) - \mathbf{w}^T \mathbf{X} (\mathbf{h}_{\mathbf{w} + \Delta \mathbf{w}}(\mathbf{X}) - \mathbf{h}_{\mathbf{w}}(\mathbf{X}))}{\mathbf{w}^T \mathbf{w}} \Big|  \\
& \approx \Big| \frac{\Delta \mathbf{w}^T}{\|\mathbf{w}\|_2^2} \mathbf{X}(\mathbf{y} - \mathbf{h}_{\mathbf{w}}(\mathbf{X})) \Big|,
\end{align*}
\end{small}
where in the third and equation equation, we use $\mathbf{w} + \Delta \mathbf{w} = \mathbf{w}$ , and $\mathbf{h}_{\mathbf{w} + \Delta \mathbf{w}}(\mathbf{X}) = \mathbf{h}_{\mathbf{w}}(\mathbf{X})$ for sufficient small $\Delta \mathbf{w}$. 
Therefore $ \frac{\Delta \hat{\lambda}_{L2-LR}}{\Delta \mathbf{w}} = O(\frac{1}{\|\mathbf{w}\|_2^2})$.

For L1-LR,
\begin{small}
\begin{align*}
\hat{\lambda}_{L1-LR} = \frac{\text{sign}(\mathbf{w})^T \mathbf{X} (\mathbf{y} - \mathbf{h}_{\mathbf{w}}(\mathbf{X}))}{\text{sign}(\mathbf{w})^T \text{sign}(\mathbf{w})}. 
\end{align*}
\end{small} 

The variant of $\hat{\lambda}_{L1-LR}$ with respect to the variant of $\mathbf{w}$ is
\begin{small}
\begin{align*}
& \Big| \Delta \hat{\lambda}_{L1-LR} \Big|  = \Big| \hat{\lambda}_{L1-LR}(\mathbf{w} + \Delta \mathbf{w}) - \hat{\lambda}_{L1-LR}(\mathbf{w}) \Big| \\ 
& = \Big| \frac{\text{sign}(\mathbf{w} + \Delta \mathbf{w})^T \mathbf{X} (\mathbf{y} - \mathbf{h}_{\mathbf{w} + \Delta \mathbf{w}}(\mathbf{X}))}{\text{sign}(\mathbf{w} + \Delta \mathbf{w})^T \text{sign}(\mathbf{w} + \Delta \mathbf{w})} - \frac{\text{sign}(\mathbf{w})^T \mathbf{X} (\mathbf{y} - \mathbf{h}_{\mathbf{w}}(\mathbf{X}))}{\text{sign}(\mathbf{w})^T \text{sign}(\mathbf{w})} \Big| \\
& = \Big| \frac{\text{sign}(\mathbf{w})^T}{{\| \text{sign}(\mathbf{w})\|_2^2}} \mathbf{X}(\mathbf{h}_{\mathbf{w}+\Delta \mathbf{w}}(\mathbf{X}) - \mathbf{h}_{\mathbf{w}}(\mathbf{X})) \Big|,
\end{align*}
\end{small}
where we use $\text{sign}(\mathbf{w} + \Delta \mathbf{w}) = \text{sign}(\mathbf{w})$.
Therefore $ \frac{\Delta \hat{\lambda}_{L1-LR}}{\Delta \mathbf{w}} = O(\frac{1}{\|\text{sign}(\mathbf{w})\|_2^2})$.

For SVM-RHL,
\begin{small}
\begin{align*}
\frac{1}{\hat{\lambda}_{SVM-RHL}} = \frac{\mathbf{w}^T \Big( \sum_{j=1}^n -y_j \mathbf{x}_j \mathbf{1}_{y_j \langle \mathbf{w}, \mathbf{x}_j \rangle < 1} \Big)}{\mathbf{w}^T \mathbf{w}}. 
\end{align*}
\end{small}

The variant of $\frac{1}{\hat{\lambda}_{SVM-RHL}}$ with respect to the variant of $\mathbf{w}$ is
\begin{small}
\begin{align*}
& \Big| \Delta \hat{\lambda}_{SVM-RHL} \Big| = \Big| \hat{\lambda}_{SVM-RHL}(\mathbf{w} + \Delta \mathbf{w}) - \hat{\lambda}_{SVM-RHL}(\mathbf{w} \Big|\\
& = \Big| \frac{(\mathbf{w} + \Delta \mathbf{w})^T \Big( \sum_{j=1}^n -y_j \mathbf{x}_j \mathbf{1}_{y_j \langle (\mathbf{w} + \Delta \mathbf{w}), \mathbf{x}_j \rangle < 1} \Big)}{(\mathbf{w} + \Delta \mathbf{w})^T (\mathbf{w} + \Delta \mathbf{w})} - \frac{\mathbf{w}^T \Big( \sum_{j=1}^n -y_j \mathbf{x}_j \mathbf{1}_{y_j \langle \mathbf{w}, \mathbf{x}_j \rangle < 1} \Big)}{\mathbf{w}^T \mathbf{w}} \Big| \\
& = \Big| \frac{\Delta \mathbf{w}^T} {\| \mathbf{w}\|_2^2} \Big( \sum_{j=1}^n -y_j \mathbf{x}_j \mathbf{1}_{y_j \langle \mathbf{w}, \mathbf{x}_j \rangle < 1} \Big) \Big|,
\end{align*}
\end{small}
where we assume $\mathbf{w} + \Delta \mathbf{w} = \mathbf{w}$ and $y_j \langle (\mathbf{w} + \Delta \mathbf{w}), \mathbf{x}_j \rangle < 1 $ when $y_j \langle \mathbf{w}, \mathbf{x}_j \rangle < 1$ for sufficient small $\Delta w$.
Therefore $ \frac{\Delta \hat{\lambda}_{SVM-RHL}}{\Delta \mathbf{w}} = O(\frac{1}{\|\mathbf{w}\|_2^2})$.

For SVM-SHL,
\begin{small}
\begin{align*}
\frac{1}{\hat{\lambda}_{SVM-SHL}} = \frac{\mathbf{w}^T \Big( \sum_{j=1}^n - 2y_j \mathbf{x}_j (1- y_j \langle \mathbf{w}, \mathbf{x}_j \rangle) \mathbf{1}_{y_j \langle \mathbf{w}, \mathbf{x}_j \rangle <= 1} \Big)}{\mathbf{w}^T \mathbf{w}}. 
\end{align*}
\end{small}

The variant of $\frac{1}{\hat{\lambda}_{SVM-SHL}}$ with respect to the variant of $\mathbf{w}$ is
\begin{small}
\begin{align*}
& \Big| \Delta \hat{\lambda}_{SVM-SHL} \Big| = \Big| \hat{\lambda}_{SVM-SHL}(\mathbf{w} + \Delta \mathbf{w}) - \hat{\lambda}_{SVM-SHL}(\mathbf{w} \Big|\\
& = \Big| \frac{(\mathbf{w} + \Delta \mathbf{w})^T \Big( \sum_{j=1}^n -2 y_j \mathbf{x}_j (1- y_j \langle \mathbf{w} + \Delta \mathbf{w}, \mathbf{x}_j \rangle) \mathbf{1}_{y_j \langle (\mathbf{w} + \Delta \mathbf{w}), \mathbf{x}_j \rangle < 1} \Big)}{(\mathbf{w} + \Delta \mathbf{w})^T (\mathbf{w} + \Delta \mathbf{w})} \\
&	\qquad - \frac{\mathbf{w}^T \Big( \sum_{j=1}^n - 2 y_j \mathbf{x}_j (1- y_j \langle \mathbf{w}, \mathbf{x}_j \rangle) \mathbf{1}_{y_j \langle \mathbf{w}, \mathbf{x}_j \rangle < 1} \Big)}{\mathbf{w}^T \mathbf{w}} \Big| \\
& = \Big| \frac{\Delta \mathbf{w}^T} {\| \mathbf{w}\|_2^2} \Big( \sum_{j=1}^n -2 y_j (1- y_j \langle \mathbf{w}, \mathbf{x}_j \rangle) \mathbf{x}_j \mathbf{1}_{y_j \langle \mathbf{w}, \mathbf{x}_j \rangle < 1} \Big) \Big|,
\end{align*}
\end{small}
where we use the same assumption as SVM-RHL.
Therefore $ \frac{\Delta \hat{\lambda}_{SVM-SHL}}{\Delta \mathbf{w}} = O(\frac{1}{\|\mathbf{w}\|_2^2})$.

More accurate comparison of SVM-RHL and SVM-SHL, we notice that their difference is between the factor $2\big(1 - y_j \big( \langle \mathbf{w}, \mathbf{x}_j \rangle \big) \big)$ and 1. By leveraging the property of SVM, we know that when the training set $\mathbf{X}$ can be (approximately) linearly separable, then $y_j \langle \mathbf{w}, \mathbf{x}_j \rangle $ is close to 1, i.e., $1-y_j \langle \mathbf{w}, \mathbf{x}_j \rangle $ is a small positive number. 
Therefore, $ 1- y_j \big( \langle \mathbf{w}, \mathbf{x}_j \rangle \big) \big) < \frac{1}{2}$, and thus SVM-SHL is more sensitive than SVM-RHL. 

%\vspace{-5mm}
\section{Hyperparameter Sensitivity Analysis}

\subsection{Proof of Claim~\ref{theorem_reg}}
\label{app:theorem_reg}

For RR, its hyperparameter sensitivity is defined as 

\begin{small}
\begin{align*}
\begin{split}
& \Bigg| \frac{\Delta \hat{\lambda}_{RR}^{(i)}}{\Delta w_i} \Bigg| = \Bigg|\frac{\hat{\lambda}_{RR}^{(i)}(w_i + \Delta w_i) - \hat{\lambda}_{RR}^{(i)}(w_i)}{\Delta w_i}\Bigg| \\
& = \Bigg|\frac{1}{\Delta w_i} \bigg( \frac{\langle \mathbf{x}_i, \mathbf{r}_i \rangle}{w_i + \Delta w_i} - \frac{\langle \mathbf{x}_i, \mathbf{r}_i \rangle}{w_i} \bigg)\Bigg| = \Bigg|\frac{1}{(w_i + \Delta w_i) w_i} \langle \mathbf{x}_i, \mathbf{r}_i \rangle \Bigg|.
\end{split}
\end{align*}
\end{small}
For LASSO, 
\begin{small}
\begin{align*}
\Bigg| \frac{\Delta \hat{\lambda}_{LASSO}^{(i)}}{\Delta w_i} \Bigg| = \Bigg| \frac{-2 \langle \mathbf{x}_i, \mathbf{x}_i \rangle (w_i + \Delta w_i) + 2 \langle \mathbf{x}_i, \mathbf{x}_i \rangle w_i }{\Delta w_i} \Bigg| = \big| 2 \langle \mathbf{x}_i, \mathbf{x}_i \rangle \big|.
\end{align*}
\end{small}
%Similarly, $\frac{\Delta \hat{\lambda}_{LASSO}^{(i)}}{\Delta w_i} = 2 \langle \mathbf{x}_i, \mathbf{x}_i \rangle $ if $w_i < 0$.
Note that the sensitivity of RR depends on both the optimal $w_i$ and the variation $\Delta w_i$; While for LASSO, it is independent of both $w_i$ and $\Delta w_i$. As a result, $\hat{\lambda}_{LASSO}^{(i)}$ of LASSO has a minor (and almost constant) change if the length of $\mathbf{x}_i$ is small (which can be obtained through preprocessing); However, $\hat{\lambda}_{RR}^{(i)}$ of RR can change largely once the absolute value of $w_i$ is much smaller than 1, or/and the absolute value of $\Delta w_i$ is near to $w_i$ (Notice that $\Delta w_i$ and $w_i$ always have the opposite sign in our experiments, and thus if $|\Delta w_i| \rightarrow |w_i|, w_i + \Delta w_i \rightarrow 0$). 
%, which is often the case. For instance, $l_2$ norm of $\mathbf{w}$ is required to be less than or equal 1, i.e., $\| \mathbf{w} \|_2 \leq 1$.  

For ENet, since it incorporates both $L_2$ and $L_1$ regularizations, the sensitivity of $\hat{\lambda}_2^{(i)}$ and $\hat{\lambda}_1^{(i)}$ share the same property with $\hat{\lambda}_{RR}^{(i)}$ and $\hat{\lambda}_{LASSO}^{(i)}$, respectively. % Specifically,

For KRR, the sensitivity is 
\begin{small}
\begin{align*}
%\label{KernelRidge_sensi}
\begin{split}
\Bigg| \frac{\Delta \hat{\lambda}_{KRR}^{(j)}}{\Delta \alpha_j} \Bigg| & = \Bigg| \frac{1}{\Delta \alpha_j} \bigg( \frac{y_j}{\alpha_j + \Delta \alpha_j} - \frac{y_j}{\alpha_j} \bigg) \Bigg| = \Bigg| -\frac{1}{(\alpha_j + \Delta \alpha_j) \alpha_j} y_j \Bigg|,   
\end{split}
\end{align*}
\end{small}
which has a similar form with RR. Thus, the far smaller $\alpha_j$ is than 1, or the much closer $\Delta \alpha_j$ is to $\alpha_j$, the more sensitive KRR is.  

%\vspace{-5mm}
\subsection{Proof of Claim~\ref{theorem_lr}}
\label{app:theorem_lr}

First, we consider L2-LR and L1-LR.

For L2-LR, 
$\hat{\lambda}_{L_2-LR}^{(i)} (w_i + \Delta w_i) = - \frac{\langle \mathbf{x}_i, h_{\mathbf{w}+\Delta w_i}(\mathbf{X}) - \mathbf{y} \rangle}{ 2 (w_i + \Delta w_i)}$, 
where $h_{\mathbf{w}+\Delta w_i}(\mathbf{X}) = \left[ h_{\mathbf{w}+\Delta w_i}(\mathbf{x}_1), \cdots, h_{\mathbf{w}+\Delta w_i}(\mathbf{x}_n) \right]^\lambda $ and $h_{\mathbf{w}+\Delta w_i} (\mathbf{x}_i) = \frac{1}{1 + \exp(\sum_{j \neq i} w_j x_{i,j}) + (w_i + \Delta w_i) x_{i,i}}$ (One should notice that the notation $\mathbf{w}+\Delta w_i$ here is not so ``formal", as $\Delta w_i$ is not added to all elements of $\mathbf{w}$, but to its $i$-th entry. We use such notation for simplicity).
Therefore, 
\begin{small}
\begin{align*}
%\label{L2_LR_sensi}
\begin{split}
& \Bigg| \frac{\Delta \hat{\lambda}_{L_2-LR}^{(i)}}{\Delta w_i} \Bigg| = \Bigg| \frac{\hat{\lambda}_{L_2-LR}^{(i)} (w_i + \Delta w_i) - \hat{\lambda}_{L_2-LR}^{(i)} (w_i)}{\Delta w_i} \Bigg| \\
& = \Bigg| \frac{\langle \mathbf{x}_i, h_{\mathbf{w}+\Delta w_i}(\mathbf{X}) - \mathbf{y} \rangle}{\Delta w_i} \bigg( -\frac{1}{2(w_i + \Delta w_i)}  + \frac{\langle \mathbf{x}_i, h_{\mathbf{w}}(\mathbf{X}) - \mathbf{y} \rangle}{2 w_i}  \bigg) \Bigg| \\
& = \Bigg| \frac{\langle \mathbf{x}_i, h_{\mathbf{w}+\Delta w_i}(\mathbf{X}) - \mathbf{y} \rangle}{\Delta w_i} \bigg( - \frac{1}{2(w_i + \Delta w_i)}  + \frac{\langle \mathbf{x}_i, h_{\mathbf{w}}(\mathbf{X}) - \mathbf{y} \rangle}{2(w_i + \Delta w_i)}  \bigg) \\ 
& \quad + \frac{1}{\Delta w_i} \bigg( - \frac{\langle \mathbf{x}_i, h_{\mathbf{w}}(\mathbf{X}) - y \rangle}{2(w_i + \Delta w_i)}  + \frac{\langle \mathbf{x}_i, h_{\mathbf{w}}(\mathbf{X}) - \mathbf{y} \rangle}{2 w_i}  \bigg) \Bigg| \\
& = \Bigg| - \frac{\langle \mathbf{x}_i, h_{\mathbf{w}+\Delta w_i}(\mathbf{X}) - h_{\mathbf{w}}(\mathbf{X}) \rangle}{2(w_i + \Delta w_i) \Delta w_i} + \frac{\langle \mathbf{x}_i, h_{\mathbf{w}}(\mathbf{X}) - \mathbf{y} \rangle}{2 w_i (w_i + \Delta w_i)}  \Bigg|. 
\end{split}
\end{align*}
\end{small}

For L1-LR, 
\begin{small}
\begin{align*}
%\label{L1_LR_sensi}
\begin{split}
\Bigg| \frac{\Delta \hat{\lambda}_{L_1-LR}^{(i)}}{\Delta w_i} \Bigg| & = \Bigg| \frac{1}{\Delta w_i} \big( \langle \mathbf{x}_i, h_{\mathbf{w} + \Delta w_i}(\mathbf{X}) - \mathbf{y} \rangle - \langle \mathbf{x}_i, h_{\mathbf{w}}(\mathbf{X}) - \mathbf{y} \rangle \big) \Bigg| \\
& = \Bigg| \frac{1}{\Delta w_i} \langle \mathbf{x}_i, h_{\mathbf{w} + \Delta w_i}(\mathbf{X}) - h_{\mathbf{w}}(\mathbf{X}) \rangle \Bigg|.
\end{split}
\end{align*}
\end{small}
%Similarly, if $w_i <0$, $\frac{\Delta \hat{\lambda}_{L_1-LR}^{(i)}}{\Delta w_i} = - \frac{1}{\Delta w_i} \langle \mathbf{x}_i, h_{\mathbf{w} + \Delta w_i}(\mathbf{X}) - h_{\mathbf{w}}(\mathbf{X}) \rangle $.
%Comparing Eqn~\ref{L2_LR_sensi} with Eqn~\ref{L1_LR_sensi} 
Comparing above two equations and reusing aforementioned analysis, we observe that once $|w_i|$ is much smaller than 1 or $\Delta w_i$ is comparable with $w_i$, then L2-LR is more sensitive than L1-LR. %in terms of the variation of $w_i$. 

Then, we consider L2-KLR and L1-KLR.

For L2-KLR,
\begin{small}
\begin{align*}
\begin{split}
& \Bigg| \frac{\Delta \hat{\lambda}_{L_2-KLR}^{(j)}}{\Delta \alpha_j} \Bigg| = \Bigg| \frac{1}{\Delta \alpha_j} \bigg( \frac{y_j - h_{\bm{\alpha} + \Delta \alpha_j}(\mathbf{k}_j)}{2(\alpha_j + \Delta \alpha_j)} - \frac{y_j - h_{\bm{\alpha}} (\mathbf{k}_j)}{2 \alpha_j} \bigg) \Bigg| \\
& = \Bigg| - \frac{h_{\bm{\alpha}+\Delta \alpha_j}(\mathbf{k}_j) - h_{\bm{\alpha}}(\mathbf{k}_j)}{2(\alpha_j + \Delta \alpha_j) \Delta \alpha_j} + \frac{h_{\bm{\alpha}}(\mathbf{k}_j) - y_j}{2(\alpha_j + \Delta \alpha_j) \alpha_j} \Bigg|,
\end{split}
\end{align*}
\end{small}
where $h_{\bm{\alpha}+\Delta \alpha_j} (\mathbf{k}_j) = \frac{1}{1+ \exp(\langle \bm{\alpha}, \mathbf{k}_j \rangle + \Delta \alpha_j k_{j,j})}$.

For L1-KLR, %if $\mathbf{k}^j \bm{\alpha} < 0$,
\begin{small}
\begin{align*}
\Bigg| \frac{\Delta \hat{\lambda}_{L_1-KLR}^{(j)}}{\Delta \alpha_j} \Bigg| = \Bigg| \frac{1}{\Delta \alpha_j} \big( h_{\bm{\alpha}+\Delta \alpha_j}(\mathbf{k}_j) - h_{\bm{\alpha}}(\mathbf{k}_j) \big) \Bigg|.
\end{align*}
\end{small}
%and $\frac{\Delta \hat{\lambda}_{L_1-KLR}^{(j)}}{\Delta \alpha_j} = \frac{1}{\Delta \alpha_j} \big( - h_{\bm{\alpha}+\Delta \alpha_j}(\mathbf{k}_j) + h_{\bm{\alpha}}(\mathbf{k}_j) \big)$ if $\mathbf{k}^j \bm{\alpha} > 0$. 

We have similar sensitivity analysis of L2-KLR and L1-KLR as that of L2-LR and L1-LR. That is, if $|\alpha_j|$ is much smaller than 1 or $\Delta \alpha_j$ is comprable with $\alpha_j$, then L2-KLR is more sensitive than L1-KLR.

%\vspace{-5mm}
\subsection{Proof of Claim~\ref{theorem_svc}}
\label{app:theorem_svc}

First, we consider SVM-RHL and SVM-SHL.

For SVM-RHL,
\begin{footnotesize} 
\begin{align*}
%\label{SVM_RHL_sensi}
\begin{split}
\Bigg| \frac{\Delta \hat{C}_{SVM-RHL}^{(i)}}{\Delta w_i} \Bigg| & = \Bigg| \frac{1}{\Delta w_i} \Bigg( \frac{w_i + \Delta w_i}{\sum\limits_{j, y_j \big( \langle \mathbf{w}, \mathbf{x}_j \rangle + \Delta w_i x_{j,i} \big) < 1} y_j x_{j,i}} - \frac{w_i}{\sum\limits_{j, y_j \langle \mathbf{w}, \mathbf{x}_j \rangle <1} y_j x_{j,i} } \Bigg) \Bigg| \\
& \approx \frac{1}{\sum\limits_{j, y_j \big( \langle \mathbf{w}, \mathbf{x}_j \rangle + \Delta w_i x_{j,i} \big) < 1} y_j x_{j,i}}, 
\end{split}
\end{align*}
\end{footnotesize}
where we assume that by adding $\Delta w_i$, the sign of $1- y_j \big( \langle \mathbf{w}, \mathbf{x}_j \rangle + \Delta w_i x_{i,i} \big) \big)$ is still positive (It often satisfies in practice). 

For SVM-SHL, 
\begin{footnotesize}
\begin{align*}
%\label{SVM_SHL_sensi}
\begin{split}
& \Bigg| \frac{\Delta \hat{C}_{SVM-SHL}^{(i)}}{\Delta w_i} \Bigg| = \\
&  \Bigg| \frac{1}{\Delta w_i} \Bigg( \frac{w_i + \Delta w_i}{\sum\limits_{j, y_j \big( \langle \mathbf{w}, \mathbf{x}_j \rangle + \Delta w_i x_{j,i} \big) < 1} 2 y_j x_{j,i} \big(1 - y_j \big( \langle \mathbf{w}, \mathbf{x}_j \rangle + \Delta w_i x_{j,i} \big) \big) } \\
& \quad - \frac{w_i}{\sum\limits_{j, y_j \langle \mathbf{w}, \mathbf{x}_j \rangle <1} 2 y_j x_{j,i} \big(1 - y_j \langle \mathbf{w}, \mathbf{x}_j \rangle \big) } \Bigg) \Bigg| \\
& \approx \frac{1}{\sum\limits_{j, y_j \big( \langle \mathbf{w}, \mathbf{x}_j \rangle + \Delta w_i x_{j,i} \big) < 1} 2 y_j x_{j,i} \big(1 - y_j \big( \langle \mathbf{w}, \mathbf{x}_j \rangle + \Delta w_i x_{j,i} \big) \big) }.
\end{split}
\end{align*}
\end{footnotesize}
%Comparing Eqn~\ref{SVM_RHL_sensi} and Eqn~\ref{SVM_SHL_sensi}, 
Comparing above two equations, we notice that their difference is between the factor $2\big(1 - y_j \big( \langle \mathbf{w}, \mathbf{x}_j \rangle + \Delta w_i x_{i,i} \big) \big)$ and 1. By leveraging the property of SVM, we know that when the training set $\mathbf{X}$ can be (approximately) linearly separable, then $y_j \langle \mathbf{w}, \mathbf{x}_j \rangle $ is close to 1, i.e., $1-y_j \langle \mathbf{w}, \mathbf{x}_j \rangle $ is a small positive number. 
Therefore, 
%by adding $\Delta w_i$ such that the sign of $1- y_j \big( \langle \mathbf{w}, \mathbf{x}_j \rangle + \Delta w_i x_{i,i} \big) \big)$ is still positive, 
we conclude that $ 1- y_j \big( \langle \mathbf{w}, \mathbf{x}_j \rangle + \Delta w_i x_{i,i} \big) \big) < \frac{1}{2}$, and thus $\hat{C}_{SVM-SHL}^{(i)}$ is more sensitive than $\hat{C}_{SVM-RHL}^{(i)}$.

Then, we consider KSVM-RHL and KSVM-SHL.

For KSVM-RHL,
\begin{footnotesize} 
\begin{align*}
%\label{KSVM_RHL_sensi}
\Bigg| \frac{\Delta \hat{C}_{KSVM-RHL}^{(i)}}{\Delta \alpha_i} \Bigg|  = \Bigg| \frac{1}{\Delta \alpha_i} \Bigg( \frac{\mathbf{k}^i \bm{\alpha} + k_{ii} \Delta \alpha_i}{\sum\limits_{j, y_j (\langle \bm{\alpha}, \mathbf{k}_j \rangle + \Delta \alpha_i k_{i,j}) <1} y_j k_{j,i}} - \frac{\mathbf{k}^i \bm{\alpha}}{\sum\limits_{j, y_j \langle \bm{\alpha}, \mathbf{k}_j \rangle <1} y_j k_{j,i} } \Bigg) \Bigg|.
\end{align*}
\end{footnotesize}

For KSVM-SHL
\begin{small}
\begin{align*}
%\label{KSVM_SHL_sensi}
\begin{split}
& \Bigg| \frac{\Delta \hat{C}_{KSVM-SHL}^{(i)}}{\Delta \alpha_i} \Bigg| = \\
& \Bigg| \frac{1}{\Delta \alpha_i} \Bigg( \frac{\mathbf{k}^i \bm{\alpha} + k_{ii} \Delta \alpha_i}{\sum\limits_{j, y_j (\langle \bm{\alpha}, \mathbf{k}_j \rangle + \Delta \alpha_i k_{i,j}) <1} 2 y_j k_{j,i} \big( 1 - y_j (\langle \bm{\alpha}, \mathbf{k}_j \rangle + \Delta \alpha_i k_{i,j}) \big)} \\
& \quad -  \frac{\mathbf{k}^i \bm{\alpha}}{\sum\limits_{j, y_j \langle \bm{\alpha}, \mathbf{k}_j \rangle <1} 2 y_j k_{j,i} \big( 1 - y_j \langle \bm{\alpha}, \mathbf{k}_j \rangle \big)} \Bigg) \Bigg|.
\end{split}
\end{align*}
\end{small}

Similar results can be obtained, i.e., $\hat{C}_{KSVM-SHL}^{(i)}$ is more sensitive than $\hat{C}_{KSVM-RHL}^{(i)}$,  as $1 - y_j (\langle \bm{\alpha}, \mathbf{k}_j \rangle + \Delta \alpha_i k_{i,j}) < \frac{1}{2}$ is often satisfied. 

\begin{figure}[htbp]
\center
\subfigure[M1 vs. M3]{\includegraphics[width=0.23\textwidth]{./src_time/figs/result-CovType-lr-acc-time-m1-m3.pdf}\label{lr_covtype_m1_m3}} 
\subfigure[M2 vs. M3]{\includegraphics[width=0.23\textwidth]{./src_time/figs/result-CovType-lr-acc-time-m2-m3.pdf}\label{lr_covtype_m2_m3}}
\caption{Relative ACC error and speedup of L2-LR on CovType.}
\label{lr_covtype}
\end{figure}

\begin{figure}[htbp]
\center
\subfigure[M1 vs. M3]{\includegraphics[width=0.23\textwidth]{./src_time/figs/result-CovType-svc-acc-time-m1-m3.pdf}\label{svc_covtype_m1_m3}} 
\subfigure[M2 vs. M3]{\includegraphics[width=0.23\textwidth]{./src_time/figs/result-CovType-svc-acc-time-m2-m3.pdf}\label{svc_covtype_m2_m3}}
\caption{Relative ACC error and speedup of SVM-SHL on CovType.}
\label{svc_covtype}
\end{figure}

\begin{figure}[htbp]
\center
\subfigure[L2-LR]{\includegraphics[width=0.23\textwidth]{./src_time/figs/result-Gaussian-speedup-lr-0.001-error.pdf}\label{lr_speedup}} 
\subfigure[SVM-SHL]{\includegraphics[width=0.23\textwidth]{./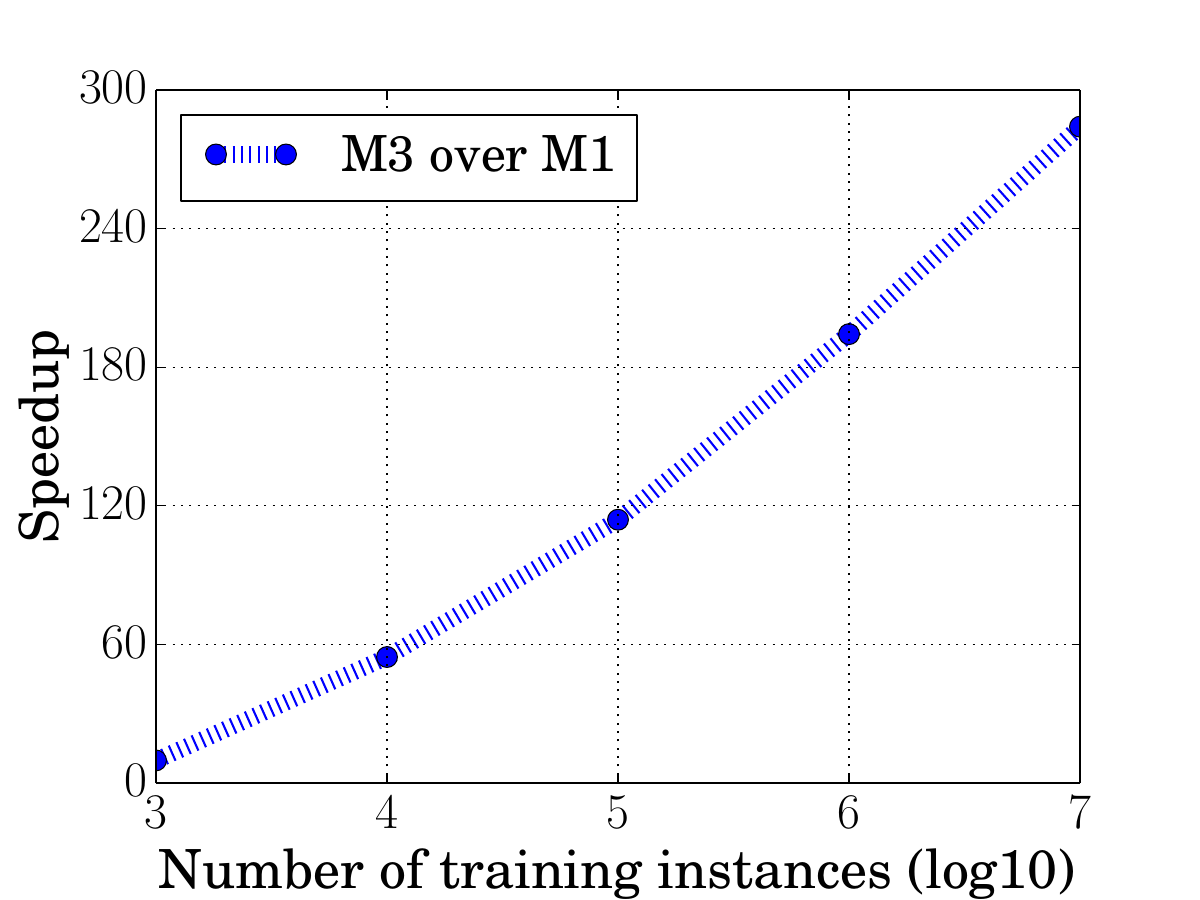}\label{svc_speedup}}
\caption{Speedup of L2-LR and SVM-SHL on synthetic data drawn from Gaussian distribution with Poission noise.}
\label{speedup_gaussian}
\end{figure}

\begin{figure}[htbp]
\center
\subfigure[L2-LR]{\includegraphics[width=0.23\textwidth]{./src_time/figs/result-CovType-lr-defense-m1-m3.pdf}\label{lr_defense_covtype_m1_m3}} 
\subfigure[SVM-SHL]{\includegraphics[width=0.23\textwidth]{./src_time/figs/result-CovType-svc-defense-m1-m3.pdf}\label{svc_defense_covtype_m1_m3}}
\caption{Relative ACC error of L2-LR and SVM-SHL under defense on CovType.}
\label{real_defense_clf_covType}
\end{figure}

\section{Other Attack Results}
\label{app:attack_res}

We show the hyperparameter stealing results of classification models on Ionosphere and Iris in Figure~\ref{clf_res_attack_other} and evaluate real-world scenario on CovType in Figures~\ref{lr_covtype} and~\ref{svc_covtype}. In Figure~\ref{speedup_gaussian}, we also show the speedup of \textbf{M3} with less than 0.1\% $\Delta$-ACC error on synthetic data, which are drawn from Gaussian distribution with Poission noise. We observe that as the number of training set increases, the speedup also enhances.  
% \begin{figure}
% \center
% \subfigure[Iris]{\includegraphics[width=0.23\textwidth]{./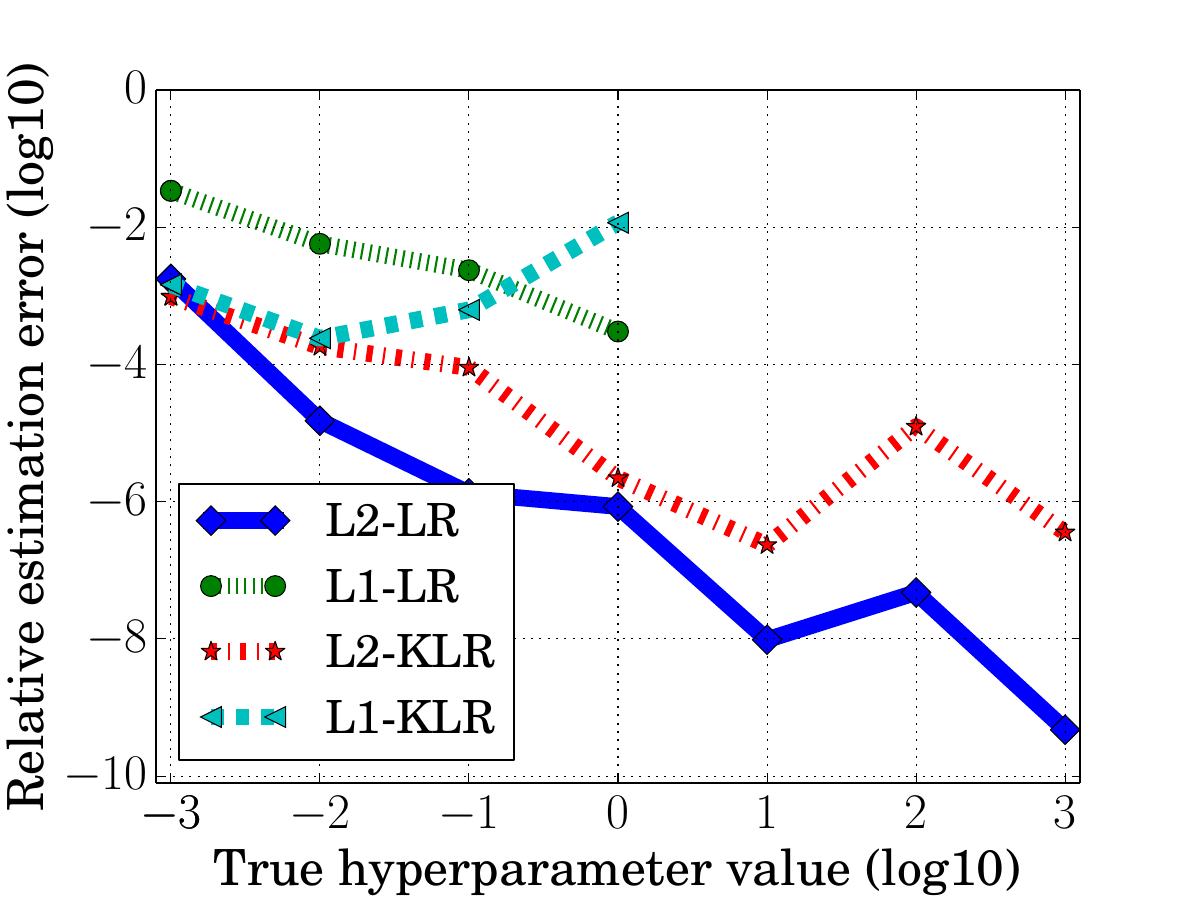}\label{clf_lr_iris}} 
% \subfigure[Ionosphere]{\includegraphics[width=0.23\textwidth]{./src_attack/figs/clf/result-clf-lr-ionosphere-new-final.pdf}\label{clf_lr_ionosphere}}
% %\subfigure[Madelon]{\includegraphics[width=0.32\textwidth]{./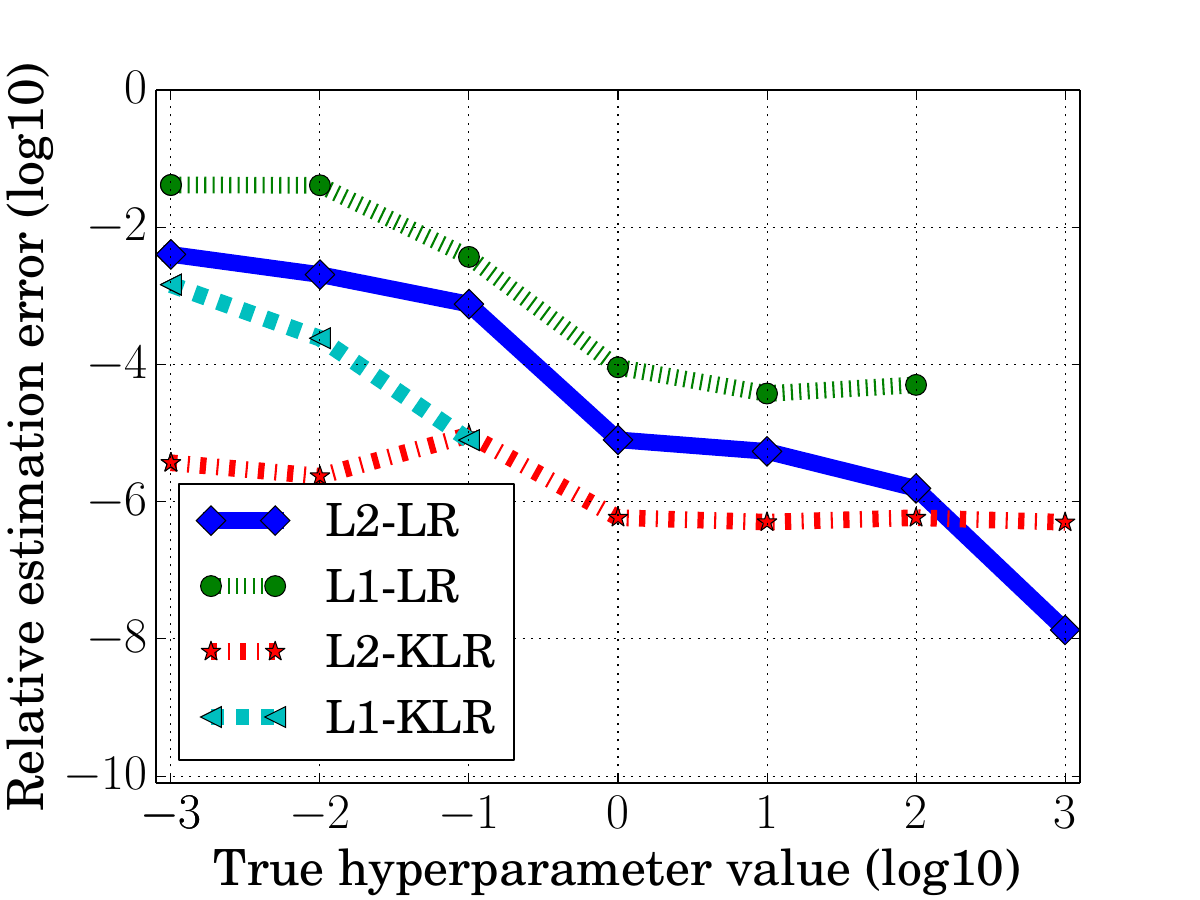}\label{clf_lr_madelon}} 
% \caption{Hyperparameter stealing results of binary LR-based classification models.}
% \label{clf_blr_res_attack}
% \end{figure}

% \begin{figure}
% \center
% \label{clf_blsvc_res_attack}
% \subfigure[Iris]{\includegraphics[width=0.23\textwidth]{./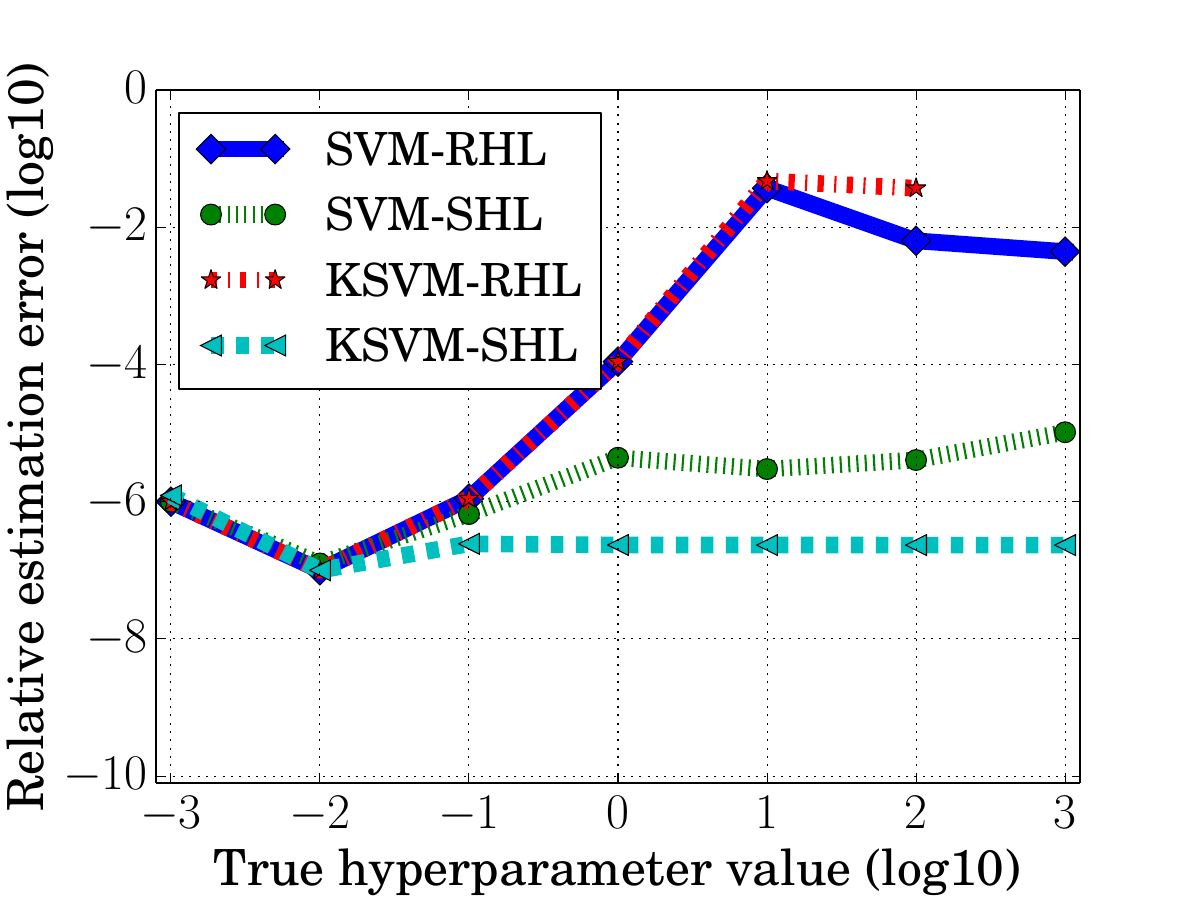}\label{clf_svc_iris}} 
% \subfigure[Ionosphere]{\includegraphics[width=0.23\textwidth]{./src_attack/figs/clf/result-clf-svc-ionosphere-new-final.pdf}\label{clf_svc_ionosphere}}
% %\subfigure[Madelon]{\includegraphics[width=0.32\textwidth]{./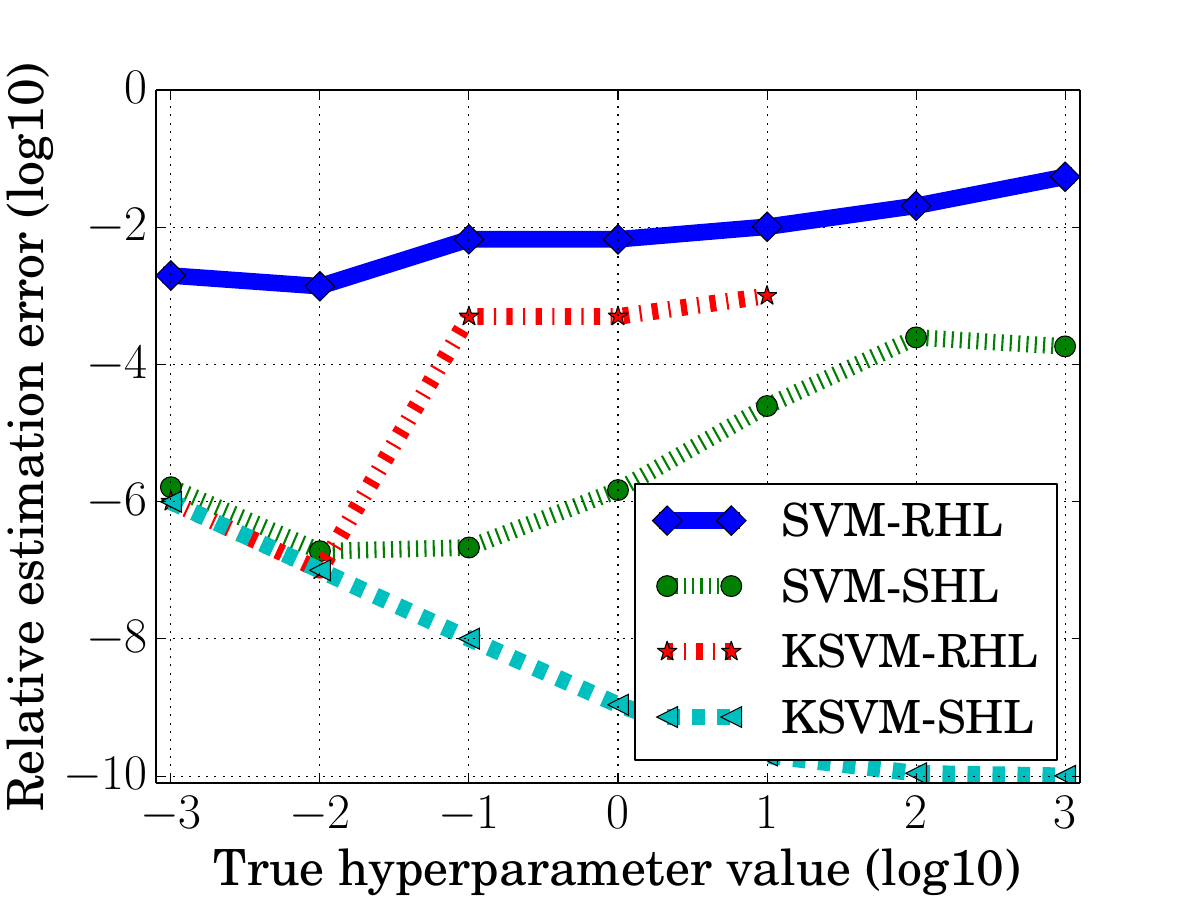}\label{clf_svc_madelon}} 
% \caption{Hyperparameter stealing results of binary SVM-based classification models.}
% \end{figure}

\begin{figure}
\center
\subfigure[Ionosphere]{\includegraphics[width=0.23\textwidth]{./src_attack/figs/clf/result-clf-lr-ionosphere-new-final.pdf}\label{clf_lr_ionosphere}} 
\subfigure[Ionosphere]{\includegraphics[width=0.23\textwidth]{./src_attack/figs/clf/result-clf-svc-ionosphere-new-final.pdf}\label{clf_svc_ionosphere}}
%\subfigure[Iris]{\includegraphics[width=0.32\textwidth]{./src_attack/figs/clf/result-clf-mlr-iris-new-final.pdf}\label{clf_mlr_ionosphere}}
\caption{Hyperparameter stealing results of classification algorithms on Ionosphere.}
\label{clf_res_attack_other}
\end{figure}

\section{Other Defense Results}

We show the hyperparameter defense results of classification models on Ionosphere and Iris in Figure~\ref{clf_res_defense_other} and evaluate real-world scenario on CovType in Figure~\ref{real_defense_clf_covType}.

% \begin{figure}
% \center
% \subfigure[Iris]{\includegraphics[width=0.23\textwidth]{./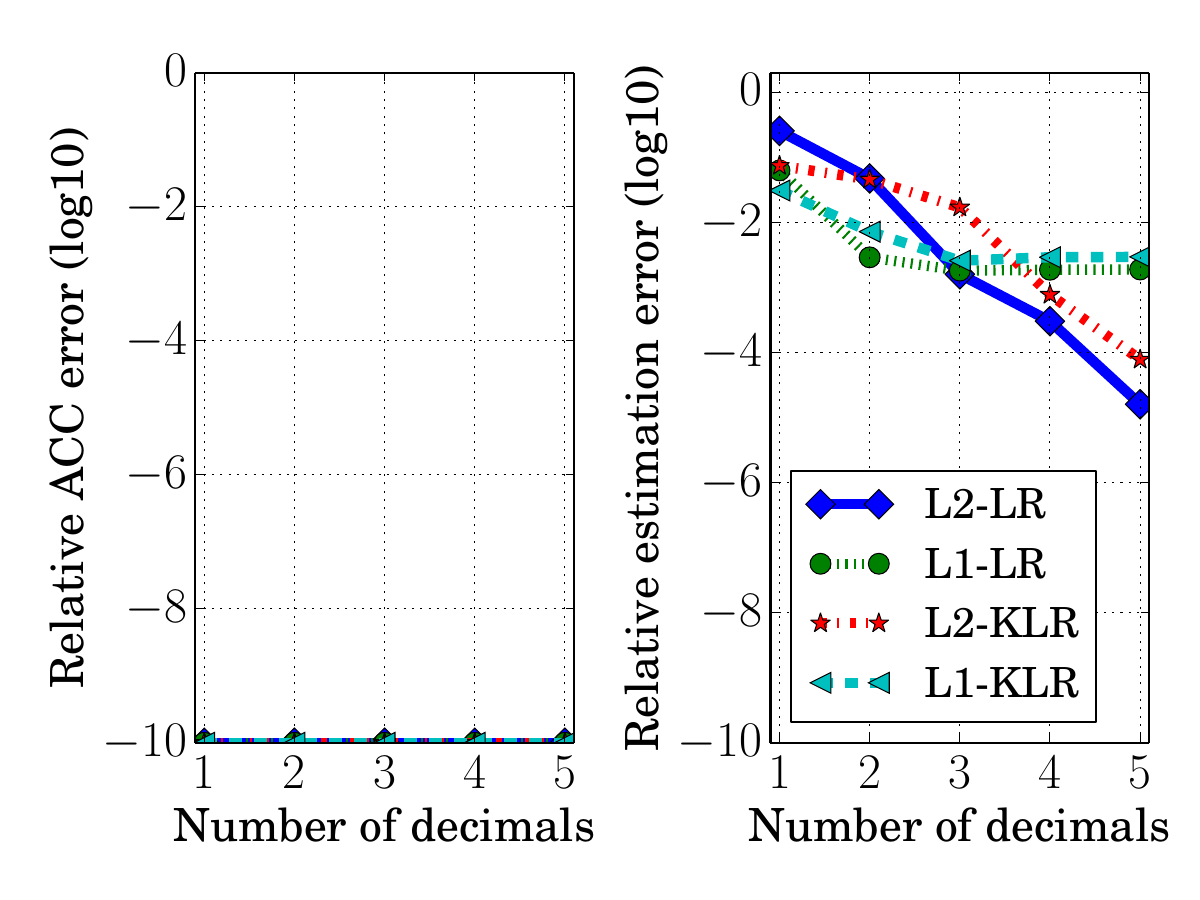}\label{lr_iris_defense}} 
% \subfigure[Ionosphere]{\includegraphics[width=0.23\textwidth]{./src_defense/figs/clf/result-clf-lr-ionosphere-new-new.pdf}\label{lr_ionosphere_defense}}
% %\subfigure[Madelon]{\includegraphics[width=0.32\textwidth]{./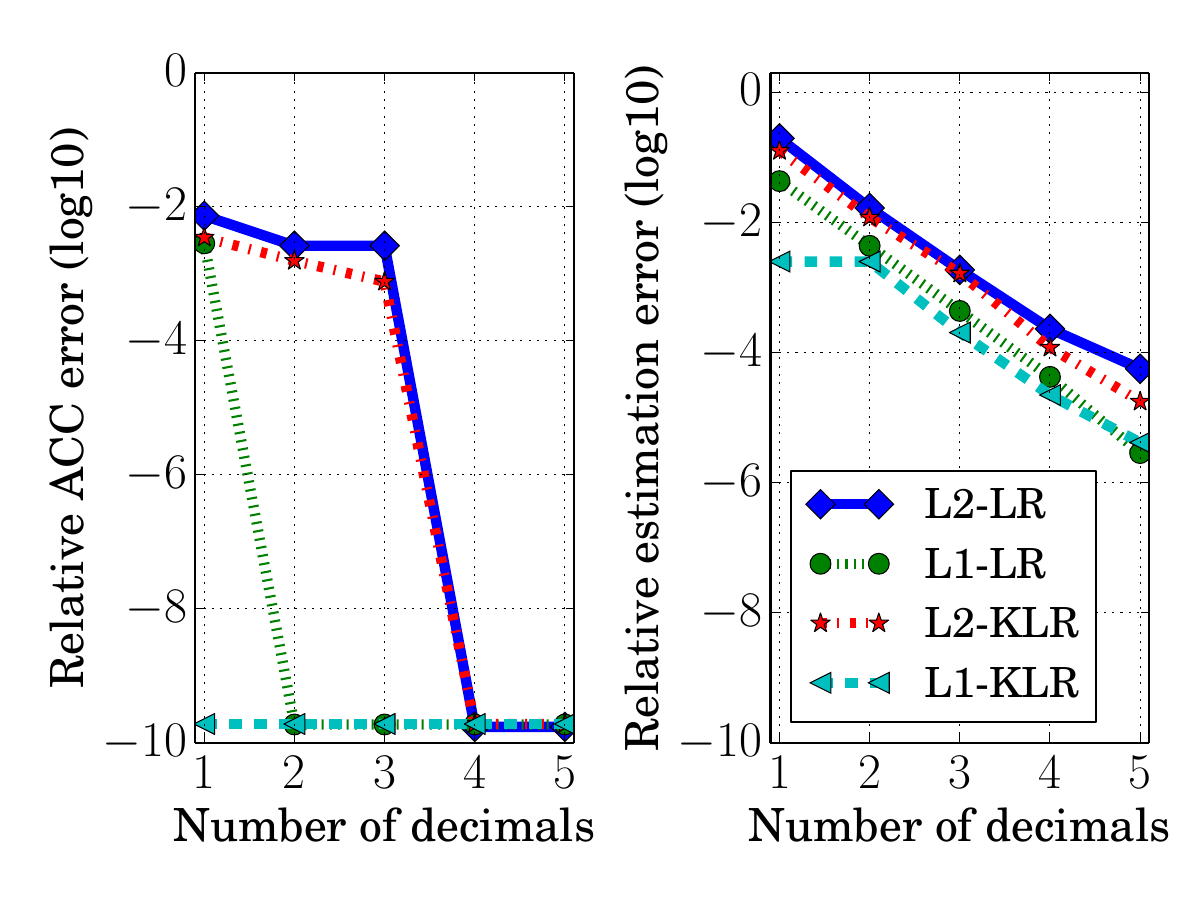}\label{lr_madelon_defense}} 
% \caption{Hyperparameter defense results of LR-based methods.}
% \label{clf_lr_res_defense}
% \end{figure}

% \begin{figure}
% \center
% \subfigure[Iris]{\includegraphics[width=0.23\textwidth]{./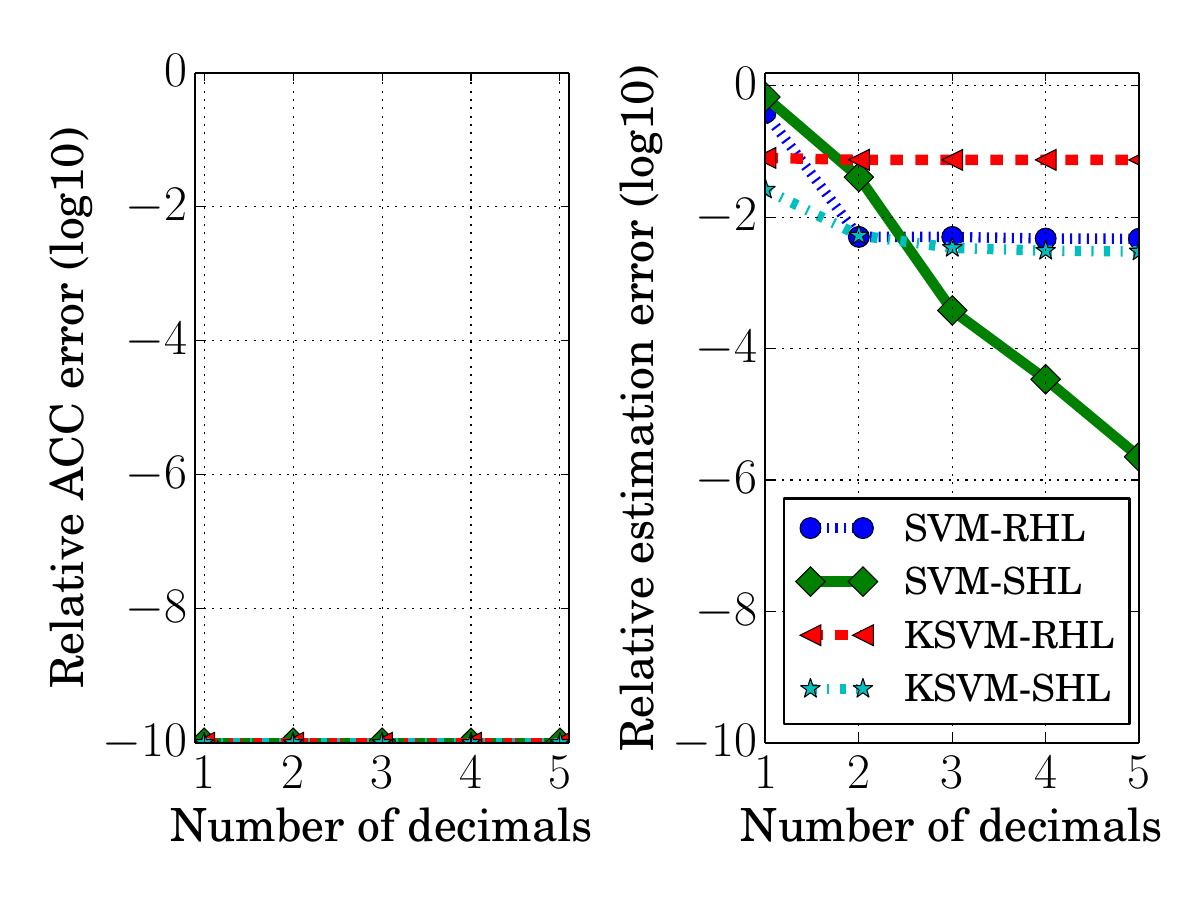}\label{svc_iris_defense}} 
% \subfigure[Ionosphere]{\includegraphics[width=0.23\textwidth]{./src_defense/figs/clf/result-clf-svc-ionosphere-new-new.pdf}\label{svc_ionosphere_defense}}
% %\subfigure[Madelon]{\includegraphics[width=0.32\textwidth]{./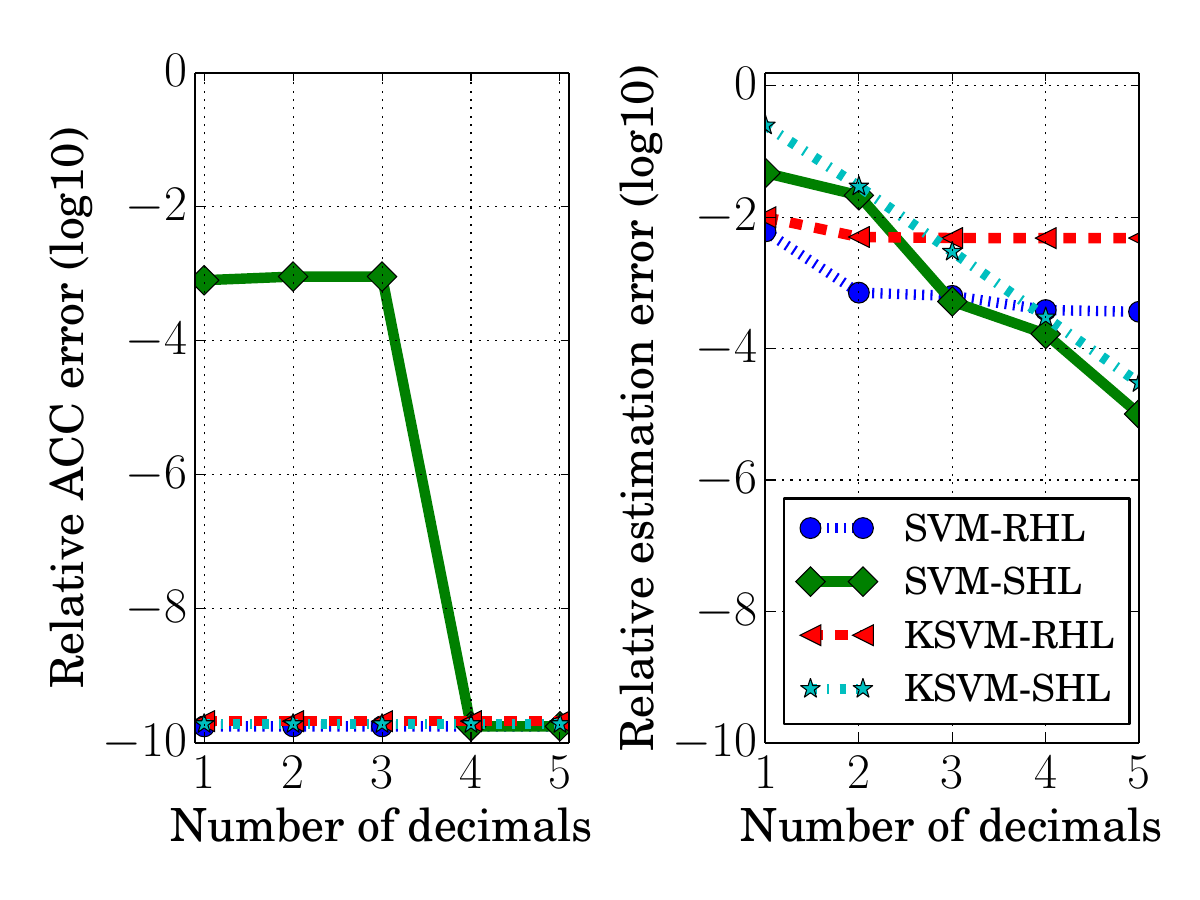}\label{svc_ionosphere_defense}} 
% \caption{Hyperparameter defense results of SVM-based methods.}
% \label{clf_svc_res_defense}
% \end{figure}

\begin{figure}
\center
\subfigure[Ionosphere]{\includegraphics[width=0.23\textwidth]{./src_defense/figs/clf/result-clf-lr-ionosphere-new-new.pdf}\label{lr_ionosphere_defense}} 
\subfigure[Ionosphere]{\includegraphics[width=0.23\textwidth]{./src_defense/figs/clf/result-clf-svc-ionosphere-new-new.pdf}\label{svc_ionosphere_defense}}
%\subfigure[Iris]{\includegraphics[width=0.32\textwidth]{./src_defense/figs/clf/result-clf-mlr-iris-new-new.pdf}\label{mlr_ionosphere_defense}}
\caption{Hyperparameter defense results of classification algorithms on Ionosphere.}
\label{clf_res_defense_other}
\end{figure}

\section{Other Sensitivity Results}

We show the hyperparameter sensitivity results of classification models on Ionosphere in Figure~\ref{clf_res_sensi_ionosphere}.

\begin{figure*}
\center
\subfigure[LR]{\includegraphics[width=0.24\textwidth]{./src_sensitivity/figs/clf/result-clf-lr-ionosphere.pdf}\label{lr_ionosphere_sensi}}
\subfigure[KLR]{\includegraphics[width=0.24\textwidth]{./src_sensitivity/figs/clf/result-clf-klr-ionosphere.pdf}\label{klr_ionosphere_sensi}}
\subfigure[SVM]{\includegraphics[width=0.24\textwidth]{./src_sensitivity/figs/clf/result-clf-svc-ionosphere.pdf}\label{svc_ionosphere_sensi}}
\subfigure[KSVM]{\includegraphics[width=0.24\textwidth]{./src_sensitivity/figs/clf/result-clf-ksvc-ionosphere.pdf}\label{ksvc_ionosphere_sensi}} 
\caption{Hyperparameter sensitivity results of classification models on Ionosphere.}
\label{clf_res_sensi_ionosphere}
\end{figure*}
