# Supplementary material for: Stealing Hyperparameters in Machine Learning
Source: arXiv:1802.05351 source file (2019-09-07)
Supplement: Supplementary file 2 [file appendix_v1.tex]

%\newpage
\appendix

\section{Details of Convex-induced Regression Models}
\label{app:cvx_reg}

\subsection{Ridge Regression}

The objective function is
\begin{align*}
%\label{ridge_reg}
\begin{split}
& \mathcal{L}_{Ridge}(\lambda, \mathbf{w}) = \| \mathbf{y}-\mathbf{X} \mathbf{w} \|_2^2 + \lambda \| \mathbf{w} \|_2^2 \\
& = \mathbf{y}^T \mathbf{y} - 2 \mathbf{w}^T \mathbf{X}^T \mathbf{y} + \mathbf{w}^T \mathbf{X}^T \mathbf{X} \mathbf{w} + \lambda \mathbf{w}^T \mathbf{w} \\
& = \mathbf{y}^T \mathbf{y} - 2 w_i \mathbf{x}_i^T \mathbf{y} - 2 \mathbf{w}_{-i}^T \mathbf{X}^T_{:,-i} \mathbf{y} + w_i \langle \mathbf{x}_i, \mathbf{x}_i \rangle w_i + 2 w_i \mathbf{x}_i^T \mathbf{X}_{:,-i} \mathbf{w}_{-i} \\
& \quad \quad + \mathbf{w}_{-i}^T \mathbf{X}^T_{:,-i} \mathbf{X}_{:,-i} \mathbf{w}_{-i} + \lambda (w_i^2 + \mathbf{w}_{-i}^T \mathbf{w}_{-i} )   
\end{split}
\end{align*}

Taking the gradient of $\mathcal{L}_{Ridge}$ with respect to $w_i$ and setting it to 0 yields
\begin{align*}
%\label{ridge_reg_grad}
\begin{split}
\frac{\partial \mathcal{L}_{Ridge}}{\partial w_i} & = -2 \mathbf{x}_i^T \mathbf{y} + 2 \langle \mathbf{x}_i, \mathbf{x}_i \rangle w_i + 2 \mathbf{x}_i^T \mathbf{X}_{:,-i} \mathbf{w}_{-i} + 2 \lambda w_i \\ 
& = 2 \langle \mathbf{x}_i, \mathbf{x}_i \rangle w_i - 2 \left\langle \mathbf{x}_i, \mathbf{r}_i \right \rangle + 2 \lambda w_i = 0 
\end{split}
\end{align*}
Then, we can estimate $\lambda$  for each $w_i$ as in Eqn~\ref{ridge_reg_soln}.

\subsection{LASSO}

The subgradient of $\mathcal{L}_{LASSO}$ with respect to $w_i$ is 
\begin{align*}
%\label{lasso_grad}
\frac{\partial \mathcal{L}_{LASSO}}{\partial w_i} = 2 \langle \mathbf{x}_i, \mathbf{x}_i \rangle w_i - 2 \left\langle \mathbf{x}_i, \mathbf{r}_i \right\rangle + \lambda \partial \|\mathbf{w}\|_1 |_{w_i},
\end{align*}
where 
\begin{align*}
\partial \| \mathbf{w} \|_1 |_{w_i} = 
\begin{cases}
-1 & \text{if } w_i < 0 \\
[-1, 1] & \text{if } w_i = 0 \\
1  & \text{if } w_i > 0.
\end{cases}
\end{align*}

Then, we have the following subgradient 
%anlaytic solution of subgradient as follows
\begin{align*}
%\label{lasso_subgrad}
\frac{\partial \mathcal{L}_{LASSO}}{\partial w_i} =  
\begin{cases}
2 \langle \mathbf{x}_i, \mathbf{x}_i \rangle w_i - 2 \left\langle \mathbf{x}_i, \mathbf{r}_i \right\rangle - \lambda & \text{if } w_i < 0 \\
\left[ - 2 \left\langle \mathbf{x}_i, \mathbf{r}_i \right \rangle - \lambda, - 2 \left\langle \mathbf{x}_i, \mathbf{r}_i \right\rangle + \lambda \right] & \text{if } \, w_i = 0 \\
2 \langle \mathbf{x}_i, \mathbf{x}_i \rangle w_i - 2 \left\langle \mathbf{x}_i, \mathbf{r}_i \right\rangle + \lambda & \text{if } w_i > 0
\end{cases}
\end{align*}
By setting it to 0, we can estimate $\lambda$ for each $w_i$ as in Eqn~\ref{lasso_soln}.

\subsection{Elastic Net}

Similarly with ridge regression and LASSO, we take the subgradient of $\mathcal{L}_{ElasticNet}$ with respect to $w_i$ as
\begin{align*}
\frac{\partial \mathcal{L}_{ElasticNet}}{\partial w_i} = 2 \langle \mathbf{x}_i, \mathbf{x}_i \rangle w_i - 2 \left\langle \mathbf{x}_i, \mathbf{r}_i \right\rangle + \lambda_2 \partial_{w_i} \mathbf{w}^T \mathbf{w} + \lambda_1 \partial \| \mathbf{w} \|_1 |_{w_i}.
\end{align*}

Incorporating into the subgraident $\partial \| \mathbf{w} \|_1 |_{w_i}$, we have 
\begin{align*}
\small
%\label{enet_subgrad}
\frac{\partial \mathcal{L}_{ElasticNet}}{\partial w_i} =  
\begin{cases}
2 \langle \mathbf{x}_i, \mathbf{x}_i \rangle w_i - 2 \left\langle \mathbf{x}_i, \mathbf{r}_i \right\rangle + 2 \lambda_2 w_i - \lambda_1 & \text{if } w_i < 0 \\
\left[ - 2 \left\langle \mathbf{x}_i, \mathbf{r}_i \right \rangle + 2 \lambda_2 w_i - \lambda_1, - 2 \left\langle \mathbf{x}_i, \mathbf{r}_i \right\rangle + 2 \lambda_2 w_i + \lambda_1 \right] & \text{if }  w_i = 0 \\
2 \langle \mathbf{x}_i, \mathbf{x}_i \rangle w_i - 2 \left\langle \mathbf{x}_i, \mathbf{r}_i \right\rangle + 2 \lambda_2 w_i + \lambda_1 & \text{if } w_i > 0
\end{cases}
\end{align*}

Then, Setting $\partial_{w_i} \mathcal{L}_{ElasticNet} = 0$, we have the equations defined in Eqn~\ref{enet_eqn_1}.

\section{Details of Convex-induced Classification Models}
\label{app:cvx_clf}

\subsection{$L_2$-regularized BLR}
\label{app:l2blr}

The gradient of $\mathcal{L}_{L_2-BLR}$ with respect to $\mathbf{w}$ is given by
\begin{align*}
\small
%\label{l2lr_grad}
\begin{split}
& \frac{\partial \mathcal{L}_{L_2-BLR}}{\partial \mathbf{w}} = - \sum_{j=1}^n \left[ y_j \frac{1}{h_\mathbf{w}(\mathbf{x}^j_T)} \frac{\partial h_\mathbf{w}(\mathbf{x}^j_T)}{\partial \mathbf{w}} + (1-y_j) \frac{-1}{1-h_\mathbf{w}(\mathbf{x}^j_T)} \frac{\partial h_\mathbf{w}(\mathbf{x}^j_T)}{\partial \mathbf{w}}\right] + 2 \lambda \mathbf{w} \\
& \quad = - \sum_{j=1}^n \left[ y_j \frac{1}{h_\mathbf{w}(\mathbf{x}^j_T)} h_\mathbf{w}(\mathbf{x}^j_T) (1-h_\mathbf{w}(\mathbf{x}^j_T)) + (1-y_j) \frac{1}{1-h_\mathbf{w}(\mathbf{x}^j_T)} h_\mathbf{w}(\mathbf{x}^j_T) (1-h_\mathbf{w}(\mathbf{x}^j_T)) \right] \frac{\partial \mathbf{w}^T \mathbf{x}^j}{\partial \mathbf{w}} + 2 \lambda \mathbf{w} \\
& \quad = - \sum_{j=1}^n \left(y_j (1-h_\mathbf{w}(\mathbf{x}^j_T)) - (1-y_j) h_\mathbf{w}(\mathbf{x}^j_T) \right) \mathbf{x}^j + 2 \lambda \mathbf{w} \\ 
& \quad = \sum_{j=1}^n (h_\mathbf{w}(\mathbf{x}^j_T) - y_j) \mathbf{x}^j + 2 \lambda \mathbf{w} \\ 
& \quad = \mathbf{X}^T (h_\mathbf{w}(\mathbf{X}) - \mathbf{y}) + 2 \lambda \mathbf{w}.
\end{split}
\end{align*}

Setting the derivative to be \textbf{0}, we can then estimate each $w_i$ as in Eqn~\ref{l2lr_soln}.

\subsection{$L_1$-regularized BLR}
\label{app:l1blr}

The subgradient of $\mathcal{L}_{L_1-BLR}$ with respect to $\mathbf{w}$ is given by
\begin{align*}
%\label{l1lr_grad}
\frac{\partial \mathcal{L}_{L_1-BLR}}{\partial \mathbf{w}} = \mathbf{X}^T (h_\mathbf{w}(\mathbf{X}) - \mathbf{y}) + \lambda \partial_\mathbf{w} \| \mathbf{w} \|_1. 
\end{align*}

Setting $\partial_\mathbf{w} \mathcal{L}_{L_1-BLR}=0$ and considering the piecewise subgradient of $\| \mathbf{w} \|_1$, we can estimate $\lambda$ for each nonzero $w_i$ as in Eqn~\ref{l1lr_soln}.

\subsection{$L_2$-regularized MLR}

The NLL for sample $\mathbf{x}^j$ can be written as
\begin{align*}
%\label{mlr_nll}
\begin{split}
& \text{NLL}_{MLR}(\mathbf{W}; \mathbf{x}^j_T, \mathbf{y}^j) = - \log \prod_{c=1}^C Pr(y_{j,c}=1|\mathbf{x}^j_T,\mathbf{W})^{y_{j,c}} \\
& \qquad = - \sum_{c=1}^C y_{j,c} \log  Pr(y_{j,c}=1|\mathbf{x}^j_T,\mathbf{W}) \\
& \qquad = - \sum_{c=1}^C y_{j,c} \langle \mathbf{w}_c, \mathbf{x}^j_T \rangle + \sum_{c=1}^C y_{j,c} \log \big( \sum_{c^\prime=1}^C \exp (\langle \mathbf{w}_{c^\prime}, \mathbf{x}^j_T ) \big) \\ 
& \qquad = - \sum_{c=1}^C y_{j,c} \langle \mathbf{w}_c, \mathbf{x}^j_T \rangle + \log \big( \sum_{c^\prime=1}^C \exp (\langle \mathbf{w}_{c^\prime}, \mathbf{x}^j_T ) \big),
\end{split}
\end{align*}
where we use the fact that $\sum_{c} y_{j,c} = 1$ in the second equation. 

For each class $c$, the derivative of $\text{NLL}_{MLR}$ for $\mathbf{w}_c$ with sample $\mathbf{x}^j$ is given by
\begin{align}
\label{mlr_nll_grad}
\begin{split} 
\frac{\partial \text{NLL}_{MLR}}{\partial \mathbf{w}_c} & = - y_{j,c} \mathbf{x}^j_T + \frac{\exp(\langle \mathbf{w}_{c^\prime}, \mathbf{x}^j_T \rangle)}{\sum_{c^\prime = 1}^C \exp (\langle \mathbf{c^\prime}, \mathbf{x}^j_T \rangle)} \mathbf{x}^j_T \\ 
& = \big( Pr(y_{j,c}=1|\mathbf{x}^j_T, \mathbf{W}) - y_{j,c} \big) \mathbf{x}^j_T.
\end{split} 
\end{align}

With Eqn~\ref{mlr_nll_grad}, for class $c$, the derivative of $\mathcal{L}_{L_2-MLR}$ with respect to $\mathbf{w}_c$ is
\begin{align}
\label{l2mlr_soln_1}
\begin{split}
\frac{\partial \mathcal{L}_{L_2-MLR}}{\partial \mathbf{w}_c} & = \sum_{j=1}^n \big( Pr(y_{j,c}=1|\mathbf{x}^j_T, \mathbf{W}) - y_{j,c} \big) \mathbf{x}^T_t + 2 \lambda \, \mathbf{w}_c \\
& = \mathbf{X}^T (\bm{\mu}_{c,\mathbf{W}}(\mathbf{X}) - \mathbf{y}_c) + 2 \lambda \, \mathbf{w}_c.
\end{split}
\end{align}

Note that above equation has the similar form as in the binary case, i.e., transposed data times an error term. By setting it to zero, for each class $c$ and each $\mathbf{x}_i$, $\lambda$ is estimated as in Eqn~\ref{l2mlr_soln_2}.

\subsection{$L_2$-regularized BKLR}
\label{app:l2bklr}

Similarly with L2-BLR, the derivative of $\mathcal{L}_{L_2-BKLR}$ with respect to $\bm{\alpha}$ is given by
\begin{align}
\label{l2klr_soln_1}
\begin{split}
\frac{\partial \mathcal{L}_{L_2-BKLR}}{\partial \bm{\alpha}}
& = \sum_{j=1}^n (h_{\bm{\alpha}}(\mathbf{k}_j) - y_j) \mathbf{k}_j + 2 \lambda \mathbf{K} \bm{\alpha} \\
%& = \mathbf{K} (h_{\bm{\alpha}}(\mathbf{K}) - \mathbf{y}) + 2 \lambda \mathbf{K} \bm{\alpha} \\
& = \mathbf{K} (h_{\bm{\alpha}}(\mathbf{K}) - \mathbf{y} + 2 \lambda \bm{\alpha}),
\end{split}
\end{align}
where we use $\mathbf{K}^T = \mathbf{K}$ and $h_{\bm{\alpha}}(\mathbf{K}) = \left[ h_{\bm{\alpha}}(\mathbf{k}_1), \cdots, h_{\bm{\alpha}}(\mathbf{k}_n) \right]^T $.

Given $\bm{\alpha}$, we set $\partial_{\bm{\alpha}} \mathcal{L}_{L_2-BKLR} = \mathbf{0}$ and consider that $\mathbf{K}$ is full rank, we thus have $h_{\bm{\alpha}}(\mathbf{K}) - \mathbf{y} + 2 \lambda \bm{\alpha} = \mathbf{0}$. Then, for each $\alpha_i$, we then estimate $\lambda$ as in Eqn~\ref{l2klr_soln}.

\subsection{$L_1$-regularized BKLR}
\label{app:l1bklr}

The subgradient of the second term in Eqn~\ref{l1klr_dual} for $\bm{\alpha}$ is
\begin{align*}
\begin{split}
\frac{\partial \| \mathbf{K} \bm{\alpha} \|_1 }{\partial \bm{\alpha}} & = \frac{\partial \| \mathbf{K} \bm{\alpha} \|_1 }{\partial \mathbf{K} \bm{\alpha}} \frac{\partial \mathbf{K} \bm{\alpha}}{\partial \bm{\alpha}} = \frac{\bm{\alpha}^T \mathbf{K}^T }{\bm{\alpha}} \textbf{sign}(\mathbf{K} \bm{\alpha}) \\ 
& =  \mathbf{K}^T \textbf{sign}(\mathbf{K} \bm{\alpha}) = \mathbf{K} \textbf{sign}(\mathbf{K} \bm{\alpha}),
\end{split}
\end{align*} 
where $\textbf{sign}(\mathbf{K} \bm{\alpha}) = \left[ \text{sign}(\mathbf{k}^1\bm{\alpha});  \text{sign}(\mathbf{k}^2\bm{\alpha}); \cdots; \text{sign}(\mathbf{k}^n\bm{\alpha}) \right]$ is the sign vector of $\mathbf{K} \bm{\alpha}$. 

Therefore, the subgradient of $\mathcal{L}_{L_1-BKLR}$ for $\bm{\alpha}$ is given by
\begin{align}
\frac{\partial \mathcal{L}_{L_1-BKLR}}{\partial \bm{\alpha}} = \mathbf{K} (h_{\bm{\alpha}}(\mathbf{K}) - \mathbf{y} + \lambda \textbf{sign}(\mathbf{K} \bm{\alpha})).
\end{align}

By setting it to $\mathbf{0}$, we estimate $\lambda$ as in Eqn~\ref{llklr_soln}.

\section{Sensitivity Analysis}

\subsection{Proof of Theorem~\ref{theorem_reg}}
\label{app:theorem_reg}

For Ridge regression, 
\begin{align}
\begin{split}
\Bigg| \frac{\Delta \hat{\lambda}_{Ridge}^{(i)}}{\Delta w_i} \Bigg| & = \Bigg|\frac{\hat{\lambda}_{Ridge}^{(i)}(w_i + \Delta w_i) - \hat{\lambda}_{Ridge}^{(i)}(w_i)}{\Delta w_i}\Bigg| \\
& = \Bigg|\frac{1}{\Delta w_i} \bigg( \frac{\langle \mathbf{x}_i, \mathbf{r}_i \rangle}{w_i + \Delta w_i} - \frac{\langle \mathbf{x}_i, \mathbf{r}_i \rangle}{w_i} \bigg)\Bigg| \\ 
& = \Bigg|\frac{1}{(w_i + \Delta w_i) w_i} \langle \mathbf{x}_i, \mathbf{r}_i \rangle \Bigg|.
\end{split}
\end{align}

For LASSO, if $w_i > 0$
\begin{align}
\Bigg| \frac{\Delta \hat{\lambda}_{LASSO}^{(i)}}{\Delta w_i} \Bigg| = \Bigg| \frac{-2 \langle \mathbf{x}_i, \mathbf{x}_i \rangle (w_i + \Delta w_i) + 2 \langle \mathbf{x}_i, \mathbf{x}_i \rangle w_i }{\Delta w_i} \Bigg| = \big| 2 \langle \mathbf{x}_i, \mathbf{x}_i \rangle \big|.
\end{align}
%Similarly, $\frac{\Delta \hat{\lambda}_{LASSO}^{(i)}}{\Delta w_i} = 2 \langle \mathbf{x}_i, \mathbf{x}_i \rangle $ if $w_i < 0$.

Note that the variation of Ridge regression depends on both the true $w_i$ and the changed $w_i + \Delta w_i$; While for LASSO, it is independent of both $w_i$ and $\Delta w_i$ and is constant. As a consequence, the estimated $\hat{\lambda}_{LASSO}^{(i)}$ of LASSO will be almost not affected if the length of $\mathbf{x}_i$ is small, which can be obtained through preprocessing the raw data; However, $\hat{\lambda}_{Ridge}^{(i)}$ of Ridge regression can be changed dramatically once $w_i$ is much smaller than 1, or/and the absolute value of $\Delta w_i$ is comparable with $w_i$ (We mention in advance that $\Delta w_i$ and $w_i$ always have the opposite sign in our experiments, and thus when $|\Delta w_i| \rightarrow |w_i|, w_i + \Delta w_i \rightarrow 0$). 
%, which is often the case. For instance, $l_2$ norm of $\mathbf{w}$ is required to be less than or equal 1, i.e., $\| \mathbf{w} \|_2 \leq 1$.  

For Elastic Net, since it incorporates both $l_2$ and $l_1$ regularizations, the sensitivity of $\hat{\lambda_2}^{(i)}$ and $\hat{\lambda_1}^{(i)}$ share the same property with $\hat{\lambda}_{Ridge}^{(i)}$ in Ridge regression and $\hat{\lambda}_{LASSO}^{(i)}$ in LASSO. Specifically,

For Kernel Ridge regression, the sensitivity is 
\begin{align}
\label{KernelRidge_sensi}
\begin{split}
\Bigg| \frac{\Delta \hat{\lambda}_{KernelRidge}^{(j)}}{\Delta \alpha_j} \Bigg| & = \Bigg| \frac{1}{\Delta \alpha_j} \bigg( \frac{y_j}{\alpha_j + \Delta \alpha_j} - \frac{y_j}{\alpha_j} \bigg) \Bigg| \\
& = \Bigg| -\frac{1}{(\alpha_j + \Delta \alpha_j) \alpha_j} y_j \Bigg|,   
\end{split}
\end{align}
which has a similar form with Ridge regression. Thus, the far smaller $\alpha_j$ is than 1, or the much closer $\Delta \alpha_j$ is to $\alpha_j$, the more sensitive Kernel Ridge regression is.

\subsection{Proof of Theorem~\ref{theorem_lr}}
\label{app:theorem_lr}

First, we consider $L_2$-BLR and $L_1$-BLR.

For $L_2$-BLR, 
$\hat{\lambda}_{L_2-BLR}^{(i)} (w_i + \Delta w_i) = - \frac{\langle \mathbf{x}_i, h_{\mathbf{w}+\Delta w_i}(\mathbf{X}) - \mathbf{y} \rangle}{ 2 (w_i + \Delta w_i)}$, 
where $h_{\mathbf{w}+\Delta w_i}(\mathbf{X}) = \left[ h_{\mathbf{w}+\Delta w_i}(\mathbf{x}^1_T), h_{\mathbf{w}+\Delta w_i}(\mathbf{x}^2_T), \cdots, h_{\mathbf{w}+\Delta w_i}(\mathbf{x}^n_T) \right]^T $ and $h_{\mathbf{w}+\Delta w_i} (\mathbf{x}^i_T) = \frac{1}{1 + \exp(\sum_{j \neq i} w_j x_{i,j}) + (w_i + \Delta w_i) x_{i,i}}$ (One should notice that the notation $\mathbf{w}+\Delta w_i$ here is not so ``formal", as $\Delta w_i$ is not added to all elements of $\mathbf{w}$, but to its $i$-th entry. We use such notation for ease of writing).
Therefore, 
\begin{align}
\label{L2_BLR_sensi}
\begin{split}
& \Bigg| \frac{\Delta \hat{\lambda}_{L_2-BLR}^{(i)}}{\Delta w_i} \Bigg| = \Bigg| \frac{\hat{\lambda}_{L_2-BLR}^{(i)} (w_i + \Delta w_i) - \hat{\lambda}_{L_2-BLR}^{(i)} (w_i)}{\Delta w_i} \Bigg| \\
& = \Bigg| \frac{1}{\Delta w_i} \bigg( -\frac{1}{2(w_i + \Delta w_i)} \langle \mathbf{x}_i, h_{\mathbf{w}+\Delta w_i}(\mathbf{X}) - \mathbf{y} \rangle + \frac{1}{2 w_i} \langle \mathbf{x}_i, h_{\mathbf{w}}(\mathbf{X}) - \mathbf{y} \rangle \bigg) \Bigg| \\
& = \Bigg| \frac{1}{\Delta w_i} \bigg( - \frac{1}{2(w_i + \Delta w_i)} \langle \mathbf{x}_i, h_{\mathbf{w}+\Delta w_i}(\mathbf{X}) - \mathbf{y} \rangle + \frac{1}{2(w_i + \Delta w_i)} \langle \mathbf{x}_i, h_{\mathbf{w}}(\mathbf{X}) - \mathbf{y} \rangle \bigg) \\ 
& \quad + \frac{1}{\Delta w_i} \bigg( - \frac{1}{2(w_i + \Delta w_i)} \langle \mathbf{x}_i, h_{\mathbf{w}}(\mathbf{X}) - y \rangle + \frac{1}{2 w_i} \langle \mathbf{x}_i, h_{\mathbf{w}}(\mathbf{X}) - \mathbf{y} \rangle \bigg) \Bigg| \\
& = \Bigg| - \frac{1}{2(w_i + \Delta w_i) \Delta w_i} \langle \mathbf{x}_i, h_{\mathbf{w}+\Delta w_i}(\mathbf{X}) - h_{\mathbf{w}}(\mathbf{X}) \rangle \\
& \quad + \frac{1}{2 w_i (w_i + \Delta w_i)} \langle \mathbf{x}_i, h_{\mathbf{w}}(\mathbf{X}) - \mathbf{y} \rangle \Bigg|. 
\end{split}
\end{align}

For $L_1$-BLR, 
\begin{align}
\label{L1_BLR_sensi}
\begin{split}
\Bigg| \frac{\Delta \hat{\lambda}_{L_1-BLR}^{(i)}}{\Delta w_i} \Bigg| & = \Bigg| \frac{1}{\Delta w_i} \big( \langle \mathbf{x}_i, h_{\mathbf{w} + \Delta w_i}(\mathbf{X}) - \mathbf{y} \rangle - \langle \mathbf{x}_i, h_{\mathbf{w}}(\mathbf{X}) - \mathbf{y} \rangle \big) \Bigg| \\
& = \Bigg| \frac{1}{\Delta w_i} \langle \mathbf{x}_i, h_{\mathbf{w} + \Delta w_i}(\mathbf{X}) - h_{\mathbf{w}}(\mathbf{X}) \rangle \Bigg|.
\end{split}
\end{align}
%Similarly, if $w_i <0$, $\frac{\Delta \hat{\lambda}_{L_1-BLR}^{(i)}}{\Delta w_i} = - \frac{1}{\Delta w_i} \langle \mathbf{x}_i, h_{\mathbf{w} + \Delta w_i}(\mathbf{X}) - h_{\mathbf{w}}(\mathbf{X}) \rangle $.

Comparing Eqn~\ref{L2_BLR_sensi} with Eqn~\ref{L1_BLR_sensi} and reusing the aforementioned analysis, we observe that once the absolute value of $w_i$ is one or two orders of magnitude smaller than 1 or $\Delta w_i$ is comparable with $w_i$, then $L_2$-BLR is more sensitive than $L_1$-BLR in terms of the variation of $w_i$. 

Then, we consider $L_2$-BKLR and $L_1$-BKLR.

For $L_2$-BKLR,
\begin{align}
\begin{split}
& \Bigg| \frac{\Delta \hat{\lambda}_{L_2-BKLR}^{(j)}}{\Delta \alpha_j} \Bigg| = \Bigg| \frac{1}{\Delta \alpha_j} \bigg( \frac{y_j - h_{\bm{\alpha} + \Delta \alpha_j}(\mathbf{k}_j)}{2(\alpha_j + \Delta \alpha_j)} - \frac{y_j - h_{\bm{\alpha}} (\mathbf{k}_j)}{2 \alpha_j} \bigg) \Bigg| \\
& = \Bigg| - \frac{h_{\bm{\alpha}+\Delta \alpha_j}(\mathbf{k}_j) - h_{\bm{\alpha}}(\mathbf{k}_j)}{2(\alpha_j + \Delta \alpha_j) \Delta \alpha_j} + \frac{h_{\bm{\alpha}}(\mathbf{k}_j) - y_j}{2(\alpha_j + \Delta \alpha_j) \alpha_j} \Bigg|,
\end{split}
\end{align}
where $h_{\bm{\alpha}+\Delta \alpha_j} (\mathbf{k}_j) = \frac{1}{1+ \exp(\langle \bm{\alpha}, \mathbf{k}_j \rangle + \Delta \alpha_j k_{j,j})}$.

For $L_1$-BKLR, %if $\mathbf{k}^j \bm{\alpha} < 0$,
\begin{align}
\Bigg| \frac{\Delta \hat{\lambda}_{L_1-BKLR}^{(j)}}{\Delta \alpha_j} \Bigg| = \Bigg| \frac{1}{\Delta \alpha_j} \big( h_{\bm{\alpha}+\Delta \alpha_j}(\mathbf{k}_j) - h_{\bm{\alpha}}(\mathbf{k}_j) \big) \Bigg|.
\end{align}
%and $\frac{\Delta \hat{\lambda}_{L_1-BKLR}^{(j)}}{\Delta \alpha_j} = \frac{1}{\Delta \alpha_j} \big( - h_{\bm{\alpha}+\Delta \alpha_j}(\mathbf{k}_j) + h_{\bm{\alpha}}(\mathbf{k}_j) \big)$ if $\mathbf{k}^j \bm{\alpha} > 0$. 

We can perform similar sensitivity analysis of $L_2$-BKLR and $L_1$-BKLR as that of $L_2$-BLR and $L_1$-BLR. Namely, if the absolute value of $\alpha_j$ is one or two orders of magnitude smaller than 1 or $\Delta \alpha_j$ is comprable with $\alpha_j$, then L2-BKLR is more sensitive than L1-BKLR.

\subsection{Proof of Theorem~\ref{theorem_svc}}
\label{app:theorem_svc}

First, we consider BLSVC-RHL and BLSVC-SHL.

For BLSVC-RHL, 
\begin{align}
\label{BLSVC_RHL_sensi}
\begin{split}
& \Bigg| \frac{\Delta \hat{C}_{BLSVC-RHL}^{(i)}}{\Delta w_i} \Bigg| = \\
& \Bigg| \frac{1}{\Delta w_i} \Bigg( \frac{w_i + \Delta w_i}{\sum\limits_{j, y_j \big( \langle \mathbf{w}, \mathbf{x}_T^j \rangle + \Delta w_i x_{j,i} \big) < 1} y_j x_{j,i}} - \frac{w_i}{\sum\limits_{j, y_j \langle \mathbf{w}, \mathbf{x}_T^j \rangle <1} y_j x_{j,i} } \Bigg) \Bigg|. 
\end{split}
\end{align}

For BLSVC-SHL, 
\begin{align}
\label{BLSVC_SHL_sensi}
\begin{split}
& \Bigg| \frac{\Delta \hat{C}_{BLSVC-SHL}^{(i)}}{\Delta w_i} \Bigg| = \\
&  \Bigg| \frac{1}{\Delta w_i} \Bigg( \frac{w_i + \Delta w_i}{\sum\limits_{j, y_j \big( \langle \mathbf{w}, \mathbf{x}_T^j \rangle + \Delta w_i x_{j,i} \big) < 1} 2 y_j x_{j,i} \big(1 - y_j \big( \langle \mathbf{w}, \mathbf{x}_T^j \rangle + \Delta w_i x_{j,i} \big) \big) } \\
& \quad - \frac{w_i}{\sum\limits_{j, y_j \langle \mathbf{w}, \mathbf{x}_T^j \rangle <1} 2 y_j x_{j,i} \big(1 - y_j \langle \mathbf{w}, \mathbf{x}_T^j \rangle \big) } \Bigg) \Bigg| .
\end{split}
\end{align}

Comparing Eqn~\ref{BLSVC_RHL_sensi} and Eqn~\ref{BLSVC_SHL_sensi}, we notice that their difference is between the factor $2\big(1 - y_j \big( \langle \mathbf{w}, \mathbf{x}_T^j \rangle + \Delta w_i x_{i,i} \big) \big)$ and 1. Taking into account the property of SVC, we know that when the training set $\mathbf{X}$ can be (approximately) linearly separable, then $y_j \langle \mathbf{w}, \mathbf{x}_T^j \rangle $ is close to 1, i.e., $1-y_j \langle \mathbf{w}, \mathbf{x}_T^j \rangle $ is a small positive number. Therefore, by adding $\Delta w_i$ such that the sign of $1- y_j \big( \langle \mathbf{w}, \mathbf{x}_T^j \rangle + \Delta w_i x_{i,i} \big) \big)$ is still positive, we conclude that $ 1- y_j \big( \langle \mathbf{w}, \mathbf{x}_T^j \rangle + \Delta w_i x_{i,i} \big) \big) < \frac{1}{2}$, and thus $\hat{C}_{BLSVC-SHL}^{(i)}$ is more sensitive than $\hat{C}_{BLSVC-RHL}^{(i)}$.

Then, we consider BKSVC-RHL and BKSVC-SHL.

For BKSVC-RHL, 
\begin{align}
\label{BKSVC_RHL_sensi}
\begin{split}
& \Bigg| \frac{\Delta \hat{C}_{BKSVC-RHL}^{(i)}}{\Delta \alpha_i} \Bigg|  = \\ 
& \Bigg| \frac{1}{\Delta \alpha_i} \Bigg( \frac{\mathbf{k}^i \bm{\alpha} + k_{ii} \Delta \alpha_i}{\sum\limits_{j, y_j (\langle \bm{\alpha}, \mathbf{k}_j \rangle + \Delta \alpha_i k_{i,j}) <1} y_j k_{j,i}} - \frac{\mathbf{k}^i \bm{\alpha}}{\sum\limits_{j, y_j \langle \bm{\alpha}, \mathbf{k}_j \rangle <1} y_j k_{j,i} } \Bigg) \Bigg|.
\end{split}
\end{align}

For BKSVC-SHL
\begin{align}
\label{BKSVC_SHL_sensi}
\begin{split}
& \Bigg| \frac{\Delta \hat{C}_{BKSVC-SHL}^{(i)}}{\Delta \alpha_i} \Bigg| = \\
& \Bigg| \frac{1}{\Delta \alpha_i} \Bigg( \frac{\mathbf{k}^i \bm{\alpha} + k_{ii} \Delta \alpha_i}{\sum\limits_{j, y_j (\langle \bm{\alpha}, \mathbf{k}_j \rangle + \Delta \alpha_i k_{i,j}) <1} 2 y_j k_{j,i} \big( 1 - y_j (\langle \bm{\alpha}, \mathbf{k}_j \rangle + \Delta \alpha_i k_{i,j}) \big)} \\
& \quad -  \frac{\mathbf{k}^i \bm{\alpha}}{\sum\limits_{j, y_j \langle \bm{\alpha}, \mathbf{k}_j \rangle <1} 2 y_j k_{j,i} \big( 1 - y_j \langle \bm{\alpha}, \mathbf{k}_j \rangle \big)} \Bigg) \Bigg|.
\end{split}
\end{align}

Similar results can be obtained, i.e., $\hat{C}_{BKSVC-SHL}^{(i)}$ is more sensitive than $\hat{C}_{BKSVC-RHL}^{(i)}$,  as $1 - y_j (\langle \bm{\alpha}, \mathbf{k}_j \rangle + \Delta \alpha_i k_{i,j}) < \frac{1}{2}$ is often satisfied.
