# Supplementary material for: Stealing Hyperparameters in Machine Learning
Source: arXiv:1802.05351 source file (2019-09-07)
Supplement: Supplementary file 3 [file appendix.tex]

%\newpage
\appendix

\section{Attacks to Other Learning Algorithms}
\label{app:other}

\myparatight{LASSO}
%\label{app:lasso}
The objective function of LASSO is:
\begin{small}
\begin{align}
\label{lasso}
\mathcal{L}(\mathbf{w}) = \| \mathbf{y}-\mathbf{X}^T\mathbf{w} \|_2^2 + \lambda \| \mathbf{w} \|_1,
\end{align}
\end{small}
whose gradient  is:
\begin{small}
\begin{align*}
%\label{lasso_grad}
\frac{\partial \mathcal{L}(\mathbf{w})}{\partial \mathbf{w}} = -2 \mathbf{X y} + 2 \mathbf{X}\mathbf{X}^T\mathbf{w} + \lambda \mathbf{s},
%2  \mathbf{x}_i^T \mathbf{x}_i \mathbf{w}  - 2 \left\langle \mathbf{x}_i, \mathbf{r}_i \right\rangle + \lambda \partial \|\mathbf{w}\|_1 |_{w_i},
\end{align*}
\end{small}
where the $i$th entry $s_i$ of the vector $\mathbf{s}$ is defined as:
\begin{small}
\begin{align}
\label{vectors}
s_i=\frac{\partial |w_i|}{\partial w_i}=
\begin{cases}
-1 & \text{if } w_i < 0 \\
0 & \text{if } \, w_i = 0 \\
1 & \text{if } w_i > 0
\end{cases}
\end{align}
\end{small}
 $| w_i |$ is \emph{not differentiable} when $w_i=0$, so
we define the derivative at $w_i=0$ as 0, which means that we do not use the model parameters that are 0 to estimate the hyperparameter. By setting the gradient to be $\mathbf{0}$, we can estimate $\lambda$ using Eqn.~\ref{fianl_est} with $\mathbf{a}=\mathbf{s}$ and $\mathbf{b}=-2 \mathbf{X y} + 2 \mathbf{X}\mathbf{X}^T\mathbf{w}$.
 
 We note that if $\lambda \geq \lambda_{\max} = \| \mathbf{X} \mathbf{y} \|_{\infty}$, then $\mathbf{w} = \mathbf{0}$. In such cases, we cannot estimate the exact hyperparameter. However, in practice,  $\lambda \geq \lambda_{\max}$ must hold in order to learn meaningful model parameters. 
%  It is because $\mathbf{0}$ is optimal if $(\mathbf{X}^T \mathbf{y})_j \in [-\lambda, \lambda]$, for any $j$. Therefore, $\hat{\lambda}^{(i)}_{LASSO} < \max_i |\langle \mathbf{y}, \mathbf{x}_i \rangle|$.

\myparatight{$L_1$-regularized LR (L1-LR)} The objective function of L1-LR is:
\begin{small}
\begin{align}
\label{l2lr}
\mathcal{L}(\mathbf{w}) = \text{L}(\mathbf{X}, \mathbf{y}, \mathbf{w}) + \lambda \| \mathbf{w} \|_1,
\end{align}
\end{small}
where $\text{L}(\mathbf{X}, \mathbf{y}, \mathbf{w})$=$-\sum_{i=1}^n  ( y_i \, \log h(\mathbf{x}_i,\mathbf{w}) + (1-y_i)$ $ \log (1- h(\mathbf{x}_i,\mathbf{w})))$ and $h(\mathbf{x},\mathbf{w})$ is defined to be $\frac{1}{1+\exp{(- \mathbf{w}^T \mathbf{x})}} $. 
The gradient of the objective function with respect to $\mathbf{w}$ is:
\begin{small}
\begin{align*}
%\label{l2lr_grad}
\begin{split}
& \frac{\partial \mathcal{L}(\mathbf{w})}{\partial \mathbf{w}} =
% - \sum_{i=1}^n \left[ \frac{y_i}{h_\mathbf{w}(\mathbf{x}_i)} \frac{\partial h_\mathbf{w}(\mathbf{x}_i)}{\partial \mathbf{w}} + \frac{-(1-y_i)}{1-h_\mathbf{w}(\mathbf{x}_i)} \frac{\partial h_\mathbf{w}(\mathbf{x}_i)}{\partial \mathbf{w}}\right] + 2 \lambda \mathbf{w} \\
%& \quad = - \sum_{j=1}^n \left[ \frac{y_j }{h_\mathbf{w}(\mathbf{x}_i)} h_\mathbf{w}(\mathbf{x}_i) (1-h_\mathbf{w}(\mathbf{x}_i)) - \frac{(1-y_j)}{1-h_\mathbf{w}(\mathbf{x}_i)} h_\mathbf{w}(\mathbf{x}_i) (1-h_\mathbf{w}(\mathbf{x}_i)) \right] \frac{\partial \mathbf{w}^T \mathbf{x}^j}{\partial \mathbf{w}} + 2 \lambda \mathbf{w} \\
%& \quad = - \sum_{i=1}^n \left(y_i (1-h_\mathbf{w}(\mathbf{x}_i)) - (1-y_i) h_\mathbf{w}(\mathbf{x}_i) \right) \mathbf{x}_i + 2 \lambda \mathbf{w} \\ 
%& \quad = \sum_{i=1}^n (h_\mathbf{w}(\mathbf{x}_i) - y_i) \mathbf{x}_i + 2 \lambda \mathbf{w} = 
\mathbf{X} (\mathbf{h}  - \mathbf{y}) + \lambda \mathbf{s},
\end{split}
\end{align*}
\end{small}
where  $\mathbf{h} = \left[ h(\mathbf{x}_1,\mathbf{w}); h(\mathbf{x}_2,\mathbf{w}); \cdots; h(\mathbf{x}_n,\mathbf{w}) \right]$ and $\mathbf{s}$ is defined in Eqn.~\ref{vectors}. 
Via setting the gradient to be \textbf{0}, we can estimate $\lambda$ using Eqn.~\ref{fianl_est} with
$\mathbf{a} = \mathbf{s}$ and $\mathbf{b} = \mathbf{X} (\mathbf{h}  - \mathbf{y})$.

%\begin{small}
%\begin{align}
%\label{l1lr}
%\mathcal{L}(\mathbf{w}) = \sum_{i=1}^n \text{NLL}(\mathbf{w};\mathbf{x}_i,y_i) + \lambda \| \mathbf{w} \|_1,
%%\mathcal{L}_{L1-LR}(\lambda, \mathbf{w}) = - \sum_{i=1}^n \left[ y_j \log h_\mathbf{w}(\mathbf{x}_j) + (1-y_j) \log(1-h_\mathbf{w}(\mathbf{x}_j)) \right] + \lambda \| \mathbf{w} \|_1.
%\end{align}
%\end{small}
%where it uses cross entropy loss function and $L_1$ regularization. Generally, the optimal $\mathbf{w}$ can be approximately solved via LBFGS~\cite{liu1989limited}. 
%The subderivative of $\mathcal{L}(\mathbf{w})$ with respect to $\mathbf{w}$ is 
%\begin{small}
%\begin{align*}
%%\label{l1lr_grad}
%\frac{\partial \mathcal{L}_{L1-LR}}{\partial \mathbf{w}} = \mathbf{X} (h_\mathbf{w}(\mathbf{X}) - \mathbf{y}) + \lambda \partial_\mathbf{w} \| \mathbf{w} \|_1. 
%\end{align*}
%\end{small}
%Setting it to be \textbf{0} and removing zero $w_i$, we have
%$\mathbf{a} = \text{sign}(\mathbf{w}) $ and $\mathbf{b} = \mathbf{X} (h_\mathbf{w}(\mathbf{X}) - \mathbf{y}) $.

\myparatight{SVM with regular hinge loss (SVM-RHL)} 
The objective function of SVM-RHL is:
\begin{small}
\begin{align}
\label{hl_bsvc}
\mathcal{L}(\mathbf{w}) = \sum_{i=1}^n L(\mathbf{x}_i, y_i, \mathbf{w}) + \lambda \| \mathbf{w} \|_2^2, 
\end{align}
\end{small}
where $L(\mathbf{x}_i, y_i, \mathbf{w}) = \max(0, 1 - y_i  \mathbf{w}^T \mathbf{x}_i)$ is called regular hinge loss function.  
The gradient with respect to $\mathbf{w}$ is: 
\begin{small}
\begin{align*}
%\label{RHL_subg}
\frac{\partial L}{\partial \mathbf{w}} = 
\begin{cases}
-y_i \mathbf{x}_i & \text{if } y_i  \mathbf{w}^T \mathbf{x}_i  < 1 \\
%[-y_j \mathbf{x}_j, \mathbf{0}] & \text{if } y_j \langle \mathbf{w}, \mathbf{x}_j \rangle = 1 \\
\mathbf{0} & \text{if } y_i  \mathbf{w}^T \mathbf{x}_i  > 1,
\end{cases}
\end{align*}
\end{small}
where $L(\mathbf{x}_i, y_i, \mathbf{w})$ is non-differentiable at the point where  $y_i  \mathbf{w}^T \mathbf{x}_i  = 1$.
 We estimate $\lambda$ using only training instances $\mathbf{x}_i$ that satisfy $y_i  \mathbf{w}^T \mathbf{x}_i  < 1$. 
Specifically, we estimate $\lambda$ using Eqn.~\ref{fianl_est} with $\mathbf{a} = 2 \mathbf{w}$ and $\mathbf{b} = \sum_{i=1}^n -y_i \mathbf{x}_i \mathbf{1}_{y_i  \mathbf{w}^T \mathbf{x}_i < 1}$, where $\mathbf{1}_{y_i  \mathbf{w}^T \mathbf{x}_i < 1}$ is an indicator function with value 1 if $ y_i  \mathbf{w}^T \mathbf{x}_i < 1 $ and 0 otherwise. 

\myparatight{SVM with square hinge loss (SVM-SHL)}  
The objective function of SVM-SHL is:
\begin{small}
\begin{align}
\label{hl_bsvc}
\mathcal{L}(\mathbf{w}) = \sum_{i=1}^n L(\mathbf{x}_i, y_i, \mathbf{w}) + \lambda \| \mathbf{w} \|_2^2, 
\end{align}
\end{small}
where $L(\mathbf{x}_i, y_i, \mathbf{w}) = \max(0, 1 - y_i  \mathbf{w}^T \mathbf{x}_i)^2$ is called square hinge loss function.  
The gradient with respect to $\mathbf{w}$ is: 
\begin{small}
\begin{align*}
%\label{RHL_subg}
\frac{\partial L}{\partial \mathbf{w}} = 
\begin{cases}
-2y_i \mathbf{x}_i (1 - y_i  \mathbf{w}^T \mathbf{x}_i) & \text{if } y_i  \mathbf{w}^T \mathbf{x}_i  \leq 1 \\
%[-y_j \mathbf{x}_j, \mathbf{0}] & \text{if } y_j \langle \mathbf{w}, \mathbf{x}_j \rangle = 1 \\
\mathbf{0} & \text{if } y_i  \mathbf{w}^T \mathbf{x}_i  > 1.
\end{cases}
\end{align*}
\end{small}
  
Therefore, we estimate $\lambda$ using Eqn.~\ref{fianl_est} with $\mathbf{a} =  \mathbf{w}$ and $\mathbf{b} = \sum_{i=1}^n - y_i \mathbf{x}_i (1 - y_i  \mathbf{w}^T \mathbf{x}_i) \mathbf{1}_{y_i  \mathbf{w}^T \mathbf{x}_i \leq 1}$.

%$L_{SHL}(y_j, \langle \mathbf{w}, \mathbf{x}_j \rangle) = \max(0, 1 - y_j \langle \mathbf{w}, \mathbf{x}_j \rangle)^2$. SHL is convex, smooth, and differential. Its subgradient with respect to $\mathbf{w}$ is given by
%\begin{small}
%\begin{align*}  
%%\label{SHL_subg}
%\frac{\partial L_{SHL}}{\partial \mathbf{w}} =
%\begin{cases}
%-2 y_j \mathbf{x}_j (1 - y_j \langle \mathbf{w}, \mathbf{x}_j \rangle) & \text{if } y_j \langle \mathbf{w}, \mathbf{x}_j \rangle <= 1 \\
%\mathbf{0}  & \text{if } y_j \langle \mathbf{w}, \mathbf{x}_j \rangle > 1
%\end{cases}
%\end{align*}
%\end{small}
%Therefore, for SVM-SHL, we have $\mathbf{a} = \mathbf{w}$ and $\mathbf{b} = \sum_{j=1}^n -2 y_j \mathbf{x}_j (1 - y_j \langle \mathbf{w}, \mathbf{x}_j \rangle) \mathbf{1}_{y_j \langle \mathbf{w}, \mathbf{x}_j \rangle \leq 1}$.

%\myparatight{SVM with square hinge loss (SVM-SHL)}

\myparatight{$L_1$-regularized kernel LR (L1-KLR)} 
The objective function of L1-KLR is:
\begin{small}
\begin{align}
\label{l2klr_dual}
\begin{split}
\mathcal{L}(\bm{\alpha}) =\text{L}(\mathbf{X}, \mathbf{y}, \mathbf{\bm \alpha}) + 
\lambda \| \mathbf{K} \bm{\alpha} \|_1,
\end{split}
\end{align} 
\end{small}
where $\text{L}(\mathbf{X}, \mathbf{y}, \mathbf{\bm \alpha}) = $ $-\sum_{i=1}^n ( y_i \, \log h(\mathbf{x}_i,\mathbf{\bm \alpha}) + (1-y_i)$ $ \log (1- h(\mathbf{x}_i,\mathbf{\bm \alpha})))$ and $h(\mathbf{x},\mathbf{\bm \alpha}) = \frac{1}{1 + \exp{(- \sum_{j=1}^n  \alpha_j \phi(\mathbf{x})^T\phi(\mathbf{x}_j))}}$. 
%$\bm{\alpha}$ is often solved approximately via coordinate descent.  
The gradient of the objective function with respect to $\bm{\alpha}$ is:
\begin{small}
\begin{align*}
%\label{l2klr_soln_1}
\begin{split}
\frac{\partial \mathcal{L}(\bm{\alpha})}{\partial \bm{\alpha}} 
%& = \sum_{j=1}^n (h_{\bm{\alpha}}(\mathbf{k}_j) - y_j) \mathbf{k}_j + 2 \lambda \mathbf{K} \bm{\alpha} \\
& = \mathbf{K} (\mathbf{h} - \mathbf{y} +  \lambda \mathbf{t}),
\end{split}
\end{align*}
\end{small}
where $\mathbf{h} = \left[ h(\mathbf{x}_1,\mathbf{\bm \alpha}); h(\mathbf{x}_2,\mathbf{\bm \alpha}); \cdots; h(\mathbf{x}_n,\mathbf{\bm \alpha}) \right]$ 
and $\mathbf{t}=\text{sign}(\mathbf{K} {\bm \alpha})$.
Via setting the gradient to be \textbf{0} and considering that $\mathbf{K}$ is invertible, we can estimate $\lambda$ using Eqn.~\ref{fianl_est} with  
$\mathbf{a} = \mathbf{t}$ and $\mathbf{b} = \mathbf{h} - \mathbf{y}$.

\myparatight{Kernel SVM with regular hinge loss (KSVM-RHL)}
The objective function of KSVM-RHL  is:
%\begin{small}
%\begin{align*}
%%\label{kernel_bsvc_prime}
%\mathcal{L}_{KSVM}(\lambda, \mathbf{w^\prime})  = \lambda \sum_{i=1}^n L_{HL}(y_j, \langle \mathbf{w^\prime}, \phi(\mathbf{x}_j) \rangle) + \frac{1}{2} \| \mathbf{w^\prime} \|_2^2. 
%\end{align*}
%\end{small}
%Using $\mathbf{w}^\prime = \Phi(\mathbf{X})^\lambda \bm{\alpha}$, we have its dual form
\begin{small}
\begin{align}
\label{kernel_bsvc_dual}
\begin{split}
\mathcal{L}(\bm{\alpha}) = \sum_{i=1}^n L(\mathbf{x}_i, y_i,  \bm{\alpha}) + \lambda \bm{\alpha}^T \mathbf{K} \bm{\alpha},
\end{split}
\end{align}
\end{small}
where $L(\mathbf{x}_i, y_i,  \bm{\alpha}) = \max(0, 1 - y_i  \bm{\alpha}^T \mathbf{k}_i )$, where $\mathbf{k}_i$ is the $i$th column of the gram matrix $\mathbf{K}$.
Following the same methodology we used for SVM-RHL,  
we estimate $\lambda$ using Eqn.~\ref{fianl_est} with $\mathbf{a} = 2 \mathbf{K} \bm{\alpha}$ and $\mathbf{b} = \sum_{i=1}^n -y_i \mathbf{k}_i \mathbf{1}_{y_i  \bm{\alpha}^T \mathbf{k}_i < 1}$. 

%we estimate $\lambda$ for each $\alpha_i$ as 
%\begin{footnotesize}
%\begin{align}
%\label{kernel_bsvc_rhl_soln}
%\hat{\lambda}^{(i)}_{KSVM-RHL} = \frac{\mathbf{k}^i \bm{\alpha}}{\sum\limits_{j, y_j \langle \bm{\alpha}, \mathbf{k}_j \rangle <1} y_j k_{j,i}}.
%\end{align} 
%\end{footnotesize}
%%\vspace{-5mm}

\myparatight{Kernel SVM with square hinge loss (KSVM-SHL)}
The objective function of KSVM-SHL  is:
%\begin{small}
%\begin{align*}
%%\label{kernel_bsvc_prime}
%\mathcal{L}_{KSVM}(\lambda, \mathbf{w^\prime})  = \lambda \sum_{i=1}^n L_{HL}(y_j, \langle \mathbf{w^\prime}, \phi(\mathbf{x}_j) \rangle) + \frac{1}{2} \| \mathbf{w^\prime} \|_2^2. 
%\end{align*}
%\end{small}
%Using $\mathbf{w}^\prime = \Phi(\mathbf{X})^\lambda \bm{\alpha}$, we have its dual form
\begin{small}
\begin{align}
\label{kernel_bsvc_dual}
\begin{split}
\mathcal{L}(\bm{\alpha}) = \sum_{i=1}^n L(\mathbf{x}_i, y_i,  \bm{\alpha}) + \lambda \bm{\alpha}^T \mathbf{K} \bm{\alpha},
\end{split}
\end{align}
\end{small}
where $L(\mathbf{x}_i, y_i,  \bm{\alpha}) = \max(0, 1 - y_i  \bm{\alpha}^T \mathbf{k}_i )^2$.
Following the same methodology we used for SVM-SHL,  
we estimate $\lambda$ using Eqn.~\ref{fianl_est} with $\mathbf{a} = \mathbf{K} \bm{\alpha}$ and $\mathbf{b} = \sum_{i=1}^n -y_i \mathbf{k}_i (1-y_i  \bm{\alpha}^T \mathbf{k}_i) \mathbf{1}_{y_i  \bm{\alpha}^T \mathbf{k}_i \leq 1}$.

%\myparatight{SHL} $L_{SHL}(y_j, \langle \bm{\alpha}, \mathbf{k}_j \rangle) = \max(0, 1 - y_j \langle \bm{\alpha}, \mathbf{k}_j \rangle )^2$. We take the derivative of $\mathcal{L}(\bm{\alpha})$ for $\bm{\alpha}$ and set it to be $\mathbf{0}$. Then, for KSVM-SHL, we have
%$\mathbf{a} =\mathbf{K} \bm{\alpha}$ and $\mathbf{b} = \sum_{j=1}^n -2 y_j \mathbf{k}_j (1 - y_j \langle \bm{\alpha}, \mathbf{k}_j \rangle) \mathbf{1}_{y_j \langle \bm{\alpha}, \mathbf{k}_j \rangle \leq 1}$.
%
%
%
%\myparatight{Kernel SVM with regular hinge loss (KSVM-RHL)}
%
%\myparatight{Kernel SVM with square hinge loss (KSVM-SHL)}
%

\section{More than One Hyperparameter}
\label{app:enet}
We use a popular regression algorithm called \emph{Elastic Net (ENet)}~\cite{} as an example to illustrate how we can apply attacks 
to learning algorithms with more than one hyperparameter. 
The objective function of ENet is: 
%\subsubsection{Elastic Net: More general case}
\begin{small}
\begin{align}
\label{enet}
\mathcal{L}(\mathbf{w}) = \| \mathbf{y}-\mathbf{X}^T\mathbf{w} \|_2^2 + \lambda_1 \| \mathbf{w} \|_1 + \lambda_2 \| \mathbf{w} \|_2^2,
\end{align}
\end{small}
where the loss function is least square and regularization term is the combination of $L_2$ regularization and $L_1$ regularization. 
We compute the gradient as follows: 
\begin{small}
\begin{align*}
%\label{lasso_grad}
\frac{\partial \mathcal{L}(\mathbf{w})}{\partial \mathbf{w}} = -2 \mathbf{X y} + 2 \mathbf{X}\mathbf{X}^T\mathbf{w} + \lambda_1 \mathbf{s} + 2 \lambda_2 \mathbf{w} \odot |\mathbf{s}|,
%2  \mathbf{x}_i^T \mathbf{x}_i \mathbf{w}  - 2 \left\langle \mathbf{x}_i, \mathbf{r}_i \right\rangle + \lambda \partial \|\mathbf{w}\|_1 |_{w_i},
\end{align*}
\end{small}
where $\mathbf{s}$ is defined in Eqn.~\ref{vectors} and the vector $\mathbf{w} \odot |\mathbf{s}|=[w_1|s_1|; w_2|s_2|; \cdots;w_m|s_m|]$. 
Similar to LASSO, we do not use the model parameters that are 0 to estimate the hyperparameters. Via setting the gradient to $\mathbf{0}$ and using the linear least square to solve the underdetermined system, we have:
\begin{small}
\begin{align}
\hat{\bm{\lambda}} = -\left( \mathbf{A}^T \mathbf{A} \right)^{-1} \mathbf{A}^T \mathbf{b},
\end{align}
\end{small}
where $\hat{\bm{\lambda}}=[\hat{\lambda_1};\hat{\lambda_2}]$,  $\mathbf{A}=[\mathbf{s}; 2\mathbf{w} \odot |\mathbf{s}|]$, and $\mathbf{b}=-2 \mathbf{X y} + 2 \mathbf{X}\mathbf{X}^T\mathbf{w}$.

Figure~\ref{} shows the attack and defense results for ENet on the dataset XX. XXXX

\section{**** Theoretical  Analysis***}

We unformally define the sensitive of $\hat{\lambda}$ with respect to $\mathbf{w}$
as $ \frac{\Delta \hat{\lambda}}{\Delta \mathbf{w}}$.  

For RR,
\begin{small}
\begin{align*}
\hat{\lambda}_{RR} = \frac{\mathbf{w}^T (\mathbf{Xy} - \mathbf{X}\mathbf{X}^T \mathbf{w})}{\mathbf{w}^T \mathbf{w}}. 
\end{align*}
\end{small}

The variant of $\hat{\lambda}_{RR}$ with respect to the variant of $\mathbf{w}$ is 
\begin{small}
\begin{align*}
& \Big| \Delta \hat{\lambda}_{RR} \Big| = \Big| \hat{\lambda}_{RR}(\mathbf{w} + \Delta \mathbf{w}) - \hat{\lambda}_{RR}(\mathbf{w}) \Big| \\
& = \Big| \frac{{(\mathbf{w} + \Delta \mathbf{w})}^T (\mathbf{Xy} - \mathbf{X}\mathbf{X}^T (\mathbf{w}+\Delta \mathbf{w}))}{{(\mathbf{w}+\Delta \mathbf{w})}^T (\mathbf{w}+\Delta \mathbf{w})} - \frac{\mathbf{w}^T (\mathbf{Xy} - \mathbf{X}\mathbf{X}^T \mathbf{w})}{\mathbf{w}^T \mathbf{w}} \Big| \\
& = \Big| \frac{\Delta \mathbf{w}^T (\mathbf{Xy} - 2 \mathbf{X} \mathbf{X}^T \mathbf{w}) - \Delta \mathbf{w}^T \mathbf{X} \mathbf{X}^T \Delta \mathbf{w}}{\mathbf{w}^T \mathbf{w}} \Big| \\
& \approx \Big| \frac{\Delta \mathbf{w}^T}{\|\mathbf{w}\|_2^2} \mathbf{X} (\mathbf{y}- 2 \mathbf{X}^T \mathbf{w}) \Big|,
\end{align*}
\end{small}
where in the second and third equations, we use $\mathbf{w} + \Delta \mathbf{w} = \mathbf{w}$ , and $\Delta \mathbf{w}^T \mathbf{X} \mathbf{X}^T \Delta \mathbf{w} = 0$ for sufficient small $\Delta \mathbf{w}$.
Therefore $ \frac{\Delta \hat{\lambda}_{RR}}{\Delta \mathbf{w}} = O(\frac{1}{\|\mathbf{w}\|_2^2})$.

For LASSO,
\begin{small}
\begin{align*}
\hat{\lambda}_{LASSO} = \frac{2 \text{sign}(\mathbf{w})^T (\mathbf{Xy} - \mathbf{X} \mathbf{X}^T \mathbf{w})}{\text{sign}(\mathbf{w})^T \text{sign}(\mathbf{w})}.
\end{align*}
\end{small} 

The variant of $\hat{\lambda}_{LASSO}$ with respect to the variant of $\mathbf{w}$ is 
\begin{small}
\begin{align*}
& \Big| \Delta \hat{\lambda}_{LASSO} \Big| = \Big| \hat{\lambda}_{LASSO}(\mathbf{w} + \Delta \mathbf{w}) - \hat{\lambda}_{LASSO}(\mathbf{w}) \Big| \\
& = \Big| \frac{2 \text{sign}(\mathbf{w} + \Delta \mathbf{w})^T (\mathbf{Xy} - \mathbf{X} \mathbf{X}^T (\mathbf{w} + \Delta \mathbf{w}))}{\text{sign}(\mathbf{w} + \Delta \mathbf{w})^T \text{sign}(\mathbf{w} + \Delta \mathbf{w})} - \frac{2 \text{sign}(\mathbf{w})^T (\mathbf{Xy} - \mathbf{X} \mathbf{X}^T \mathbf{w})}{\text{sign}(\mathbf{w})^T \text{sign}(\mathbf{w})} \Big| \\
& = \Big| \frac{\text{sign}(\mathbf{w})^T \mathbf{X} \mathbf{X}^T \Delta \mathbf{w}}{\|\text{sign}(\mathbf{w})\|_2^2} \Big| \\
& = \Big| \frac{\Delta \mathbf{w}^T}{\|\text{sign}(\mathbf{w})\|_2^2} \mathbf{X} \mathbf{X}^T \text{sign}(\mathbf{w}) \Big|,
\end{align*}
\end{small}
where in the third equation, we use $\text{sign}(\mathbf{w} + \Delta \mathbf{w}) = \text{sign}(\mathbf{w})$.
Therefore $ \frac{\Delta \hat{\lambda}_{LASSO}}{\Delta \mathbf{w}} = O(\frac{1}{\|\text{sign}(\mathbf{w})\|_2^2})$.

For L2-LR,
\begin{small}
\begin{align*}
\hat{\lambda}_{L2-LR} = \frac{\mathbf{w}^T \mathbf{X} (\mathbf{y} - \mathbf{h}_{\mathbf{w}}(\mathbf{X}))}{\mathbf{w}^T \mathbf{w}}. 
\end{align*}
\end{small}

The variant of $\hat{\lambda}_{L2-LR}$ with respect to the variant of $\mathbf{w}$ is 
\begin{small}
\begin{align*}
& \Big| \Delta \hat{\lambda}_{L2-LR} \Big|  = \Big| \hat{\lambda}_{L2-LR}(\mathbf{w} + \Delta \mathbf{w}) - \hat{\lambda}_{L2-LR}(\mathbf{w}) \Big| \\ 
& = \Big| \frac{(\mathbf{w}+ \Delta \mathbf{w})^T (\mathbf{y} - \mathbf{h}_{\mathbf{w}+\Delta \mathbf{w}}(\mathbf{X}))}{(\mathbf{w} + \Delta \mathbf{w})^T (\mathbf{w} + \Delta \mathbf{w})} -  \frac{\mathbf{w}^T \mathbf{X} (\mathbf{y} - \mathbf{h}_{\mathbf{w}}(\mathbf{X}))}{\mathbf{w}^T \mathbf{w}} \Big| \\
& = \Big| \frac{\Delta \mathbf{w}^T \mathbf{X}(\mathbf{y} - \mathbf{h}_{\mathbf{w} + \Delta \mathbf{w}}(\mathbf{X})) - \mathbf{w}^T \mathbf{X} (\mathbf{h}_{\mathbf{w} + \Delta \mathbf{w}}(\mathbf{X}) - \mathbf{h}_{\mathbf{w}}(\mathbf{X}))}{\mathbf{w}^T \mathbf{w}} \Big|  \\
& \approx \Big| \frac{\Delta \mathbf{w}^T}{\|\mathbf{w}\|_2^2} \mathbf{X}(\mathbf{y} - \mathbf{h}_{\mathbf{w}}(\mathbf{X})) \Big|,
\end{align*}
\end{small}
where in the third and equation equation, we use $\mathbf{w} + \Delta \mathbf{w} = \mathbf{w}$ , and $\mathbf{h}_{\mathbf{w} + \Delta \mathbf{w}}(\mathbf{X}) = \mathbf{h}_{\mathbf{w}}(\mathbf{X})$ for sufficient small $\Delta \mathbf{w}$. 
Therefore $ \frac{\Delta \hat{\lambda}_{L2-LR}}{\Delta \mathbf{w}} = O(\frac{1}{\|\mathbf{w}\|_2^2})$.

For L1-LR,
\begin{small}
\begin{align*}
\hat{\lambda}_{L1-LR} = \frac{\text{sign}(\mathbf{w})^T \mathbf{X} (\mathbf{y} - \mathbf{h}_{\mathbf{w}}(\mathbf{X}))}{\text{sign}(\mathbf{w})^T \text{sign}(\mathbf{w})}. 
\end{align*}
\end{small} 

The variant of $\hat{\lambda}_{L1-LR}$ with respect to the variant of $\mathbf{w}$ is
\begin{small}
\begin{align*}
& \Big| \Delta \hat{\lambda}_{L1-LR} \Big|  = \Big| \hat{\lambda}_{L1-LR}(\mathbf{w} + \Delta \mathbf{w}) - \hat{\lambda}_{L1-LR}(\mathbf{w}) \Big| \\ 
& = \Big| \frac{\text{sign}(\mathbf{w} + \Delta \mathbf{w})^T \mathbf{X} (\mathbf{y} - \mathbf{h}_{\mathbf{w} + \Delta \mathbf{w}}(\mathbf{X}))}{\text{sign}(\mathbf{w} + \Delta \mathbf{w})^T \text{sign}(\mathbf{w} + \Delta \mathbf{w})} - \frac{\text{sign}(\mathbf{w})^T \mathbf{X} (\mathbf{y} - \mathbf{h}_{\mathbf{w}}(\mathbf{X}))}{\text{sign}(\mathbf{w})^T \text{sign}(\mathbf{w})} \Big| \\
& = \Big| \frac{\text{sign}(\mathbf{w})^T}{{\| \text{sign}(\mathbf{w})\|_2^2}} \mathbf{X}(\mathbf{h}_{\mathbf{w}+\Delta \mathbf{w}}(\mathbf{X}) - \mathbf{h}_{\mathbf{w}}(\mathbf{X})) \Big|,
\end{align*}
\end{small}
where we use $\text{sign}(\mathbf{w} + \Delta \mathbf{w}) = \text{sign}(\mathbf{w})$.
Therefore $ \frac{\Delta \hat{\lambda}_{L1-LR}}{\Delta \mathbf{w}} = O(\frac{1}{\|\text{sign}(\mathbf{w})\|_2^2})$.

For SVM-RHL,
\begin{small}
\begin{align*}
{\hat{\lambda}_{SVM-RHL}} = \frac{\mathbf{w}^T \Big( \sum_{j=1}^n -y_j \mathbf{x}_j \mathbf{1}_{y_j \langle \mathbf{w}, \mathbf{x}_j \rangle < 1} \Big)}{\mathbf{w}^T \mathbf{w}}. 
\end{align*}
\end{small}

The variant of ${\hat{\lambda}_{SVM-RHL}}$ with respect to the variant of $\mathbf{w}$ is
\begin{small}
\begin{align*}
& \Big| \Delta \hat{\lambda}_{SVM-RHL} \Big| = \Big| \hat{\lambda}_{SVM-RHL}(\mathbf{w} + \Delta \mathbf{w}) - \hat{\lambda}_{SVM-RHL}(\mathbf{w} \Big|\\
& = \Big| \frac{(\mathbf{w} + \Delta \mathbf{w})^T \Big( \sum_{j=1}^n -y_j \mathbf{x}_j \mathbf{1}_{y_j \langle (\mathbf{w} + \Delta \mathbf{w}), \mathbf{x}_j \rangle < 1} \Big)}{(\mathbf{w} + \Delta \mathbf{w})^T (\mathbf{w} + \Delta \mathbf{w})} - \frac{\mathbf{w}^T \Big( \sum_{j=1}^n -y_j \mathbf{x}_j \mathbf{1}_{y_j \langle \mathbf{w}, \mathbf{x}_j \rangle < 1} \Big)}{\mathbf{w}^T \mathbf{w}} \Big| \\
& = \Big| \frac{\Delta \mathbf{w}^T} {\| \mathbf{w}\|_2^2} \Big( \sum_{j=1}^n -y_j \mathbf{x}_j \mathbf{1}_{y_j \langle \mathbf{w}, \mathbf{x}_j \rangle < 1} \Big) \Big|,
\end{align*}
\end{small}
where we assume $\mathbf{w} + \Delta \mathbf{w} = \mathbf{w}$ and $y_j \langle (\mathbf{w} + \Delta \mathbf{w}), \mathbf{x}_j \rangle < 1 $ when $y_j \langle \mathbf{w}, \mathbf{x}_j \rangle < 1$ for sufficient small $\Delta w$.
Therefore $ \frac{\Delta \hat{\lambda}_{SVM-RHL}}{\Delta \mathbf{w}} = O(\frac{1}{\|\mathbf{w}\|_2^2})$.

For SVM-SHL,
\begin{small}
\begin{align*}
{\hat{\lambda}_{SVM-SHL}} = \frac{\mathbf{w}^T \Big( \sum_{j=1}^n - 2y_j \mathbf{x}_j (1- y_j \langle \mathbf{w}, \mathbf{x}_j \rangle) \mathbf{1}_{y_j \langle \mathbf{w}, \mathbf{x}_j \rangle <= 1} \Big)}{\mathbf{w}^T \mathbf{w}}. 
\end{align*}
\end{small}

The variant of ${\hat{\lambda}_{SVM-SHL}}$ with respect to the variant of $\mathbf{w}$ is
\begin{small}
\begin{align*}
& \Big| \Delta \hat{\lambda}_{SVM-SHL} \Big| = \Big| \hat{\lambda}_{SVM-SHL}(\mathbf{w} + \Delta \mathbf{w}) - \hat{\lambda}_{SVM-SHL}(\mathbf{w} \Big|\\
& = \Big| \frac{(\mathbf{w} + \Delta \mathbf{w})^T \Big( \sum_{j=1}^n -2 y_j \mathbf{x}_j (1- y_j \langle \mathbf{w} + \Delta \mathbf{w}, \mathbf{x}_j \rangle) \mathbf{1}_{y_j \langle (\mathbf{w} + \Delta \mathbf{w}), \mathbf{x}_j \rangle < 1} \Big)}{(\mathbf{w} + \Delta \mathbf{w})^T (\mathbf{w} + \Delta \mathbf{w})} \\
&	\qquad - \frac{\mathbf{w}^T \Big( \sum_{j=1}^n - 2 y_j \mathbf{x}_j (1- y_j \langle \mathbf{w}, \mathbf{x}_j \rangle) \mathbf{1}_{y_j \langle \mathbf{w}, \mathbf{x}_j \rangle < 1} \Big)}{\mathbf{w}^T \mathbf{w}} \Big| \\
& = \Big| \frac{\Delta \mathbf{w}^T} {\| \mathbf{w}\|_2^2} \Big( \sum_{j=1}^n -2 y_j (1- y_j \langle \mathbf{w}, \mathbf{x}_j \rangle) \mathbf{x}_j \mathbf{1}_{y_j \langle \mathbf{w}, \mathbf{x}_j \rangle < 1} \Big) \Big|,
\end{align*}
\end{small}
where we use the same assumption as SVM-RHL.
Therefore $ \frac{\Delta \hat{\lambda}_{SVM-SHL}}{\Delta \mathbf{w}} = O(\frac{1}{\|\mathbf{w}\|_2^2})$.

More accurate comparison of SVM-RHL and SVM-SHL, we notice that their difference is between the factor $2\big(1 - y_j \big( \langle \mathbf{w}, \mathbf{x}_j \rangle \big) \big)$ and 1. By leveraging the property of SVM, we know that when the training set $\mathbf{X}$ can be (approximately) linearly separable, then $y_j \langle \mathbf{w}, \mathbf{x}_j \rangle $ is close to 1, i.e., $1-y_j \langle \mathbf{w}, \mathbf{x}_j \rangle $ is a small positive number. 
Therefore, $ 1- y_j \big( \langle \mathbf{w}, \mathbf{x}_j \rangle \big) \big) < \frac{1}{2}$, and thus SVM-SHL is more sensitive than SVM-RHL.

\section{Hyperparameter Sensitivity Analysis}

\subsection{Proof of Claim~\ref{theorem_reg}}
\label{app:theorem_reg}

For RR, its hyperparameter sensitivity is defined as 
\begin{small}
\begin{align*}
\begin{split}
& \Bigg| \frac{\Delta \hat{\lambda}_{RR}^{(i)}}{\Delta w_i} \Bigg| = \Bigg|\frac{\hat{\lambda}_{RR}^{(i)}(w_i + \Delta w_i) - \hat{\lambda}_{RR}^{(i)}(w_i)}{\Delta w_i}\Bigg| \\
& = \Bigg|\frac{1}{\Delta w_i} \bigg( \frac{\langle \mathbf{x}_i, \mathbf{r}_i \rangle}{w_i + \Delta w_i} - \frac{\langle \mathbf{x}_i, \mathbf{r}_i \rangle}{w_i} \bigg)\Bigg| = \Bigg|\frac{1}{(w_i + \Delta w_i) w_i} \langle \mathbf{x}_i, \mathbf{r}_i \rangle \Bigg|.
\end{split}
\end{align*}
\end{small}
For LASSO, 
\begin{small}
\begin{align*}
\Bigg| \frac{\Delta \hat{\lambda}_{LASSO}^{(i)}}{\Delta w_i} \Bigg| = \Bigg| \frac{-2 \langle \mathbf{x}_i, \mathbf{x}_i \rangle (w_i + \Delta w_i) + 2 \langle \mathbf{x}_i, \mathbf{x}_i \rangle w_i }{\Delta w_i} \Bigg| = \big| 2 \langle \mathbf{x}_i, \mathbf{x}_i \rangle \big|.
\end{align*}
\end{small}
%Similarly, $\frac{\Delta \hat{\lambda}_{LASSO}^{(i)}}{\Delta w_i} = 2 \langle \mathbf{x}_i, \mathbf{x}_i \rangle $ if $w_i < 0$.
Note that the sensitivity of RR depends on both the optimal $w_i$ and the variation $\Delta w_i$; While for LASSO, it is independent of both $w_i$ and $\Delta w_i$. As a result, $\hat{\lambda}_{LASSO}^{(i)}$ of LASSO has a minor (and almost constant) change if the length of $\mathbf{x}_i$ is small (which can be obtained through preprocessing); However, $\hat{\lambda}_{RR}^{(i)}$ of RR can change largely once the absolute value of $w_i$ is much smaller than 1, or/and the absolute value of $\Delta w_i$ is near to $w_i$ (Notice that $\Delta w_i$ and $w_i$ always have the opposite sign in our experiments, and thus if $|\Delta w_i| \rightarrow |w_i|, w_i + \Delta w_i \rightarrow 0$). 
%, which is often the case. For instance, $l_2$ norm of $\mathbf{w}$ is required to be less than or equal 1, i.e., $\| \mathbf{w} \|_2 \leq 1$.  

For ENet, since it incorporates both $L_2$ and $L_1$ regularizations, the sensitivity of $\hat{\lambda}_2^{(i)}$ and $\hat{\lambda}_1^{(i)}$ share the same property with $\hat{\lambda}_{RR}^{(i)}$ and $\hat{\lambda}_{LASSO}^{(i)}$, respectively. % Specifically,

For KRR, the sensitivity is 
\begin{small}
\begin{align*}
%\label{KernelRidge_sensi}
\begin{split}
\Bigg| \frac{\Delta \hat{\lambda}_{KRR}^{(j)}}{\Delta \alpha_j} \Bigg| & = \Bigg| \frac{1}{\Delta \alpha_j} \bigg( \frac{y_j}{\alpha_j + \Delta \alpha_j} - \frac{y_j}{\alpha_j} \bigg) \Bigg| = \Bigg| -\frac{1}{(\alpha_j + \Delta \alpha_j) \alpha_j} y_j \Bigg|,   
\end{split}
\end{align*}
\end{small}
which has a similar form with RR. Thus, the far smaller $\alpha_j$ is than 1, or the much closer $\Delta \alpha_j$ is to $\alpha_j$, the more sensitive KRR is.  

%\vspace{-5mm}
\subsection{Proof of Claim~\ref{theorem_lr}}
\label{app:theorem_lr}

First, we consider $L_2$-BLR and $L_1$-BLR.

For $L_2$-BLR, 
$\hat{\lambda}_{L_2-BLR}^{(i)} (w_i + \Delta w_i) = - \frac{\langle \mathbf{x}_i, h_{\mathbf{w}+\Delta w_i}(\mathbf{X}) - \mathbf{y} \rangle}{ 2 (w_i + \Delta w_i)}$, 
where $h_{\mathbf{w}+\Delta w_i}(\mathbf{X}) = \left[ h_{\mathbf{w}+\Delta w_i}(\mathbf{x}^1_T), \cdots, h_{\mathbf{w}+\Delta w_i}(\mathbf{x}^n_T) \right]^T $ and $h_{\mathbf{w}+\Delta w_i} (\mathbf{x}^i_T) = \frac{1}{1 + \exp(\sum_{j \neq i} w_j x_{i,j}) + (w_i + \Delta w_i) x_{i,i}}$ (One should notice that the notation $\mathbf{w}+\Delta w_i$ here is not so ``formal", as $\Delta w_i$ is not added to all elements of $\mathbf{w}$, but to its $i$-th entry. We use such notation for simplicity).
Therefore, 
\begin{small}
\begin{align*}
%\label{L2_BLR_sensi}
\begin{split}
& \Bigg| \frac{\Delta \hat{\lambda}_{L_2-BLR}^{(i)}}{\Delta w_i} \Bigg| = \Bigg| \frac{\hat{\lambda}_{L_2-BLR}^{(i)} (w_i + \Delta w_i) - \hat{\lambda}_{L_2-BLR}^{(i)} (w_i)}{\Delta w_i} \Bigg| \\
& = \Bigg| \frac{\langle \mathbf{x}_i, h_{\mathbf{w}+\Delta w_i}(\mathbf{X}) - \mathbf{y} \rangle}{\Delta w_i} \bigg( -\frac{1}{2(w_i + \Delta w_i)}  + \frac{\langle \mathbf{x}_i, h_{\mathbf{w}}(\mathbf{X}) - \mathbf{y} \rangle}{2 w_i}  \bigg) \Bigg| \\
& = \Bigg| \frac{\langle \mathbf{x}_i, h_{\mathbf{w}+\Delta w_i}(\mathbf{X}) - \mathbf{y} \rangle}{\Delta w_i} \bigg( - \frac{1}{2(w_i + \Delta w_i)}  + \frac{\langle \mathbf{x}_i, h_{\mathbf{w}}(\mathbf{X}) - \mathbf{y} \rangle}{2(w_i + \Delta w_i)}  \bigg) \\ 
& \quad + \frac{1}{\Delta w_i} \bigg( - \frac{\langle \mathbf{x}_i, h_{\mathbf{w}}(\mathbf{X}) - y \rangle}{2(w_i + \Delta w_i)}  + \frac{\langle \mathbf{x}_i, h_{\mathbf{w}}(\mathbf{X}) - \mathbf{y} \rangle}{2 w_i}  \bigg) \Bigg| \\
& = \Bigg| - \frac{\langle \mathbf{x}_i, h_{\mathbf{w}+\Delta w_i}(\mathbf{X}) - h_{\mathbf{w}}(\mathbf{X}) \rangle}{2(w_i + \Delta w_i) \Delta w_i} + \frac{\langle \mathbf{x}_i, h_{\mathbf{w}}(\mathbf{X}) - \mathbf{y} \rangle}{2 w_i (w_i + \Delta w_i)}  \Bigg|. 
\end{split}
\end{align*}
\end{small}

For $L_1$-BLR, 
\begin{small}
\begin{align*}
%\label{L1_BLR_sensi}
\begin{split}
\Bigg| \frac{\Delta \hat{\lambda}_{L_1-BLR}^{(i)}}{\Delta w_i} \Bigg| & = \Bigg| \frac{1}{\Delta w_i} \big( \langle \mathbf{x}_i, h_{\mathbf{w} + \Delta w_i}(\mathbf{X}) - \mathbf{y} \rangle - \langle \mathbf{x}_i, h_{\mathbf{w}}(\mathbf{X}) - \mathbf{y} \rangle \big) \Bigg| \\
& = \Bigg| \frac{1}{\Delta w_i} \langle \mathbf{x}_i, h_{\mathbf{w} + \Delta w_i}(\mathbf{X}) - h_{\mathbf{w}}(\mathbf{X}) \rangle \Bigg|.
\end{split}
\end{align*}
\end{small}
%Similarly, if $w_i <0$, $\frac{\Delta \hat{\lambda}_{L_1-BLR}^{(i)}}{\Delta w_i} = - \frac{1}{\Delta w_i} \langle \mathbf{x}_i, h_{\mathbf{w} + \Delta w_i}(\mathbf{X}) - h_{\mathbf{w}}(\mathbf{X}) \rangle $.
%Comparing Eqn~\ref{L2_BLR_sensi} with Eqn~\ref{L1_BLR_sensi} 
Comparing above two equations and reusing aforementioned analysis, we observe that once $|w_i|$ is much smaller than 1 or $\Delta w_i$ is comparable with $w_i$, then $L_2$-BLR is more sensitive than $L_1$-BLR. %in terms of the variation of $w_i$. 

Then, we consider $L_2$-BKLR and $L_1$-BKLR.

For $L_2$-BKLR,
\begin{small}
\begin{align*}
\begin{split}
& \Bigg| \frac{\Delta \hat{\lambda}_{L_2-BKLR}^{(j)}}{\Delta \alpha_j} \Bigg| = \Bigg| \frac{1}{\Delta \alpha_j} \bigg( \frac{y_j - h_{\bm{\alpha} + \Delta \alpha_j}(\mathbf{k}_j)}{2(\alpha_j + \Delta \alpha_j)} - \frac{y_j - h_{\bm{\alpha}} (\mathbf{k}_j)}{2 \alpha_j} \bigg) \Bigg| \\
& = \Bigg| - \frac{h_{\bm{\alpha}+\Delta \alpha_j}(\mathbf{k}_j) - h_{\bm{\alpha}}(\mathbf{k}_j)}{2(\alpha_j + \Delta \alpha_j) \Delta \alpha_j} + \frac{h_{\bm{\alpha}}(\mathbf{k}_j) - y_j}{2(\alpha_j + \Delta \alpha_j) \alpha_j} \Bigg|,
\end{split}
\end{align*}
\end{small}
where $h_{\bm{\alpha}+\Delta \alpha_j} (\mathbf{k}_j) = \frac{1}{1+ \exp(\langle \bm{\alpha}, \mathbf{k}_j \rangle + \Delta \alpha_j k_{j,j})}$.

For $L_1$-BKLR, %if $\mathbf{k}^j \bm{\alpha} < 0$,
\begin{small}
\begin{align*}
\Bigg| \frac{\Delta \hat{\lambda}_{L_1-BKLR}^{(j)}}{\Delta \alpha_j} \Bigg| = \Bigg| \frac{1}{\Delta \alpha_j} \big( h_{\bm{\alpha}+\Delta \alpha_j}(\mathbf{k}_j) - h_{\bm{\alpha}}(\mathbf{k}_j) \big) \Bigg|.
\end{align*}
\end{small}
%and $\frac{\Delta \hat{\lambda}_{L_1-BKLR}^{(j)}}{\Delta \alpha_j} = \frac{1}{\Delta \alpha_j} \big( - h_{\bm{\alpha}+\Delta \alpha_j}(\mathbf{k}_j) + h_{\bm{\alpha}}(\mathbf{k}_j) \big)$ if $\mathbf{k}^j \bm{\alpha} > 0$. 

We have similar sensitivity analysis of $L_2$-BKLR and $L_1$-BKLR as that of $L_2$-BLR and $L_1$-BLR. That is, if $|\alpha_j|$ is much smaller than 1 or $\Delta \alpha_j$ is comprable with $\alpha_j$, then L2-BKLR is more sensitive than L1-BKLR.

%\vspace{-5mm}
\subsection{Proof of Claim~\ref{theorem_svc}}
\label{app:theorem_svc}

First, we consider BLSVC-RHL and BLSVC-SHL.

For BLSVC-RHL,
\begin{footnotesize} 
\begin{align*}
%\label{BLSVC_RHL_sensi}
\begin{split}
\Bigg| \frac{\Delta \hat{C}_{BLSVC-RHL}^{(i)}}{\Delta w_i} \Bigg| & = \Bigg| \frac{1}{\Delta w_i} \Bigg( \frac{w_i + \Delta w_i}{\sum\limits_{j, y_j \big( \langle \mathbf{w}, \mathbf{x}_T^j \rangle + \Delta w_i x_{j,i} \big) < 1} y_j x_{j,i}} - \frac{w_i}{\sum\limits_{j, y_j \langle \mathbf{w}, \mathbf{x}_T^j \rangle <1} y_j x_{j,i} } \Bigg) \Bigg| \\
& \approx \frac{1}{\sum\limits_{j, y_j \big( \langle \mathbf{w}, \mathbf{x}_T^j \rangle + \Delta w_i x_{j,i} \big) < 1} y_j x_{j,i}}, 
\end{split}
\end{align*}
\end{footnotesize}
where we assume that by adding $\Delta w_i$, the sign of $1- y_j \big( \langle \mathbf{w}, \mathbf{x}_T^j \rangle + \Delta w_i x_{i,i} \big) \big)$ is still positive (It often satisfies in practice). 

For BLSVC-SHL, 
\begin{footnotesize}
\begin{align*}
%\label{BLSVC_SHL_sensi}
\begin{split}
& \Bigg| \frac{\Delta \hat{C}_{BLSVC-SHL}^{(i)}}{\Delta w_i} \Bigg| = \\
&  \Bigg| \frac{1}{\Delta w_i} \Bigg( \frac{w_i + \Delta w_i}{\sum\limits_{j, y_j \big( \langle \mathbf{w}, \mathbf{x}_T^j \rangle + \Delta w_i x_{j,i} \big) < 1} 2 y_j x_{j,i} \big(1 - y_j \big( \langle \mathbf{w}, \mathbf{x}_T^j \rangle + \Delta w_i x_{j,i} \big) \big) } \\
& \quad - \frac{w_i}{\sum\limits_{j, y_j \langle \mathbf{w}, \mathbf{x}_T^j \rangle <1} 2 y_j x_{j,i} \big(1 - y_j \langle \mathbf{w}, \mathbf{x}_T^j \rangle \big) } \Bigg) \Bigg| \\
& \approx \frac{1}{\sum\limits_{j, y_j \big( \langle \mathbf{w}, \mathbf{x}_T^j \rangle + \Delta w_i x_{j,i} \big) < 1} 2 y_j x_{j,i} \big(1 - y_j \big( \langle \mathbf{w}, \mathbf{x}_T^j \rangle + \Delta w_i x_{j,i} \big) \big) }.
\end{split}
\end{align*}
\end{footnotesize}
%Comparing Eqn~\ref{BLSVC_RHL_sensi} and Eqn~\ref{BLSVC_SHL_sensi}, 
Comparing above two equations, we notice that their difference is between the factor $2\big(1 - y_j \big( \langle \mathbf{w}, \mathbf{x}_T^j \rangle + \Delta w_i x_{i,i} \big) \big)$ and 1. By leveraging the property of SVC, we know that when the training set $\mathbf{X}$ can be (approximately) linearly separable, then $y_j \langle \mathbf{w}, \mathbf{x}_T^j \rangle $ is close to 1, i.e., $1-y_j \langle \mathbf{w}, \mathbf{x}_T^j \rangle $ is a small positive number. 
Therefore, 
%by adding $\Delta w_i$ such that the sign of $1- y_j \big( \langle \mathbf{w}, \mathbf{x}_T^j \rangle + \Delta w_i x_{i,i} \big) \big)$ is still positive, 
we conclude that $ 1- y_j \big( \langle \mathbf{w}, \mathbf{x}_T^j \rangle + \Delta w_i x_{i,i} \big) \big) < \frac{1}{2}$, and thus $\hat{C}_{BLSVC-SHL}^{(i)}$ is more sensitive than $\hat{C}_{BLSVC-RHL}^{(i)}$.

Then, we consider BKSVC-RHL and BKSVC-SHL.

For BKSVC-RHL,
\begin{footnotesize} 
\begin{align*}
%\label{BKSVC_RHL_sensi}
\Bigg| \frac{\Delta \hat{C}_{BKSVC-RHL}^{(i)}}{\Delta \alpha_i} \Bigg|  = \Bigg| \frac{1}{\Delta \alpha_i} \Bigg( \frac{\mathbf{k}^i \bm{\alpha} + k_{ii} \Delta \alpha_i}{\sum\limits_{j, y_j (\langle \bm{\alpha}, \mathbf{k}_j \rangle + \Delta \alpha_i k_{i,j}) <1} y_j k_{j,i}} - \frac{\mathbf{k}^i \bm{\alpha}}{\sum\limits_{j, y_j \langle \bm{\alpha}, \mathbf{k}_j \rangle <1} y_j k_{j,i} } \Bigg) \Bigg|.
\end{align*}
\end{footnotesize}

For BKSVC-SHL
\begin{small}
\begin{align*}
%\label{BKSVC_SHL_sensi}
\begin{split}
& \Bigg| \frac{\Delta \hat{C}_{BKSVC-SHL}^{(i)}}{\Delta \alpha_i} \Bigg| = \\
& \Bigg| \frac{1}{\Delta \alpha_i} \Bigg( \frac{\mathbf{k}^i \bm{\alpha} + k_{ii} \Delta \alpha_i}{\sum\limits_{j, y_j (\langle \bm{\alpha}, \mathbf{k}_j \rangle + \Delta \alpha_i k_{i,j}) <1} 2 y_j k_{j,i} \big( 1 - y_j (\langle \bm{\alpha}, \mathbf{k}_j \rangle + \Delta \alpha_i k_{i,j}) \big)} \\
& \quad -  \frac{\mathbf{k}^i \bm{\alpha}}{\sum\limits_{j, y_j \langle \bm{\alpha}, \mathbf{k}_j \rangle <1} 2 y_j k_{j,i} \big( 1 - y_j \langle \bm{\alpha}, \mathbf{k}_j \rangle \big)} \Bigg) \Bigg|.
\end{split}
\end{align*}
\end{small}

Similar results can be obtained, i.e., $\hat{C}_{BKSVC-SHL}^{(i)}$ is more sensitive than $\hat{C}_{BKSVC-RHL}^{(i)}$,  as $1 - y_j (\langle \bm{\alpha}, \mathbf{k}_j \rangle + \Delta \alpha_i k_{i,j}) < \frac{1}{2}$ is often satisfied. 

\begin{figure}[htbp]
\center
\subfloat[M1 vs. M3]{\includegraphics[width=0.23\textwidth]{./src_time/figs/result-CovType-lr-acc-time-m1-m3.pdf}\label{lr_covtype_m1_m3}} 
\subfloat[M2 vs. M3]{\includegraphics[width=0.23\textwidth]{./src_time/figs/result-CovType-lr-acc-time-m2-m3.pdf}\label{lr_covtype_m2_m3}}
\caption{Relative ACC error and speedup of L2-BLR on CovType.}
\label{lr_covtype}
\end{figure}

\begin{figure}[htbp]
\center
\subfloat[M1 vs. M3]{\includegraphics[width=0.23\textwidth]{./src_time/figs/result-CovType-svc-acc-time-m1-m3.pdf}\label{svc_covtype_m1_m3}} 
\subfloat[M2 vs. M3]{\includegraphics[width=0.23\textwidth]{./src_time/figs/result-CovType-svc-acc-time-m2-m3.pdf}\label{svc_covtype_m2_m3}}
\caption{Relative ACC error and speedup of BLSVC-SHL on CovType.}
\label{svc_covtype}
\end{figure}

\begin{figure}[htbp]
\center
\subfloat[L2-BLR]{\includegraphics[width=0.23\textwidth]{./src_time/figs/result-Gaussian-speedup-lr-0.001-error.pdf}\label{lr_speedup}} 
\subfloat[BLSVC-SHL]{\includegraphics[width=0.23\textwidth]{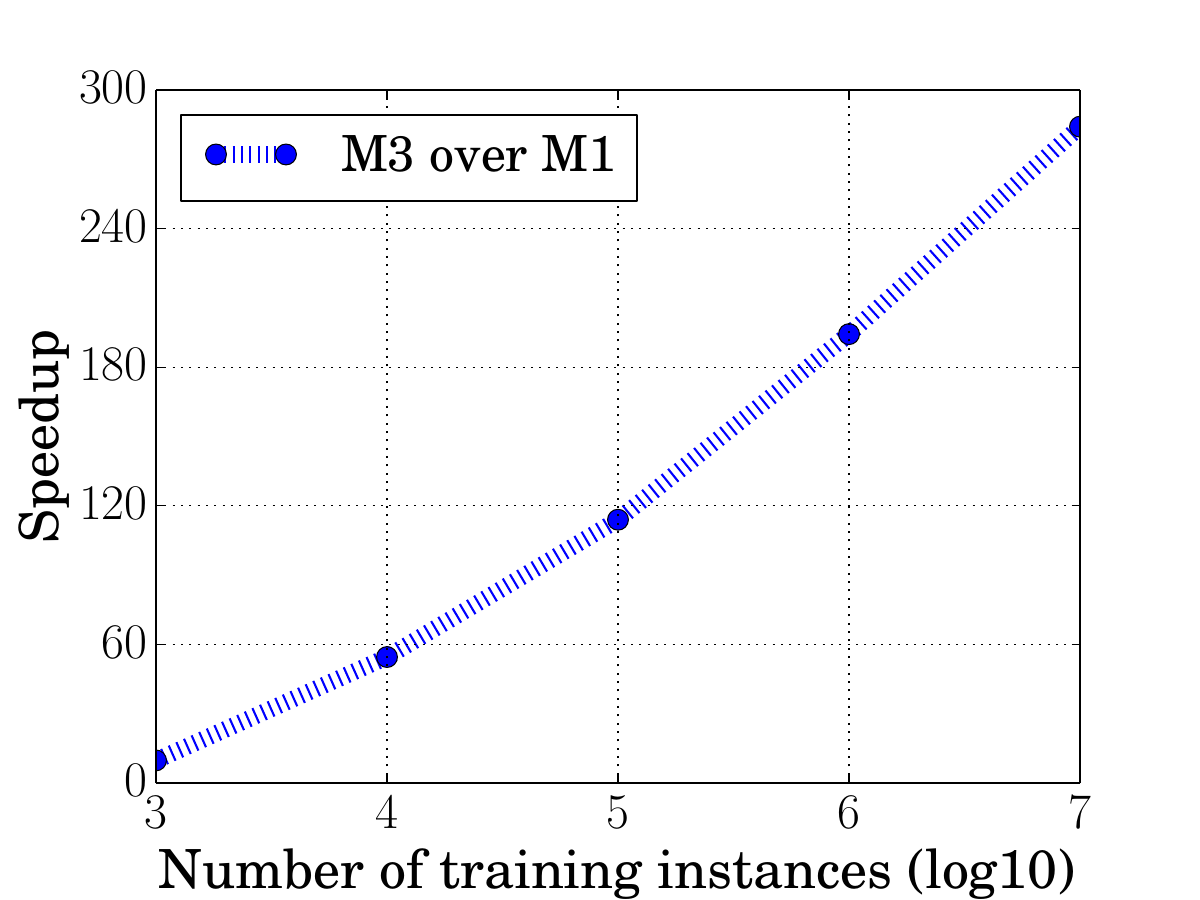}\label{svc_speedup}}
\caption{Speedup of L2-BLR and BLSVC-SHL on synthetic data drawn from Gaussian distribution with Poission noise.}
\label{speedup_gaussian}
\end{figure}

\begin{figure}[htbp]
\center
\subfloat[L2-BLR]{\includegraphics[width=0.23\textwidth]{./src_time/figs/result-CovType-lr-defense-m1-m3.pdf}\label{lr_defense_covtype_m1_m3}} 
\subfloat[BLSVC-SHL]{\includegraphics[width=0.23\textwidth]{./src_time/figs/result-CovType-svc-defense-m1-m3.pdf}\label{svc_defense_covtype_m1_m3}}
\caption{Relative ACC error of L2-BLR and BLSVC-SHL under defense on CovType.}
\label{real_defense_clf_covType}
\end{figure}

\section{Other Attack Results}
\label{app:attack_res}

We show the hyperparameter stealing results of classification models on Ionosphere and Iris in Figure~\ref{clf_res_attack_other} and evaluate real-world scenario on CovType in Figures~\ref{lr_covtype} and~\ref{svc_covtype}. In Figure~\ref{speedup_gaussian}, we also show the speedup of \textbf{M3} with less than 0.1\% $\delta$-ACC error on synthetic data, which are drawn from Gaussian distribution with Poission noise. We observe that as the number of training set increases, the speedup also enhances.  
% \begin{figure}
% \center
% \subfloat[Iris]{\includegraphics[width=0.23\textwidth]{./src_attack/figs/clf/result-clf-lr-iris-new-final.pdf}\label{clf_lr_iris}} 
% \subfloat[Ionosphere]{\includegraphics[width=0.23\textwidth]{./src_attack/figs/clf/result-clf-lr-ionosphere-new-final.pdf}\label{clf_lr_ionosphere}}
% %\subfloat[Madelon]{\includegraphics[width=0.32\textwidth]{./src_attack/figs/clf/result-clf-lr-madelon-new-final.pdf}\label{clf_lr_madelon}} 
% \caption{Hyperparameter stealing results of binary LR-based classification models.}
% \label{clf_blr_res_attack}
% \end{figure}

% \begin{figure}
% \center
% \label{clf_blsvc_res_attack}
% \subfloat[Iris]{\includegraphics[width=0.23\textwidth]{./src_attack/figs/clf/result-clf-svc-iris-new-final.pdf}\label{clf_svc_iris}} 
% \subfloat[Ionosphere]{\includegraphics[width=0.23\textwidth]{./src_attack/figs/clf/result-clf-svc-ionosphere-new-final.pdf}\label{clf_svc_ionosphere}}
% %\subfloat[Madelon]{\includegraphics[width=0.32\textwidth]{./src_attack/figs/clf/result-clf-svc-madelon-new-final.pdf}\label{clf_svc_madelon}} 
% \caption{Hyperparameter stealing results of binary SVC-based classification models.}
% \end{figure}

\begin{figure*}
\center
\subfloat[Ionosphere]{\includegraphics[width=0.32\textwidth]{./src_attack/figs/clf/result-clf-lr-ionosphere-new-final.pdf}\label{clf_lr_ionosphere}} 
\subfloat[Ionosphere]{\includegraphics[width=0.32\textwidth]{./src_attack/figs/clf/result-clf-svc-ionosphere-new-final.pdf}\label{clf_svc_ionosphere}}
\subfloat[Iris]{\includegraphics[width=0.32\textwidth]{./src_attack/figs/clf/result-clf-mlr-iris-new-final.pdf}\label{clf_mlr_ionosphere}}
\caption{Hyperparameter stealing results of classification models on Ionosphere and Iris.}
\label{clf_res_attack_other}
\end{figure*}

\section{Other Defense Results}

We show the hyperparameter defense results of classification models on Ionosphere and Iris in Figure~\ref{clf_res_defense_other} and evaluate real-world scenario on CovType in Figure~\ref{real_defense_clf_covType}.

% \begin{figure}
% \center
% \subfloat[Iris]{\includegraphics[width=0.23\textwidth]{./src_defense/figs/clf/result-clf-lr-iris-new-new.pdf}\label{lr_iris_defense}} 
% \subfloat[Ionosphere]{\includegraphics[width=0.23\textwidth]{./src_defense/figs/clf/result-clf-lr-ionosphere-new-new.pdf}\label{lr_ionosphere_defense}}
% %\subfloat[Madelon]{\includegraphics[width=0.32\textwidth]{./src_defense/figs/clf/result-clf-lr-madelon-new-new.pdf}\label{lr_madelon_defense}} 
% \caption{Hyperparameter defense results of BLR-based methods.}
% \label{clf_lr_res_defense}
% \end{figure}

% \begin{figure}
% \center
% \subfloat[Iris]{\includegraphics[width=0.23\textwidth]{./src_defense/figs/clf/result-clf-svc-iris-new-new.pdf}\label{svc_iris_defense}} 
% \subfloat[Ionosphere]{\includegraphics[width=0.23\textwidth]{./src_defense/figs/clf/result-clf-svc-ionosphere-new-new.pdf}\label{svc_ionosphere_defense}}
% %\subfloat[Madelon]{\includegraphics[width=0.32\textwidth]{./src_defense/figs/clf/result-clf-svc-madelon-new-new.pdf}\label{svc_ionosphere_defense}} 
% \caption{Hyperparameter defense results of SVC-based methods.}
% \label{clf_svc_res_defense}
% \end{figure}

\begin{figure*}
\center
\subfloat[Ionosphere]{\includegraphics[width=0.32\textwidth]{./src_defense/figs/clf/result-clf-lr-ionosphere-new-new.pdf}\label{lr_ionosphere_defense}} 
\subfloat[Ionosphere]{\includegraphics[width=0.32\textwidth]{./src_defense/figs/clf/result-clf-svc-ionosphere-new-new.pdf}\label{svc_ionosphere_defense}}
\subfloat[Iris]{\includegraphics[width=0.32\textwidth]{./src_defense/figs/clf/result-clf-mlr-iris-new-new.pdf}\label{mlr_ionosphere_defense}}
\caption{Hyperparameter defense results of classification models on Ionosphere and Iris.}
\label{clf_res_defense_other}
\end{figure*}

\section{Other Sensitivity Results}

We show the hyperparameter sensitivity results of classification models on Ionosphere in Figure~\ref{clf_res_sensi_ionosphere}.

\begin{figure*}
\center
\subfloat[BLR]{\includegraphics[width=0.24\textwidth]{./src_sensitivity/figs/clf/result-clf-lr-ionosphere.pdf}\label{lr_ionosphere_sensi}}
\subfloat[BKLR]{\includegraphics[width=0.24\textwidth]{./src_sensitivity/figs/clf/result-clf-klr-ionosphere.pdf}\label{klr_ionosphere_sensi}}
\subfloat[BLSVC]{\includegraphics[width=0.24\textwidth]{./src_sensitivity/figs/clf/result-clf-svc-ionosphere.pdf}\label{svc_ionosphere_sensi}}
\subfloat[BKSVC]{\includegraphics[width=0.24\textwidth]{./src_sensitivity/figs/clf/result-clf-ksvc-ionosphere.pdf}\label{ksvc_ionosphere_sensi}} 
\caption{Hyperparameter sensitivity results of classification models on Ionosphere.}
\label{clf_res_sensi_ionosphere}
\end{figure*}
